# Supplementary material for: HAVER: Instance-Dependent Error Bounds for Maximum Mean Estimation and Applications to Q-Learning and Monte Carlo Tree Search
Source: arXiv:2411.00405 source file (2025-04-29)
Supplement: Supplementary file 6 [file sub-appendix_v31.tex]

TODOs
\begin{itemize}
\item Haver's theorem
\item MaxLCB's theorem
  \begin{itemize}
  \item put the proof together
  \end{itemize}  
\end{itemize}

\section{Algorithm}

\begin{algorithm}[H]
  \caption{Haver Estimator}\label{algo:haver}
  \begin{algorithmic}
    \STATE{\textbf{Input:} A set of K arms with samples $\cbr{X_{i, 1:N_i}}_{i=1}^{K}$
    % with corresponding sets of empirical means $\cbr{\muhat_i}_{i=1}^K$, empirical variances $\cbr{\sigmahat_i}_{i=1}^K$, and number of arm pulls $\cbr{N_i}_{i=1}^K$
}
    \STATE{
 For each arm $i$, compute its empirical mean $\hmu_i$ and variance $\hsigma_i^2$ \\
\qquad $\hmu_i = \fr{1}{N_i}\sum_{j=1}^{N_i}X_{i,j}$, \qquad $\hsigma_i^2 = \fr{\sum_{j=1}^{N_i}\del{X_{i,j} - \hmu_i}^2}{N_i\del{N_i-1}}$ \\
 Find pivot arm $\hr$  \\
\qquad $\hr = \displaystyle \argmax_{i \in [K]} \muhat_i - \gam_{i}$ \\
\qquad where $\gam_{i} = \sqrt{\frac{18\sigmahat_i^2}{N_i}\log\del{K^{2\lambda}}}$ \\
 Form a set $\cB$ of desirable arms \\
\qquad $\cB \gets \{i \in [K]: \muhat_{i} \ge \muhat_{\hr} - \gam_{\hr} \}$ \\
 Compute the weighted average of empirical means of desirable arms in set $\cB$ \\
\qquad $\hmuB = \frac{1}{Z} \displaystyle \sum_{i \in \cB} \frac{N_i}{\sigmahat_i^2+\eps}\muhat_i$ \\
\qquad where $Z = \sum_{i \in \cB} \frac{N_i}{\sigmahat_i^2+\eps}$ \\
}
    \RETURN $\hmuB$
  \end{algorithmic}
\end{algorithm}

% Note: for now we assume that the variances are known $\sigmahat_i = \sigma_i = 1$ 

\subsection{Notations}

List of notations and definitions (todo: make it into a table)
\begin{itemize}
\item $\gam_{i} = \sqrt{\frac{18}{N_{i}}\log\del{\del{\fr{KS}{N_i}}^{2\lambda}}}$, where $S = N_{\max}\sum_{j \in [K]}N_j$
  % \begin{itemize}
  % \item in the scenario that all arm pulls are equal $\forall i \in [K],\, N_i = N$, then $\gam_i = \gam = \sqrt{\frac{18}{N}\log\del{K^{2\lambda}}}$
  % \end{itemize}
\item $\rhat = \argmax_i \hmu_i - \gam_i$
\item $s = \argmax_i \mu_i - \cs\gam_i$
\item $\cB := \cbr{i \in [K]: \hmu_{i} \ge \hmu_{\hr} - \gam_{\hr},\, \gam_{i} \le \fgam \gam_{\hr}}$
\item $\cR :=  \cbr{r \in [K]: \mu_s - \fr{4}{3}\gam_s + \fr{2}{3}\gam_r \le \mu_r \le \mu_s - \cs\gam_s + \cs\gam_r}$
\item $\cBs(r) := \cbr{i \in [K]: \mu_{i} \ge \mu_{s} - \cstar\gam_{s},\, \gam_i \le \fgam \gam_{r}}$
\item $\cBp(r) := \cbr{i: \mu_{i} \ge \mu_{s} - \cplus\gam_{s} - \cplus\gam_{i},\, \gam_i \le \fgam \gam_{r}}$
%\kj{$c_+\sqrt{\gam_s^2 + \gam_i^2}$ this might help improve const factor?}
% \item $c = c_r = 1$, $c_s = \cs$, $c_* = \cstar$, $c_+ = \cplus$, $f = \fr{4}{9}$
\end{itemize}

Throughout the paper, $c_1$ and $c_2$ are a universal and positive constant, which may have different values for different expressions. 
Both $\tilde\Theta(\cdot)$, $\tilcO(\cdot)$, and ``$\scriptscriptstyle \lsim$'' omits logarithmic factors on $K$, but not $1/\dt$. 

\section{Haver's Corollaries}


% \begin{theorem}\label{thm:haver_non_equal_arm_pulls_generic}
%   Let $s := \argmax_i \mu_i - \cs\gam_i$, $\cBs := \cbr{i \in [K]: \mu_{i} \ge \mu_{s} - \cstar \gam_{s},\, N_i \ge \finv N_{s}}$ and $\cBp := \cbr{i \in [K]: \mu_{i} \ge \mu_{s} - \sqrt{\cplus\gam_{s}^2 + \cplus\gam_{i}^2}}$. Haver's MSE is upper bounded by
%   \begin{align*}
%     \MSE
%     \stackrel{}{=}\,&\displaystyle \tilcO \del{\del{\del{\displaystyle \fr{1}{\sum_{j \in \cBs}N_j}\sum_{i \in \cBp}N_i\Delta_i}^2 + \max_{k=1}^{d(r)} \max_{\substack{S: \cBs \subseteq \cS \subseteq \cBp \\ \abs{\cS}=n^*+k }}\fr{k \sum_{j \in \cS \sm \cBs}N_j}{\del{\sum_{j \in \cS}N_j}^2} + \fr{1}{\sum_{j \in \cBs}N_j}} \wedge \del{\min_{m} \del{\fr{1}{N_m} + \Delta_m^2}} } \\
%     &+ \tilcO \del{\min_m \fr{1}{K^{\lambda}}\del{\fr{1}{N_m} + \Delta_m^2} + \max_{m}\fr{1}{K^{\lambda}N_m} }
%   \end{align*}
%   Furthermore, in the scenario that all arm pulls are equal $\forall i \in [K],\, N_i = N$, we have $\cBs$ and $\cBp$ respectively reduced to $\cBs = \cbr{i \in [K]: \Delta_i \le \cstar \gam}$, $\cBp := \cbr{i \in [K]: \Delta_i \le \cplus \gam}$, and Haver's MSE is upper bounded by
%   \begin{align*}
%     \MSE
%     \stackrel{}{=}\,& \tilcO \del{\del{\displaystyle \fr{1}{\abs{\cBs}}\sum_{i = 1}^{\abs{\cBp}}\Delta_i}^2 + \sum_{k=0}^d \fr{1}{\del{\abs{\cBs} + k}^2N}}
%   \end{align*}
% \end{theorem}
% The proof is in Appendix ~\ref{thm_proof:haver_non_equal_arm_pulls_generic}

\newtheorem*{cor-0}{Corollary ~\ref{cor:haver_equal_arm_pulls_generic}}
\begin{cor-0}
  Under the Assumption~\ref{ass:equal_arm_pulls} (equal number of samples). Let $\gam := \sqrt{\frac{18}{N}\log\del{\del{K^2N}^{2\lam}}}$ with $\lam = 2$. Let $\cBs :=\cbr{i \in [K]: \Delta_{i} \le \cstar\gam}$, $\cBp := \cbr{i \in [K]: \Delta_{i} \le \cplusq\gam}$, Haver achieves 
  \begin{align*}
    &\MSE(\hmuhaver) \\
    \stackrel{}{=}\,& \cO \del{\del{\fr{1}{\abs{\cBs}}\sum_{i = 1}^{\abs{\cBp}}\Delta_i}^2 \wedge \del{\fr{1}{N}\log\del{KS}}} \\
    &+ \cO \del{\del{\fr{1}{N}\del{\log\del{\fr{\abs{\cBp}}{\abs{\cBs}}}}^2 \log\del{3K}\log(K)} \wedge \del{\fr{1}{N}\log\del{KS}}} \\
    &+ \cO \del{\fr{1}{\abs{\cBs}N}\log\del{KS}} 
  \end{align*}
  where $d = \abs{\cBp} - \abs{\cBs}$ and $n_* = \abs{\cBs}$
\end{cor-0}

\begin{proof}
  Under the Assumption~\ref{ass:equal_arm_pulls} (equal number of samples), from Theorem~\ref{thm:haver21count2}, we have the following changes. 
  
  First, $\forall i \in [K]$,
  \begin{align*}
    \gam_i = \sqrt{\frac{18}{N_i}\log\del{\del{\fr{KN_{\max}\sum_{j \in [K]}N_j}{N_i}}^{2\lam}}} = \sqrt{\frac{18}{N}\log\del{\del{K^2N}^{2\lam}}} =: \gam 
  \end{align*}
  Second, $s = \argmax_{i} \hmu_{i} - \cs \gam_{i} = \argmax_{i} \hmu_{i} - \cs \gam = 1$
  Third, $\cBs(r)$ and $\cBp(r)$ become $\cBs$ and $\cBp$ respectively as follow:
  \begin{align*}
    \cBs(r)
    \stackrel{}{=}\,& \cbr{i \in [K]: \mu_{i} \ge \mu_{s} - \cstar\gam_{s},\, \gam_i \le \fgam \gam_{r}} \\
    \stackrel{}{=}\,& \cbr{i \in [K]: \mu_{i} \ge \mu_{1} - \cstar\gam} \\
    \stackrel{}{=}\,& \cbr{i \in [K]: \Delta_{i} \le \cstar\gam} =: \cBs
  \end{align*}
  \begin{align*}
    \cBp(r)
    \stackrel{}{=}\,& \cbr{i \in [K]: \mu_{i} \ge \mu_{s} - \cplus\gam_{s} - \cplus\gam_{i},\, \gam_i \le \fgam \gam_{r}} \\
    \stackrel{}{=}\,& \cbr{i \in [K]: \mu_{i} \ge \mu_{1} - \cplus\gam - \cplus\gam} \\
    \stackrel{}{=}\,& \cbr{i \in [K]: \Delta_{i} \le \cplusq\gam} =: \cBp,
  \end{align*}
  Additionally, $d(r) = \abs{\cBp(r)} - \abs{\cBs(r)} = \abs{\cBp} - \abs{\cBs} =: d$ and $n_*(r) = \abs{\cBs(r)} = \abs{\cBs} =: n_*$. Thus, we can safely remove the dependencies on $\cR$.
  From Theorem~\ref{thm:haver21count2}, we have 
  \begin{align*}
    &\MSE(\hmuhaver) \\
    \stackrel{}{=}\,& \cO \del{\del{\displaystyle \max_{r \in \cR} \fr{1}{\sum_{j \in \cBs(r)}N_j}\sum_{i \in \cBp(r)}N_i\Delta_i}^2 \wedge \del{\fr{1}{N_1}\log\del{KS}}} \\
    &+ \cO \del{\del{\max_{r \in \cR} \max_{k=1}^{d(r)} \max_{\substack{S: \cBs(r) \subseteq \Scal \subseteq \cBp(r) \\ \abs{\Scal}=n_*(r)+k }}\fr{k\sum_{j \in \Scal \sm \cBs(r)}N_j}{\del{\sum_{j \in \Scal}N_j}^2}\log\del{\fr{ed}{k}}\log(K)} \wedge \del{\fr{1}{N_1}\log\del{KS}}} \\
    &+ \cO\del{\del{\fr{\log(K)}{\min_{r \in \cR}\sum_{j \in \cBs(r)}N_j}} \wedge \del{\fr{1}{N_1}\log\del{KS}}} \\
    &+ \cO \del{\fr{1}{KN_1}\log\del{KS}} 
    % \stackrel{}{=}\,& \cO \del{\del{\fr{1}{\abs{\cBs}}\sum_{i = 1}^{\cBp}\Delta_i}^2 \wedge \del{\fr{1}{N}\log\del{KS}}} \\
    % &+ \cO \del{\del{\fr{d(\abs{\cBp} - \abs{\cBs})N}{\del{\abs{\cBp}N}^2} \log\del{ed}\log(K)} \wedge \del{\fr{1}{N}\log\del{KS}}} \\
    % &+ \cO\del{\del{\fr{\log(K)}{\abs{\cBs}N}} \wedge \del{\fr{1}{N}\log\del{KS}}} \\
    % &+ \cO \del{\fr{1}{KN}\log\del{KS}} \\
    % \stackrel{}{=}\,& \cO \del{\del{\fr{1}{\abs{\cBs}}\sum_{i = 1}^{\cBp}\Delta_i}^2 \wedge \del{\fr{1}{N}\log\del{KS}}} \\
    % &+ \cO \del{\fr{1}{N}\del{\fr{d^2}{\del{\abs{\cBp}}^2} \log\del{ed}\log(K)} \wedge \del{\fr{1}{N}\log\del{KS}}} \\
    % &+ \cO\del{\del{\fr{\log(K)}{\abs{\cBs}N}} \wedge \del{\fr{1}{N}\log\del{KS}}} \\
    % &+ \cO \del{\fr{1}{KN}\log\del{KS}} \\
  \end{align*}
  The first component becomes
  \begin{align*}
    \max_{r \in \cR} \fr{1}{\sum_{j \in \cBs(r)}N_j}\sum_{i \in \cBp(r)}N_i\Delta_i^2 
    \stackrel{}{=}\,& \del{\fr{1}{\abs{\cBs}}\sum_{i = 1}^{\abs{\cBp}}\Delta_i}^2
  \end{align*}
  The second component becomes
  \begin{align*}
    &\max_{r \in \cR} \max_{k=1}^{d(r)} \max_{\substack{S: \cBs(r) \subseteq \Scal \subseteq \cBp(r) \\ \abs{\Scal}=n_*(r)+k }}\fr{k\sum_{j \in \Scal \sm \cBs(r)}N_j}{\del{\sum_{j \in \Scal}N_j}^2}\log\del{\fr{ed}{k}}\log(K) \\
    \stackrel{}{=}\,& \max_{k=1}^{d} \fr{k^2N}{\del{(n^*+k)N}^2}\log\del{\fr{ed}{k}}\log(K) \\
    \stackrel{}{=}\,& \max_{k=1}^{d} \fr{k^2}{\del{n^*+k}^2N}\log\del{\fr{ed}{k}}\log(K) \\
    \stackrel{}{\le}\,& \max_{k=1}^{d} \fr{k^2}{\del{n^*+k}^2N}\log\del{3K}\log(K) \\
    \stackrel{}{\le}\,& \fr{1}{N}\del{\log\del{\fr{n^*+d}{n^*}}}^2 \log\del{3K}\log(K) \tagcmt{use Lemma~\ref{xlemma:max_bound}} \\
    \stackrel{}{=}\,& \fr{1}{N}\del{\log\del{\fr{\abs{\cBp}}{\abs{\cBs}}}}^2 \log\del{3K}\log(K)
  \end{align*}
  The third component becomes
  \begin{align*}
    \fr{\log(K)}{\min_{r \in \cR}\sum_{j \in \cBs(r)}N_j} = \fr{\log(K)}{\abs{\cBs}N} 
  \end{align*}
  Thus, we have
  \begin{align*}
    &\MSE(\hmuhaver) \\
    \stackrel{}{=}\,& \cO \del{\del{\fr{1}{\abs{\cBs}}\sum_{i = 1}^{\abs{\cBp}}\Delta_i}^2 \wedge \del{\fr{1}{N}\log\del{KS}}} \\
    &+ \cO \del{\del{\fr{1}{N}\del{\log\del{\fr{\abs{\cBp}}{\abs{\cBs}}}}^2 \log\del{3K}\log(K)} \wedge \del{\fr{1}{N}\log\del{KS}}} \\
    &+ \cO\del{\del{\fr{\log(K)}{\abs{\cBs}N} } \wedge \del{\fr{1}{N}\log\del{KS}}} \\
    &+ \cO \del{\fr{1}{KN}\log\del{KS}} \\
    \stackrel{}{=}\,& \cO \del{\del{\fr{1}{\abs{\cBs}}\sum_{i = 1}^{\abs{\cBp}}\Delta_i}^2 \wedge \del{\fr{1}{N}\log\del{KS}}} \\
    &+ \cO \del{\del{\fr{1}{N}\del{\log\del{\fr{\abs{\cBp}}{\abs{\cBs}}}}^2 \log\del{3K}\log(K)} \wedge \del{\fr{1}{N}\log\del{KS}}} \\
    &+ \cO \del{\fr{1}{\abs{\cBs}N}\log\del{KS}} \\
    % \stackrel{}{=}\,& \cO \del{\del{\del{\fr{1}{\abs{\cBs}}\sum_{i = 1}^{\abs{\cBp}}\Delta_i}^2 + \fr{1}{N}\del{\log\del{\fr{\abs{\cBp}}{\abs{\cBs}}}}^2 \log\del{3K}\log(K)  + \fr{\log(K)}{\abs{\cBs}N}} \wedge \del{\fr{1}{N}\log\del{KS}}} 
  \end{align*}
\end{proof}

\newtheorem*{cor-1}{Corollary ~\ref{cor:haver_equal_arm_pulls_all_best}}
\begin{cor-1}
  Under the Assumption~\ref{ass:equal_arm_pulls} (equal number of samples). Consider the all-best instance where $\forall i \in [K], \mu_i = \mu_1$, Haver achieves
  \begin{align*}
    \MSE(\hmuhaver) = \cO \del{\fr{1}{KN}\log\del{KS}}
  \end{align*}
\end{cor-1}

\begin{proof}
  From Corollary \ref{cor:haver_equal_arm_pulls_generic}, we set $\Bcals = \cbr{i \in [K]: \Delta_i \le \cstar \gam}$ and $\Bcalp := \cbr{i \in [K]: \Delta_i \le \cplusq \gam}$, $d = \abs{\Bcalp} - \abs{\Bcals}$.
  For the all-best instance, we can see that $\Bcals = [K]$, $\Bcalp = [K]$, $d = 0$.
  
  Therefore, from Corollary \ref{cor:haver_equal_arm_pulls_generic}, the bias squared term $\displaystyle \fr{1}{\abs{\Bcals}}\sum_{i = 1}^{\abs{\Bcalp}}\Delta_i$ becomes 0 since $\forall i \in \Bcalp = [K],\, \Delta_i = 0$. Also, the variance term $\fr{1}{N}\del{\log\del{\fr{\abs{\Bcalp}}{\abs{\Bcals}}}}^2 = 0$ since $\log\del{\fr{\abs{\Bcalp}}{\abs{\Bcals}}} = 0$. Also, $\fr{1}{\abs{\Bcals}N} = \fr{1}{KN}$.

  Therefore, Haver achieves
  \begin{align*}
    \MSE(\hmuhaver) = \cO \del{\fr{1}{KN}\log\del{KS}}.
  \end{align*}
  
\end{proof}

\newtheorem*{cor-2}{Corollary ~\ref{cor:haver_equal_arm_pulls_kstar_best}}
\begin{cor-2}
  Under the Assumption~\ref{ass:equal_arm_pulls} (equal number of samples). Consider the $\Kstar$-best instance where $\forall i \in [\Kstar],\, \mu_i = \mu_1$. With an assumption $N > \fr{4}{\Delta_{\Kstar+1}^2}\log\del{K^{6}}$, Haver achieves
  \begin{align*}
    \MSE(\hmuhaver) = \cO \del{\fr{1}{\Kstar N}\log(KS)}.
  \end{align*}
\end{cor-2}

\begin{proof}
  From Corollary \ref{cor:haver_equal_arm_pulls_generic}, we set $\Bcals = \cbr{i \in [K]: \Delta_i \le \cstar \gam}$ and $\Bcalp := \cbr{i \in [K]: \Delta_i \le \cplusq \gam}$.
  The assumption $N > \fr{81}{32\Delta_{\Kstar+1}^2}\log\del{K^{6}}$ implies that $\Delta_{\Kstar+1} > \fr{8}{3}\sqrt{\fr{18}{N}\log\del{K^{6}}} = \cplusq\gam$, thereby implies that $\forall i \ge \Kstar+1, \Delta_i \ge \Delta_{\Kstar+1} > \cplusq\gam$. Therefore, we have $\Bcals = [\Kstar]$, $\Bcalp = [\Kstar]$, $d = 0$.

  Therefore, from Corollary \ref{cor:haver_equal_arm_pulls_generic}, the bias squared term $\displaystyle \fr{1}{\abs{\Bcals}}\sum_{i = 1}^{\abs{\Bcalp}}\Delta_i$ becomes 0 since $\forall i \in \Bcalp = [\Kstar],\, \Delta_i = 0$. Also, the variance term $\fr{1}{N}\del{\log\del{\fr{\abs{\Bcalp}}{\abs{\Bcals}}}}^2 = 0$ since $\log\del{\fr{\abs{\Bcalp}}{\abs{\Bcals}}} = 0$. Also, $\fr{1}{\abs{\Bcals}N} = \fr{1}{\Kstar N}$.

  Therefore, Haver's MSE is upper bounded by
  \begin{align*}
    \MSE(\hmuhaver) = \cO \del{\fr{1}{\Kstar N}\log(KS)}.
  \end{align*}
  
\end{proof}

\newtheorem*{cor-3}{Corollary ~\ref{cor:haver_equal_arm_pulls_alpha_poly}}
\begin{cor-3}
  Under the Assumption~\ref{ass:equal_arm_pulls} (equal number of samples). Consider the Poly($\alpha$) instance where $\forall i \ge 2,\, \Delta_i = \del{\fr{i}{K}}^{\alpha}$ and $\alpha \ge 2$. With an assumption that $N$ is not too large $N \le \fr{1}{64}\del{K\fr{\ln(2)}{\alpha}}^{2\alpha}$, Haver achieves
  \begin{align*}
    \MSE(\hmuhaver) = \cO \del{\fr{1}{\alpha^2N}\log(3K)\log(K) + \fr{1}{\abs{\cBs}N}\log\del{KS}}.
    % \MSE = \tilcO \del{\fr{1}{\alpha^2N} \wedge \fr{1}{N}}
  \end{align*}
\end{cor-3}

\begin{proof}
  From Corollary \ref{cor:haver_equal_arm_pulls_generic}, we set $\Bcals = \cbr{i \in [K]: \Delta_i \le \cstar \gam}$ and $\Bcalp := \cbr{i \in [K]: \Delta_i \le \cplusq \gam}$, and
  \begin{align*}
    &\MSE(\hmuhaver) \\
    \stackrel{}{=}\,& \cO \del{\del{\fr{1}{\abs{\cBs}}\sum_{i = 1}^{\abs{\cBp}}\Delta_i}^2 \wedge \del{\fr{1}{N}\log\del{KS}}} \\
    &+ \cO \del{\del{\fr{1}{N}\del{\log\del{\fr{\abs{\cBp}}{\abs{\cBs}}}}^2 \log\del{3K}\log(K)} \wedge \del{\fr{1}{N}\log\del{KS}}} \\
    &+ \cO \del{\fr{1}{\abs{\cBs}N}\log\del{KS}} 
  \end{align*}
  
  % That means, there exists a constant $\til c \ge 0$ ($\til c$ omits log factor in $K$) such that
  % \begin{align*}
  %   \MSE
  %   \stackrel{}{=}\,& \til c \del{\del{\del{\displaystyle \fr{1}{\abs{\Bcals}}\sum_{i = 1}^{\abs{\Bcalp}}\Delta_i}^2 + \fr{1}{N}\del{\log\del{\fr{\abs{\Bcalp}}{\abs{\Bcals}}}}^2 + \fr{1}{\abs{\Bcals}N}} \wedge \fr{1}{N} + \fr{1}{KN}}.
  % \end{align*}
  
  For the first term, we use Lemma~\ref{lemma304:bcals} with $a_1=6$ and $a_2=\cplusq$ to bound
  \begin{align*}
    &\del{\displaystyle \fr{1}{\abs{\Bcals}}\sum_{i = 1}^{\abs{\Bcalp}}\Delta_i}^2 \\
    \stackrel{}{\le}\,& \del{\fr{a_2\del{2a_1a_2}^{\fr{1}{\alpha}}}{\del{\alpha+1}\sqrt{N}}}^2 \\
    \stackrel{}{\le}\,& \del{\fr{2\del{32}^{\fr{1}{\alpha}}}{\del{\alpha+1}\sqrt{N}}}^2 \\
    \stackrel{}{=}\,& \fr{4\del{32}^{\fr{2}{\alpha}}}{\del{\alpha+1}^2N}.
  \end{align*}

  For the second term, we use Lemma~\ref{lemma303:bcals} with $a_1=6$ and $a_2=\cplusq$ to bound 
  \begin{align*}
    \fr{\abs{\Bcalp}}{\abs{\Bcals}} \le \del{2a_1a_2}^{\fr{1}{\alpha}} = 32^{\fr{1}{\alpha}}.
  \end{align*}
  Hence,
  \begin{align*}
    \fr{1}{N}\del{\log\del{\fr{\abs{\Bcalp}}{\abs{\Bcals}}}}^2 \le \fr{1}{N}\del{\log\del{32^{\fr{1}{\alpha}}}}^2 = \fr{1}{\alpha^2N}\log^2(32)
  \end{align*}
  For the third term, we use Lemma~\ref{lemma303:bcals} with $a_1=6$ and $a_2=\cplusq$ to bound
  \begin{align*}
    \fr{1}{\abs{\cBs}} \le \fr{1}{K\del{\fr{1}{12}\sqrt{\fr{1}{N}}}^{\fr{1}{\alpha}}}
  \end{align*}

Combining these two terms, Haver's MSE is upper bounded by
\begin{align*}
  &\MSE(\hmuhaver) \\
  \stackrel{}{=}\,& \cO \del{\del{\fr{1}{\abs{\cBs}}\sum_{i = 1}^{\abs{\cBp}}\Delta_i}^2 \wedge \del{\fr{1}{N}\log\del{KS}}} \\
  &+ \cO \del{\del{\fr{1}{N}\del{\log\del{\fr{\abs{\cBp}}{\abs{\cBs}}}}^2 \log\del{3K}\log(K)} \wedge \del{\fr{1}{N}\log\del{KS}}} \\
  &+ \cO \del{\fr{1}{NK\del{\fr{1}{12}\sqrt{\fr{1}{N}}}^{\fr{1}{\alpha}}}\log\del{KS}} \\
  \stackrel{}{=}\,& \cO \del{\fr{4\del{32}^{\fr{2}{\alpha}}}{\del{\alpha+1}^2N} \wedge \del{\fr{1}{N}\log\del{KS}}} \\
  &+ \cO \del{\fr{1}{\alpha^2N}\log^2(32) \wedge \del{\fr{1}{N}\log\del{KS}}} \\
  &+ \cO \del{\fr{1}{NK\del{\fr{1}{12}\sqrt{\fr{1}{N}}}^{\fr{1}{\alpha}}}\log\del{KS}} \\
  \stackrel{}{=}\,& \cO \del{\del{\fr{\del{32}^{\fr{2}{\alpha}}}{\del{\alpha+1}^2N} + \fr{1}{\alpha^2N}\log(3K)\log(K)} \wedge \del{\fr{1}{N}\log\del{KS}} + \fr{1}{NK\del{\fr{1}{12}\sqrt{\fr{1}{N}}}^{\fr{1}{\alpha}}}\log\del{KS}}
  % &+ \cO \del{\fr{1}{\abs{\cBs}N}\log\del{KS}} \\
  %   \stackrel{}{=}\,& \cO \del{\del{\del{\displaystyle \fr{1}{\abs{\Bcals}}\sum_{i = 1}^{\abs{\Bcalp}}\Delta_i}^2 + \fr{1}{N}\del{\log\del{\fr{\abs{\Bcalp}}{\abs{\Bcals}}}}^2 + \fr{1}{\abs{\Bcals}N}} \wedge \fr{1}{N} + \fr{1}{KN}} \\
  % \stackrel{}{\le}\,& \cO \del{\del{\fr{4\del{8}^{\fr{2}{\alpha}}}{\del{\alpha+1}^2N} + \fr{1}{\alpha^2N}\log^2{8} + \fr{1}{\abs{\Bcals}N}} \wedge \fr{1}{N} + \fr{1}{KN}}.
\end{align*}

% There are two cases: (1) $\alpha < 1$ and (2) $\alpha \ge 1$

% Case 1: $\alpha \in (0, 1)$, then
% \begin{align*}
%   & \cO \del{\del{\fr{\del{32}^{\fr{2}{\alpha}}}{\del{\alpha+1}^2N} + \fr{1}{\alpha^2N}\log(3K)\log(K)} \wedge \del{\fr{1}{N}\log\del{KS}} + \fr{1}{NK\del{\fr{1}{12}\sqrt{\fr{1}{N}}}^{\fr{1}{\alpha}}}\log\del{KS}} \\
%   \stackrel{}{=}\,& \cO \del{\fr{1}{N}\log\del{KS} + \fr{1}{NK\del{\fr{1}{12}\sqrt{\fr{1}{N}}}^{\fr{1}{\alpha}}}\log\del{KS}} \\
%   \stackrel{}{=}\,& \cO \del{\fr{1}{N}\log\del{KS}}.
% \end{align*}

In the case of $\alpha > 2$, we have 
\begin{align*}
  & \cO \del{\del{\fr{\del{32}^{\fr{2}{\alpha}}}{\del{\alpha+1}^2N} + \fr{1}{\alpha^2N}\log(3K)\log(K)} \wedge \del{\fr{1}{N}\log\del{KS}} + \fr{1}{\abs{\cBs}N}\log\del{KS}} \\
  \stackrel{}{\le}\,& \cO \del{\fr{1}{\alpha^2N}\log(3K)\log(K) + \fr{1}{\abs{\cBs}N}\log\del{KS}}.
\end{align*}

% Case 1: $\alpha < 1$, then
% \begin{align*}
%   & \til c \del{\del{\fr{4\del{8}^{\fr{2}{\alpha}}}{\del{\alpha+1}^2N} + \fr{1}{\alpha^2N}\log^2{8} + \fr{1}{\abs{\Bcals}N}} \wedge \fr{1}{N} + \fr{1}{KN}} \\
%   \stackrel{}{\le}\,& \til c \del{\fr{1}{N} + \fr{1}{KN}} \\
%   \stackrel{}{\le}\,& \til c \del{\fr{1}{N}}.
% \end{align*}

% Case 2: $\alpha > 2$, then
% \begin{align*}
%   & \til c \del{\del{\fr{4\del{8}^{\fr{2}{\alpha}}}{\del{\alpha+1}^2N} + \fr{1}{\alpha^2N}\log^2{8} + \fr{1}{\abs{\Bcals}N}} \wedge \fr{1}{N} + \fr{1}{KN}} \\
%   \stackrel{}{\le}\,& \til c \del{\fr{1}{\alpha^2N}}.
% \end{align*}

\end{proof}

\newtheorem*{cor-4}{Corollary ~\ref{cor:haver_non_equal_arm_pulls_allbest}}
\begin{cor-4}
  Consider the all-best instance where $\forall i \in [K],\, \mu_i = \mu_{1}$ and the number of samples are characterized by $N_i = \del{K - i + 1}^{\alpha}$ where $\alpha$.  Haver achieves
  \begin{align*}
    \MSE(\hmuhaver) = \cO \del{\fr{\log(KS)}{N_1\del{\fr{K}{\alpha+1}\del{1 - \del{\fr{4}{9}^{\fr{\alpha+1}{\alpha}}}} + 1}}}.
    % \MSE = \tilcO \del{\fr{1}{\alpha^2N} \wedge \fr{1}{N}}
  \end{align*}
\end{cor-4}

\begin{proof}
  In the all-best instance, all arms have equal mean and since the number of samples are decreasing, thus $s = \argmax_{i \in [K]} \mu_i \cs \gam_i = 1$.
  From Theorem~\ref{thm:haver21count2}, we set
  \begin{align*}
    \cBs(r) =\cbr{i \in [K]: \mu_{i} \ge \mu_{s} - \cstar\gam_{s},\, \gam_i \le \fgam \gam_{r}}
  \end{align*}
  and
  \begin{align*}
    \cBp(r) := \cbr{i: \mu_{i} \ge \mu_{s} - \cplus\gam_{s} - \cplus\gam_{i},\, \gam_i \le \fgam \gam_{r}}
  \end{align*}
  In the all-best instance, for every $r \in \cR$, the first condition of $\cBs(r)$, $\mu_i \ge \mu_{s} - \cstar\gam_i$ is always satisfied and the first condition of $\cBp(r)$, $\mu_i \ge \mu_{s} - \cplus\gam_s - \cplus\gam_i$, is always satisfied. Also the second conditions of both $\cBs(r)$ and $\cBp(r)$ is the same. Thus, we have $\forall r \in \cR,\, \cBp(r) = \cBs(r)$.

  From Theorem~\ref{thm:haver21count2}, we have
  \begin{align*}
    &\MSE(\hmuhaver) \\
    \stackrel{}{=}\,& \cO \del{\del{\displaystyle \max_{r \in \cR} \fr{1}{\sum_{j \in \cBs(r)}N_j}\sum_{i \in \cBp(r)}N_i\Delta_i}^2 \wedge \del{\fr{1}{N_1}\log\del{KS}}} \\
    &+ \cO \del{\del{\max_{r \in \cR} \max_{k=0}^d \max_{\substack{S: \cBs(r) \subset \Scal \subseteq \cBp(r) \\ \abs{\Scal}=n_*+k }}\fr{k\sum_{j \in \Scal \sm \cBs(r)}N_j}{\del{\sum_{j \in \Scal}N_j}^2}\log\del{\fr{ed}{k}}\log(K)} \wedge \del{\fr{1}{N_1}\log\del{KS}}} \\
    &+ \cO\del{\del{\fr{\log(K)}{\min_{r \in \cR}\sum_{j \in \cBs(r)}N_j}} \wedge \del{\fr{1}{N_1}\log\del{KS}}} \\
    &+ \cO \del{\fr{1}{KN_1}\log\del{KS}}.
  \end{align*}

  For the first term, $\del{\displaystyle \max_{r \in \cR} \fr{1}{\sum_{j \in \cBs(r)}N_j}\sum_{i \in \cBp(r)}N_i\Delta_i}^2$ becomes $0$ since $\forall i \in [K],\, \Delta_i = 0$.
  
  For the second term, $\del{\max_{r \in \cR} \max_{k=0}^d \max_{\substack{S: \cBs(r) \subset \Scal \subseteq \cBp(r) \\ \abs{\Scal}=n_*+k }}\fr{k\sum_{j \in \Scal \sm \cBs(r)}N_j}{\del{\sum_{j \in \Scal}N_j}^2}\log\del{\fr{ed}{k}}\log(K)}$ becomes $0$ since $\forall r \in \cR,\, \cBp(r) = \cBs(r)$.

  For the third term, we have 
  \begin{align*}
    \fr{\log(K)}{\min_{r \in \cR}\sum_{j \in \cBs(r)}N_j} = \fr{\log(K)}{\sum_{j \in \cBs(1)}N_j} 
  \end{align*}
  $r = 1$ results in minimal number of arms in $\cBs(r)$ because (1) the optimal arm $1$ is always in $\cR$ and (2) among arm $r \in \cR$, arm $r = 1$ has the highest number of samples making the condition $\gam_i \le \fgam \gam_r$ most restrictive.
  An arm $i$ is included in $\cBs(1)$ if it satisfies
  \begin{align*}
    &\gam_i \le \fgam \gam_1 \\
    \stackrel{}{\Leftrightarrow}\,& \fr{18}{N_i}\log\del{\del{\fr{KS}{N_i}}^{2\lam}} \le \fr{9}{4}\fr{18}{N_1}\log\del{\del{\fr{KS}{N_1}}^{2\lam}} \\
    \stackrel{}{\Leftrightarrow}\,& \fr{1}{N_i}\log\del{\fr{KS}{N_i}} \le \fr{9}{4}\fr{1}{N_1}\log\del{\fr{KS}{N_1}} \\
    \stackrel{}{\Leftrightarrow}\,& N_i \ge \fr{4}{9}N_1 \fr{\log\del{\fr{KS}{N_i}}}{\log\del{\fr{KS}{N_1}}} \\
    \stackrel{}{\Rightarrow}\,& N_i \ge \fr{4}{9}N_1 \tagcmt{use $N_i \le N_1$} \\
    \stackrel{}{\Leftrightarrow}\,& \del{K-i+1}^{\alpha} \ge \fr{4}{9}K^{\alpha} \\
    \stackrel{}{\Leftrightarrow}\,& K-i+1 \ge \del{\fr{4}{9}}^{\fr{1}{\alpha}}K \\
    \stackrel{}{\Leftrightarrow}\,& i \le K\del{1 - \del{\fr{4}{9}}^{\fr{1}{\alpha}}}+1 \\
  \end{align*}
  Then, we have
  \begin{align*}
    \fr{1}{\sum_{j \in \cBs(1)}N_j} 
    \stackrel{}{\le}\,& \fr{1}{\sum_{j = 1}^{K\del{1 - \del{\fr{4}{9}}^{\fr{1}{\alpha}}}+1}N_j} 
    % \stackrel{}{\le}\,& \fr{1}{\sum_{j \in 1}^{K\del{1 - \del{\fr{4}{9}}^{\fr{1}{\alpha}}}+1}N_j} \\
  \end{align*}
  We set $\beta = 1 - \del{\fr{4}{9}}^{\fr{1}{\alpha}}$ (or $\alpha = \fr{\log\del{\fr{4}{9}}}{\log\del{1-\beta}}$), we have 
  \begin{align*}
    &\fr{1}{\sum_{j = 1}^{K\del{1 - \del{\fr{4}{9}}^{\fr{1}{\alpha}}}+1}N_j} \\
    \stackrel{}{=}\,& \fr{1}{\sum_{j = 1}^{\beta K+1}N_j} \\
    \stackrel{}{=}\,& \fr{1}{\sum_{j = 1}^{\beta K+1}(K-j+1)^{\alpha}} \\
    \stackrel{}{\le}\,& \fr{1}{\int_{j = 0}^{\beta K+1}(K-j+1)^{\alpha} \dif j} 
  \end{align*}
  We do change of variables of the integral. Let $u = K-j+1$, then $\dif u = -\dif j$. When $j = 0$, $u = K+1$. When $u = \beta K$, $u = K - \beta K$. The integral becomes
  \begin{align*}
    &\int_{j = 0}^{\beta K+1}(K-j+1)^{\alpha} \dif j \\
    \stackrel{}{=}\,& \int_{j = K+1}^{K - \beta K} -u^{\alpha} \dif u \\
    \stackrel{}{=}\,& \int_{j = K - \beta K}^{K+1} u^{\alpha} \dif u \\
    \stackrel{}{=}\,& \del{\fr{u^{\alpha+1}}{\alpha+1}}\Big|_{K - \beta K}^{K+1} \\
    \stackrel{}{=}\,& \fr{\del{K+1}^{\alpha+1} - \del{K - \beta K}^{\alpha+1}}{\alpha+1} \\
    \stackrel{}{=}\,& \fr{\del{K+1}^{\alpha+1} - K^{\alpha+1}\del{1 - \beta}^{\alpha+1}}{\alpha+1} \\
    \stackrel{}{=}\,& \fr{\del{K+1}^{\alpha+1} - K^{\alpha+1}\del{\fr{4}{9}^{\fr{1}{\alpha}}}^{\alpha+1}}{\alpha+1} \\
    \stackrel{}{=}\,& \fr{\del{K+1}^{\alpha+1} - K^{\alpha+1}\del{\fr{4}{9}^{\fr{\alpha+1}{\alpha}}}}{\alpha+1} \\
    \stackrel{}{\ge}\,& \fr{K^{\alpha+1} + (\alpha+1)K^{\alpha+1} - K^{\alpha+1}\del{\fr{4}{9}^{\fr{\alpha+1}{\alpha}}}}{\alpha+1} \\
    \stackrel{}{=}\,& \fr{K^{\alpha+1}\del{1 - \del{\fr{4}{9}^{\fr{\alpha+1}{\alpha}}}} + (\alpha+1)K^{\alpha}}{\alpha+1} \\
    \stackrel{}{=}\,& \fr{K^{\alpha}\del{K\del{1 - \del{\fr{4}{9}^{\fr{\alpha+1}{\alpha}}}} + (\alpha+1)}}{\alpha+1} 
    % \stackrel{}{=}\,& \fr{K^{\alpha+1}\del{ 1 - (1-\beta)^{\alpha+1}}}{\alpha+1} \\
  \end{align*}
  Thus,
  \begin{align*}
    &\fr{1}{\sum_{j = 1}^{K\del{1 - \del{\fr{4}{9}}^{\fr{1}{\alpha}}}+1}N_j}  \\
    \stackrel{}{\le}\,& \fr{\alpha+1}{K^{\alpha}\del{K\del{1 - \del{\fr{4}{9}^{\fr{\alpha+1}{\alpha}}}} + (\alpha+1)}} \\
    \stackrel{}{=}\,& \fr{1}{K^{\alpha}\del{\fr{K}{\alpha+1}\del{1 - \del{\fr{4}{9}^{\fr{\alpha+1}{\alpha}}}} + 1}} 
  \end{align*}
  Therefore, for the third term, we have 
  \begin{align*}
    &\fr{\log(K)}{\min_{r \in \cR}\sum_{j \in \cBs(r)}N_j} \\
    \stackrel{}{=}\,& \fr{\log(K)}{\sum_{j \in \cBs(1)}N_j} \\
    \stackrel{}{\le}\,& \fr{\log(K)}{K^{\alpha}\del{\fr{K}{\alpha+1}\del{1 - \del{\fr{4}{9}^{\fr{\alpha+1}{\alpha}}}} + 1}} \\
    \stackrel{}{=}\,& \fr{\log(K)}{N_1\del{\fr{K}{\alpha+1}\del{1 - \del{\fr{4}{9}^{\fr{\alpha+1}{\alpha}}}} + 1}} \tagcmt{use $N_1 = \del{K}^{\alpha}$}
  \end{align*}
\end{proof}


\clearpage
\section{Haver's Theorem ~\ref{thm:haver21count2}}
\label{thm_proof:haver21count2}

\kj{note: start reading from here.}

Recall the definitions that would be used in Haver 
$\gam_{i} = \sqrt{\frac{18}{N_{i}}\log\del{\del{\fr{KS}{N_i}}^{2\lambda}}}$, where $S = \kjblue{N_{\max}}\sum_{j \in [K]}N_j$

$\hr = \argmax_i \hmu_i - \gam_i$

$s = \argmax_i \mu_i - \cs\gam_i$

$\cB := \cbr{i \in [K]: \hmu_{i} \ge \hmu_{\hr} - \gam_{\hr},\, \gam_{i} \le \fgam \gam_{\hr}}$

$\cR :=  \cbr{r \in [K]: \mu_s - \fr{4}{3}\gam_s + \fr{2}{3}\gam_r \le \mu_r \le \mu_s - \cs\gam_s + \cs\gam_r}$

$\cBs(r) := \cbr{i \in [K]: \mu_{i} \ge \mu_{s} - \cstar\gam_{s},\, \gam_i \le \fgam \gam_{r}}$

$\cBp(r) := \cbr{i: \mu_{i} \ge \mu_{s} - \cplus\gam_{s} - \cplus\gam_{i},\, \gam_i \le \fgam \gam_{r}}$

\newtheorem*{thm-1}{Theorem ~\ref{thm:haver21count2}}
\begin{thm-1}
  Haver achieves
  \begin{align*}
    &\MSE(\hmuhaver) \\
    \stackrel{}{=}\,& \tilcO \del{\del{\displaystyle \max_{r \in \cR} \fr{1}{\sum_{j \in \cBs(r)}N_j}\sum_{i \in \cBp(r)}N_i\Delta_i}^2 \wedge \del{\fr{1}{N_1}}} \\
    &+ \tilcO \del{\del{\max_{r \in \cR} \max_{k=1}^{d(r)} \max_{\substack{S: \cBs(r) \subseteq \Scal \subseteq \cBp(r) \\ \abs{\Scal}=n_*(r)+k }}\fr{k\sum_{j \in \Scal \sm \cBs(r)}N_j}{\del{\sum_{j \in \Scal}N_j}^2}} \wedge \del{\fr{1}{N_1}}} \\
    &+ \tilcO \del{\del{\fr{1}{\min_{r \in \cR}\sum_{j \in \cBs(r)}N_j}} \wedge \del{\fr{1}{N_1}}} \\
    &+ \tilcO \del{\fr{1}{KN_1}}
  \end{align*}
  where $d(r) = \abs{\cBp(r)} - \abs{\cBs(r)}$ and $n_*(r) = \abs{\cBs(r)}$
\end{thm-1}

\begin{proof}
  We have
  \begin{align*}
    &\MSE(\hmuhaver) \\
    \stackrel{}{=}\,& \EE\sbr{\del{\hmuB - \mu_1}^2} \\
    \stackrel{}{=}\,& \int_{0}^{\infty} \PP\del{ \del{\hmuB - \mu_1}^2 > \eps }  \dif \eps  \\
    \stackrel{}{=}\,& \int_{0}^{\infty} \PP\del{ \abs{\hmuB - \mu_1} > \eps } \difeps \tagcmt{change of variable} \\
    \stackrel{}{=}\,& \int_{0}^{\infty} \PP\del{ \abs{\hmuB - \mu_1} < \eps,\, \exists i,\, \abs{\hmu_i - \mu_i} \ge \qgam \gam_i} \difeps \\
    &+ \int_{0}^{\infty} \PP\del{ \abs{\hmuB - \mu_1} < \eps,\, \forall i,\, \abs{\hmu_i - \mu_i} < \qgam \gam_i} \difeps
  \end{align*}
  For the first term, we use Lemma~\ref{lemma200.a:haver21count2} to obtain
  \begin{align*}
    \int_{0}^{\infty} \PP\del{ \abs{\hmuB - \mu_1} < \eps,\, \exists i,\, \abs{\hmu_i - \mu_i} \ge \qgam \gam_i} \difeps \le \tilcO \del{\fr{1}{KN_1}}
  \end{align*}

  For the second term, the condition $(a)$ $\forall i,\, \abs{\hmu_i - \mu_i} < \qgam \gam_i$ implies that $\hr \in \cR$. We prove this claim as follows. By the definition of $\hr$, we have
  \begin{align*}
    &\hmu_{\hr} - \hmu_s \ge \gam_{\hr} - \gam_{s} \\
    \stackrel{}{\Rightarrow}\,& \mu_{\hr} + \qgam \gam_{\hr} - \mu_{s} + \qgam \gam_{s} \ge \gam_{\hr} - \gam_{s} \tagcmt{use the condition $(a)$} \\
    \stackrel{}{\Leftrightarrow}\,& \mu_{\hr} \ge \mu_s + \fr{2}{3}\gam_{\hr} - \fr{4}{3}\gam_{s} 
  \end{align*}
  In addition, by definition of $s$, we have
  \begin{align*}
    \mu_{\hr} \le \mu_{s} - \cs\gam_{s} + \cs\gam_{\hr}
  \end{align*}
  These conditions imply that $\hr \in \cR$
  % the set $\cR = \cbr{r \in [K],\, \mu_s + \fr{2}{3}\gam_{r} - \fr{4}{3}\gam_{s} \le \mu_{r} \le \mu_{s} - \cs\gam_{s} + \cs\gam_{r}}$ is statistically plausible set of $\hr$
  % Also, we have $s \in \cR$ so $\cR$ is non-empty.
  % From here on, we assume the condition $\forall i,\, \abs{\hmu_i - \mu_i} < \qgam \gam_i$ unless it states otherwise.

  With $\hr \in \cR$, we decompose the second term 
  \begin{align*}
    &\int_{0}^{\infty} \PP\del{ \abs{\hmuB - \mu_1} < \eps, \hr \in \cR} \difeps \\
    \stackrel{}{=}\,& \int_{0}^{\infty} \PP\del{ \hmuB - \mu_1 < -\eps,\, \hr \in \cR} \difeps \\
    &+ \int_{0}^{\infty} \PP\del{ \hmuB - \mu_1 > \eps,\, \hr \in \cR} \difeps
  \end{align*}
  For the first subterm, we use Lemma~\ref{lemma_ga:haver21count2} to obtain
  \begin{align*}
    &\int_{0}^{\infty} \PP\del{ \hmuB - \mu_1 < -\eps,\, \hr \in \cR} \difeps \\
    \stackrel{}{=}\,& \tilcO \del{\del{\displaystyle \max_{r \in \cR} \fr{1}{\sum_{j \in \cBs(r)}N_j}\sum_{i \in \cBp(r)}N_i\Delta_i}^2 \wedge \del{\fr{1}{N_1}}} \\
    &+ \tilcO \del{\del{\max_{r \in \cR} \max_{k=1}^{d(r)} \max_{\substack{S: \cBs(r) \subseteq \Scal \subseteq \cBp(r) \\ \abs{\Scal}=n_*(r)+k }}\fr{k\sum_{j \in \Scal \sm \cBs(r)}N_j}{\del{\sum_{j \in \Scal}N_j}^2}} \wedge \del{\fr{1}{N_1}}} \\
    &+ \tilcO\del{\del{\fr{1}{\min_{r \in \cR}\sum_{j \in \cBs(r)}N_j}} \wedge \del{\fr{1}{N_1}}} \\
    &+ \tilcO \del{\fr{1}{KN_1}}
  \end{align*}
  For the second subterm, we use Lemma~\ref{lemma_gb:haver21count2} to obtain
  \begin{align*}
    &\int_{0}^{\infty} \PP\del{ \hmuB - \mu_1 > \eps,\, \hr \in \cR} \difeps \\
    \stackrel{}{\le}\,& \tilcO \del{\del{\max_{r \in \cR} \max_{k=1}^{d(r)} \max_{\substack{S: \cBs(r) \subseteq \Scal \subseteq \cBp(r) \\ \abs{\Scal}=n_*(r)+k }}\fr{k\sum_{j \in \Scal \sm \cBs(r)}N_j}{\del{\sum_{j \in \Scal}N_j}^2}} \wedge \del{\fr{1}{N_1}}} \\
    &+ \tilcO \del{\del{\fr{\log(K)}{\min_{r \in \cR}\sum_{j \in \cBs(r)}N_j}} \wedge \del{\fr{1}{N_1}}}  \\
    &+ \tilcO \del{\fr{1}{KN_1}}
    % \stackrel{}{\le}\,& \tilcO \del{\del{\max_{r \in \cR} \max_{k=1}^{d(r)} \max_{\substack{S: \cBs(r) \subset \Scal \subseteq \cBp(r) \\ \abs{\Scal}=n_*(r)+k }}\fr{k\sum_{j \in \Scal \sm \cBs(r)}N_j}{\del{\sum_{j \in \Scal}N_j}^2}\log\del{\fr{ed}{k}}\log(K) + \fr{\log(K)}{\min_{r \in \cR}\sum_{j \in \cBs(r)}N_j}} \wedge \del{\fr{1}{N_1}\log\del{KS}}} \\
    % &+ \tilcO \del{\fr{1}{KN_1}\log\del{KS}}
  \end{align*}
  Combining these two subterms, we have
  \begin{align*}
    &\int_{0}^{\infty} \PP\del{ \abs{\hmuB - \mu_1} < \eps, \hr \in \cR} \difeps \\
    \stackrel{}{=}\,& \int_{0}^{\infty} \PP\del{ \hmuB - \mu_1 < -\eps,\, \hr \in \cR} \difeps \\
    &+ \int_{0}^{\infty} \PP\del{ \hmuB - \mu_1 > \eps,\, \hr \in \cR} \difeps \\
    \stackrel{}{=}\,& \tilcO \del{\del{\displaystyle \max_{r \in \cR} \fr{1}{\sum_{j \in \cBs(r)}N_j}\sum_{i \in \cBp(r)}N_i\Delta_i}^2 \wedge \del{\fr{1}{N_1}}} \\
    &+ \tilcO \del{\del{\max_{r \in \cR} \max_{k=1}^{d(r)} \max_{\substack{S: \cBs(r) \subseteq \Scal \subseteq \cBp(r) \\ \abs{\Scal}=n_*(r)+k }}\fr{k\sum_{j \in \Scal \sm \cBs(r)}N_j}{\del{\sum_{j \in \Scal}N_j}^2}} \wedge \del{\fr{1}{N_1}}} \\
    &+ \tilcO \del{\del{\fr{\log(K)}{\min_{r \in \cR}\sum_{j \in \cBs(r)}N_j}} \wedge \del{\fr{1}{N_1}}} \\
    &+ \tilcO \del{\fr{1}{KN_1}} \\
    &+ \tilcO \del{\del{\max_{r \in \cR} \max_{k=1}^{d(r)} \max_{\substack{S: \cBs(r) \subseteq \Scal \subseteq \cBp(r) \\ \abs{\Scal}=n_*(r)+k }}\fr{k\sum_{j \in \Scal \sm \cBs(r)}N_j}{\del{\sum_{j \in \Scal}N_j}^2}\log\del{\fr{ed}{k}}\log(K)} \wedge \del{\fr{1}{N_1}\log\del{KS}}} \\
    &+ \tilcO \del{\del{\fr{\log(K)}{\min_{r \in \cR}\sum_{j \in \cBs(r)}N_j}} \wedge \del{\fr{1}{N_1}\log\del{KS}}}  \\
    &+ \tilcO \del{\fr{1}{KN_1}\log\del{KS}} \\
    \stackrel{}{=}\,& \tilcO \del{\del{\displaystyle \max_{r \in \cR} \fr{1}{\sum_{j \in \cBs(r)}N_j}\sum_{i \in \cBp(r)}N_i\Delta_i}^2 \wedge \del{\fr{1}{N_1}\log\del{KS}}} \\
    &+ \tilcO \del{\del{\max_{r \in \cR} \max_{k=1}^{d(r)} \max_{\substack{S: \cBs(r) \subseteq \Scal \subseteq \cBp(r) \\ \abs{\Scal}=n_*(r)+k }}\fr{k\sum_{j \in \Scal \sm \cBs(r)}N_j}{\del{\sum_{j \in \Scal}N_j}^2}\log\del{\fr{ed}{k}}\log(K)} \wedge \del{\fr{1}{N_1}\log\del{KS}}} \\
    &+ \tilcO \del{\del{\fr{\log(K)}{\min_{r \in \cR}\sum_{j \in \cBs(r)}N_j}} \wedge \del{\fr{1}{N_1}\log\del{KS}}} \\
    &+ \tilcO \del{\fr{1}{KN_1}\log\del{KS}}
  \end{align*}
  
  Finally,
  \begin{align*}
    &\MSE(\hmuhaver) \\
    \stackrel{}{=}\,& \int_{0}^{\infty} \PP\del{ \abs{\hmuB - \mu_1} < \eps,\, \exists i,\, \abs{\hmu_i - \mu_i} \ge \qgam \gam_i} \\
    &+ \int_{0}^{\infty} \PP\del{ \abs{\hmuB - \mu_1} < \eps,\, \forall i,\, \abs{\hmu_i - \mu_i} < \qgam \gam_i} \\
    \stackrel{}{\le}\,& \int_{0}^{\infty} \PP\del{ \abs{\hmuB - \mu_1} < \eps,\, \exists i,\, \abs{\hmu_i - \mu_i} \ge \qgam \gam_i} \\
    &+ \int_{0}^{\infty} \PP\del{ \abs{\hmuB - \mu_1} < \eps,\, \hr \in \cR} \\
    \stackrel{}{=}\,& \tilcO \del{\del{\displaystyle \max_{r \in \cR} \fr{1}{\sum_{j \in \cBs(r)}N_j}\sum_{i \in \cBp(r)}N_i\Delta_i}^2 \wedge \del{\fr{1}{N_1}\log\del{KS}}} \\
    &+ \tilcO \del{\del{\max_{r \in \cR} \max_{k=1}^{d(r)} \max_{\substack{S: \cBs(r) \subseteq \Scal \subseteq \cBp(r) \\ \abs{\Scal}=n_*(r)+k }}\fr{k\sum_{j \in \Scal \sm \cBs(r)}N_j}{\del{\sum_{j \in \Scal}N_j}^2}\log\del{\fr{ed}{k}}\log(K)} \wedge \del{\fr{1}{N_1}\log\del{KS}}} \\
    &+ \tilcO \del{\del{\fr{\log(K)}{\min_{r \in \cR}\sum_{j \in \cBs(r)}N_j}} \wedge \del{\fr{1}{N_1}\log\del{KS}}} \\
    &+ \tilcO \del{\fr{1}{KN_1}\log\del{KS}} \\
    &+ \tilcO \del{\fr{1}{KN_1}\log\del{KS}} \\
    \stackrel{}{=}\,& \tilcO \del{\del{\displaystyle \max_{r \in \cR} \fr{1}{\sum_{j \in \cBs(r)}N_j}\sum_{i \in \cBp(r)}N_i\Delta_i}^2 \wedge \del{\fr{1}{N_1}\log\del{KS}}} \\
    &+ \tilcO \del{\del{\max_{r \in \cR} \max_{k=1}^{d(r)} \max_{\substack{S: \cBs(r) \subseteq \Scal \subseteq \cBp(r) \\ \abs{\Scal}=n_*(r)+k }}\fr{k\sum_{j \in \Scal \sm \cBs(r)}N_j}{\del{\sum_{j \in \Scal}N_j}^2}\log\del{\fr{ed}{k}}\log(K)} \wedge \del{\fr{1}{N_1}\log\del{KS}}} \\
    &+ \tilcO \del{\del{\fr{\log(K)}{\min_{r \in \cR}\sum_{j \in \cBs(r)}N_j}} \wedge \del{\fr{1}{N_1}\log\del{KS}}} \\
    &+ \tilcO \del{\fr{1}{KN_1}\log\del{KS}} \\
  \end{align*}
  
\end{proof}

\subsection{Haver's  Lemma for under deviation}
\begin{lemma}\label{lemma_ga:haver21count2}
  Haver achieves
  \begin{align*}
    &\int_{0}^{\infty} \PP\del{ \hmuB - \mu_1 < -\eps,\, \hr \in \cR} \difeps \\
    \stackrel{}{=}\,& \cO \del{\del{\displaystyle \max_{r \in \cR} \fr{1}{\sum_{j \in \cBs(r)}N_j}\sum_{i \in \cBp(r)}N_i\Delta_i}^2 \wedge \del{\fr{1}{N_1}\log\del{\fr{KS}{N_1}}}} \\
    &+ \cO \del{\del{\max_{r \in \cR} \max_{k=1}^{d(r)} \max_{\substack{S: \cBs(r) \subseteq \Scal \subseteq \cBp(r) \\ \abs{\Scal}=n_*(r)+k }}\fr{k\sum_{j \in \Scal \sm \cBs(r)}N_j}{\del{\sum_{j \in \Scal}N_j}^2}\log\del{\fr{ed}{k}}\log(K)} \wedge \del{\fr{1}{N_1}\log\del{\fr{KS}{N_1}}}} \\
    &+ \cO\del{\del{\fr{\log(K)}{\min_{r \in \cR}\sum_{j \in \cBs(r)}N_j}} \wedge \del{\fr{1}{N_1}\log\del{\fr{KS}{N_1}}}} \\
    &+ \cO \del{\fr{1}{KN_1}\log\del{\fr{KS}{N_1}}}
    % \stackrel{}{=}\,& \cO \del{\del{\displaystyle \max_{r \in \cR} \fr{1}{\sum_{j \in \cBs(r)}N_j}\sum_{i \in \cBp(r)}N_i\Delta_i}^2 \wedge \del{\fr{1}{N_1}\log\del{\fr{KS}{N_1}}}} \\
    % &+ \cO \del{\del{\max_{r \in \cR} \fr{d\sum_{j \in \cBp(r) \sm \cBs(r)}N_j}{\del{\sum_{j \in \cBp(r)}N_j}^2}\log\del{ed}\log(K)} \wedge \del{\fr{1}{N_1}\log\del{\fr{KS}{N_1}}}} \\
    % &+ \cO\del{\del{\fr{\log(K)}{\min_{r \in \cR}\sum_{j \in \cBs(r)}N_j}} \wedge \del{\fr{1}{N_1}\log\del{\fr{KS}{N_1}}}} \\
    % &+ \cO \del{\fr{1}{KN_1}\log\del{\fr{KS}{N_1}}}
  \end{align*}
  where $d = \abs{\cBp(r)} - \abs{\cBs(r)}$, $n^* = \abs{\cBs(r)}$
\end{lemma}

\begin{proof}
  We consider 4 complement events
  \begin{itemize}
  \item $G_0 = \cbr{\cB = \cBs(\hr)}$
  \item $G_1 = \cbr{\cBs(\hr) \subset \cB \subseteq \cBp(\hr)}$
  \item $G_2 = \cbr{\exists i \in \cBs(\hr),\, i \not\in \cB}$
  \item $G_3 = \cbr{\cBs(\hr) \subseteq \cB,\, \exists i \not\in \cBp(\hr),\, i \in \cB}$
  \end{itemize}
  We have 
  \begin{align*}
    &\int_{0}^{\infty} \PP\del{ \hmuB - \mu_1 < -\eps,\, \hr \in \cR} \difeps \\
    \stackrel{}{=}\,& \int_{0}^{\infty} \PP\del{ \hmuB - \mu_1 < -\eps,\, \hr \in \cR,\, G_0} \difeps + \int_{0}^{\infty} \PP\del{ \hmuB - \mu_1 < -\eps,\, \hr \in \cR,\, G_1} \difeps \\
    &+ \int_{0}^{\infty} \PP\del{ \hmuB - \mu_1 < -\eps,\, \hr \in \cR,\, G_2} \difeps + \int_{0}^{\infty} \PP\del{ \hmuB - \mu_1 < -\eps,\, \hr \in \cR,\, G_3} \difeps
  \end{align*}
  We use Lemma~\ref{lemma_g0a:haver21count2} and ~\ref{lemma_g1a:haver21count2} for event $G_0$ 
  \begin{align*}
    &\int_{0}^{\infty} \PP\del{ \hmuB - \mu_1 < -\eps, G_0} \difeps \\
    \stackrel{}{\le}\,& \cO\del{\del{\max_{r \in \cR}\fr{1}{\sum_{j \in \cBs(r)}N_j}\sum_{i \in \cBp(r)}N_i\Delta_i}^2 + \fr{\log(K)}{\min_{r \in \cR}\sum_{j \in \cBs(r)}N_j}},
  \end{align*}
  and $G_1$ respectively
  \begin{align*}
    &\int_{0}^{\infty} \PP\del{ \hmuB - \mu_1 < -\eps, G_1} \difeps \\
    \stackrel{}{\le}\,& \cO \del{\del{\displaystyle \max_{r \in \cR} \max_{\substack{S: \cBs(r) \subseteq \Scal \subseteq \cBp(r) \\ \abs{\Scal}=n_*(r)+k }}\fr{1}{\sum_{j \in \Scal}N_j}\sum_{i \in \Scal}N_i\Delta_i}^2} \\
  &+ \cO \del{\max_{r \in \cR} \max_{k=1}^{d(r)} \max_{\substack{S: \cBs(r) \subseteq \Scal \subseteq \cBp(r) \\ \abs{\Scal}=n_*(r)+k }}\fr{k\sum_{j \in \Scal \sm \cBs(r)}N_j}{\del{\sum_{j \in \Scal}N_j}^2}\log\del{\fr{ed}{k}}\log(K)} \\
  &+ \cO\del{\fr{\log(K)}{\min_{r \in \cR}\sum_{j \in \cBs(r)}N_j}} 
  \end{align*}
  We use Lemma~\ref{lemma_g2:haver21count2} and ~\ref{lemma_g3:haver21count2} to show that $\PP\del{G_2} \le \fr{2K^2}{K^{2\lambda}}$ and $\PP\del{G_3} \le \fr{2K^2}{K^{2\lambda}}$ respectively.

  Consequently, we use Lemma~\ref{lemma_g2a:haver21count2} for both event $G_2$ and $G_3$ to obtain the integrals
  \begin{align*}
    &\int_{0}^{\infty} \PP\del{ \hmuB - \mu_1 < -\eps, G_2} \difeps \\
    \stackrel{}{\le}\,& \cO \del{\min_m \del{\fr{1}{K^2N_m}\log\del{\fr{KS}{N_m}} + \fr{1}{K^{2}}\Delta_m^2}}
  \end{align*}
  and,
  \begin{align*}
    &\int_{0}^{\infty} \PP\del{ \hmuB - \mu_1 < -\eps, G_3} \difeps \\
    \stackrel{}{\le}\,& \cO \del{\min_m \del{\fr{1}{K^2N_m}\log\del{\fr{KS}{N_m}} + \fr{1}{K^{2}}\Delta_m^2}}
  \end{align*}
  Therefore,
  \begin{align*}
    &\int_{0}^{\infty} \PP\del{ \hmuB - \mu_1 < -\eps} \difeps \\
    \stackrel{}{=}\,& \int_{0}^{\infty} \PP\del{ \hmuB - \mu_1 < -\eps, G_0} \difeps + \int_{0}^{\infty} \PP\del{ \hmuB - \mu_1 < -\eps, G_1} \difeps \\
    &+ \int_{0}^{\infty} \PP\del{ \hmuB - \mu_1 < -\eps, G_2} \difeps + \int_{0}^{\infty} \PP\del{ \hmuB - \mu_1 < -\eps, G_3} \difeps \\
    \stackrel{}{\le}\,& \cO\del{\del{\max_{r \in \cR}\fr{1}{\sum_{j \in \cBs(r)}N_j}\sum_{i \in \cBp(r)}N_i\Delta_i}^2 + \fr{\log(K)}{\min_{r \in \cR}\sum_{j \in \cBs(r)}N_j}} \\
    &+ \cO \del{\del{\displaystyle \max_{r \in \cR} \max_{\substack{S: \cBs(r) \subseteq \Scal \subseteq \cBp(r) \\ \abs{\Scal}=n_*(r)+k }}\fr{1}{\sum_{j \in \Scal}N_j}\sum_{i \in \Scal}N_i\Delta_i}^2} \\
    &+ \cO \del{\max_{r \in \cR} \max_{k=1}^{d(r)} \max_{\substack{S: \cBs(r) \subseteq \Scal \subseteq \cBp(r) \\ \abs{\Scal}=n_*(r)+k }}\fr{k\sum_{j \in \Scal \sm \cBs(r)}N_j}{\del{\sum_{j \in \Scal}N_j}^2}\log\del{\fr{ed}{k}}\log(K)} \\
    &+ \cO\del{\fr{\log(K)}{\min_{r \in \cR}\sum_{j \in \cBs(r)}N_j}} \\
    &+ \cO \del{\min_m \del{\fr{1}{K^2N_m}\log\del{\fr{KS}{N_m}} + \fr{1}{K^{2}}\Delta_m^2}} \\
    \stackrel{}{=}\,& \cO \del{\del{\displaystyle \max_{r \in \cR} \max_{\substack{S: \cBs(r) \subseteq \Scal \subseteq \cBp(r) \\ \abs{\Scal}=n_*(r)+k }}\fr{1}{\sum_{j \in \Scal}N_j}\sum_{i \in \Scal}N_i\Delta_i}^2} \\
    &+ \cO \del{\max_{r \in \cR} \max_{k=1}^{d(r)} \max_{\substack{S: \cBs(r) \subseteq \Scal \subseteq \cBp(r) \\ \abs{\Scal}=n_*(r)+k }}\fr{k\sum_{j \in \Scal \sm \cBs(r)}N_j}{\del{\sum_{j \in \Scal}N_j}^2}\log\del{\fr{ed}{k}}\log(K)} \\
    &+ \cO\del{\fr{\log(K)}{\min_{r \in \cR}\sum_{j \in \cBs(r)}N_j}} \\
    &+ \cO \del{\min_m \del{\fr{1}{K^2N_m}\log\del{\fr{KS}{N_m}} + \fr{1}{K^{2}}\Delta_m^2}} \\
    \stackrel{}{\le}\,& \cO \del{\displaystyle \max_{r \in \cR} \fr{1}{\sum_{j \in \cBs(r)}N_j}\sum_{i \in \cBp(r)}N_i\Delta_i}^2 \\
    &+ \cO \del{\max_{r \in \cR} \max_{k=1}^{d(r)} \max_{\substack{S: \cBs(r) \subseteq \Scal \subseteq \cBp(r) \\ \abs{\Scal}=n_*(r)+k }}\fr{k\sum_{j \in \Scal \sm \cBs(r)}N_j}{\del{\sum_{j \in \Scal}N_j}^2}\log\del{\fr{ed}{k}}\log(K)} \\
    &+ \cO\del{\fr{\log(K)}{\min_{r \in \cR}\sum_{j \in \cBs(r)}N_j}} \\
    &+ \cO \del{\min_m \del{\fr{1}{K^2N_m}\log\del{\fr{KS}{N_m}} + \fr{1}{K^{2}}\Delta_m^2}} 
    % \stackrel{}{\le}\,& \cO \del{\displaystyle \max_{r \in \cR} \fr{1}{\sum_{j \in \cBs(r)}N_j}\sum_{i \in \cBp(r)}N_i\Delta_i}^2 \\
    % &+ \cO \del{\max_{r \in \cR} \fr{d\sum_{j \in \cBp(r) \sm \cBs(r)}N_j}{\del{\sum_{j \in \cBp(r)}N_j}^2}\log\del{ed}\log(K)} \\
    % &+ \cO\del{\fr{\log(K)}{\min_{r \in \cR}\sum_{j \in \cBs(r)}N_j}} \\
    % &+ \cO \del{\min_m \del{\fr{1}{K^2N_m}\log\del{\fr{KS}{N_m}} + \fr{1}{K^{2}}\Delta_m^2}} 
    % \stackrel{}{\le}\,& \cO \del{\del{\del{\max_{r \in \cR}\fr{1}{\sum_{j \in \cBs(r)}N_j}\sum_{i \in \cBp(r)}N_i\Delta_i}^2 + \sup_{k=1}^d \max_{\substack{S: \cBs \subseteq \Scal \subseteq \cBp \\ \abs{\Scal}=n^*+k }}\fr{k \sum_{j \in \Scal \sm \cBs}N_j}{\del{\sum_{j \in \Scal}N_j}^2} + \fr{1}{\sum_{j \in \cBs}N_j}} } \\
    % &+ \cO \del{\min_m \del{\fr{1}{K^2N_m}\log\del{\fr{KS}{N_m}} + \fr{1}{K^{2}}\Delta_m^2}}
  \end{align*}

  Furthermore, Lemma~\ref{lemma102.a:haver} states that 
  \begin{align*}
    &\int_{0}^{\infty} \PP\del{ \hmuB - \mu_1 < -\eps} \difeps \\
    \stackrel{}{\le}\,& \cO \del{\min_m \del{\fr{1}{N_m}\log\del{\fr{KS}{N_m}} + \Delta_m^2}}
  \end{align*}
  Combining two results, we have
  \begin{align*}
    &\int_{0}^{\infty} \PP\del{ \hmuB - \mu_1 < -\eps} \difeps \\
    \stackrel{}{=}\,& \cO \del{\del{\displaystyle \max_{r \in \cR} \fr{1}{\sum_{j \in \cBs(r)}N_j}\sum_{i \in \cBp(r)}N_i\Delta_i}^2 \wedge \del{\min_m \del{\fr{1}{N_m}\log\del{\fr{KS}{N_m}} + \Delta_m^2}}} \\
    &+ \cO \del{\del{\max_{r \in \cR} \max_{k=1}^{d(r)} \max_{\substack{S: \cBs(r) \subseteq \Scal \subseteq \cBp(r) \\ \abs{\Scal}=n_*(r)+k }}\fr{k\sum_{j \in \Scal \sm \cBs(r)}N_j}{\del{\sum_{j \in \Scal}N_j}^2}\log\del{\fr{ed}{k}}\log(K)} \wedge \del{\min_m \del{\fr{1}{N_m}\log\del{\fr{KS}{N_m}} + \Delta_m^2}}} \\
    &+ \cO\del{\del{\fr{\log(K)}{\min_{r \in \cR}\sum_{j \in \cBs(r)}N_j}} \wedge \del{\min_m \del{\fr{1}{N_m}\log\del{\fr{KS}{N_m}} + \Delta_m^2}}} \\
    &+ \cO \del{\min_m \del{\fr{1}{K^2N_m}\log\del{\fr{KS}{N_m}} + \fr{1}{K^{2}}\Delta_m^2}} \\
    \stackrel{}{=}\,& \cO \del{\del{\displaystyle \max_{r \in \cR} \fr{1}{\sum_{j \in \cBs(r)}N_j}\sum_{i \in \cBp(r)}N_i\Delta_i}^2 \wedge \del{\fr{1}{N_1}\log\del{\fr{KS}{N_1}}}} \\
    &+ \cO \del{\del{\max_{r \in \cR} \max_{k=1}^{d(r)} \max_{\substack{S: \cBs(r) \subseteq \Scal \subseteq \cBp(r) \\ \abs{\Scal}=n_*(r)+k }}\fr{k\sum_{j \in \Scal \sm \cBs(r)}N_j}{\del{\sum_{j \in \Scal}N_j}^2}\log\del{\fr{ed}{k}}\log(K)} \wedge \del{\fr{1}{N_1}\log\del{\fr{KS}{N_1}}}} \\
    &+ \cO\del{\del{\fr{\log(K)}{\min_{r \in \cR}\sum_{j \in \cBs(r)}N_j}} \wedge \del{\fr{1}{N_1}\log\del{\fr{KS}{N_1}}}} \\
    &+ \cO \del{\fr{1}{K^2N_1}\log\del{\fr{KS}{N_1}}} \tagcmt{upper bound by $m = 1$} \\
    \stackrel{}{=}\,& \cO \del{\del{\displaystyle \max_{r \in \cR} \fr{1}{\sum_{j \in \cBs(r)}N_j}\sum_{i \in \cBp(r)}N_i\Delta_i}^2 \wedge \del{\fr{1}{N_1}\log\del{\fr{KS}{N_1}}}} \\
    &+ \cO \del{\del{\max_{r \in \cR} \max_{k=1}^{d(r)} \max_{\substack{S: \cBs(r) \subseteq \Scal \subseteq \cBp(r) \\ \abs{\Scal}=n_*(r)+k }}\fr{k\sum_{j \in \Scal \sm \cBs(r)}N_j}{\del{\sum_{j \in \Scal}N_j}^2}\log\del{\fr{ed}{k}}\log(K)} \wedge \del{\fr{1}{N_1}\log\del{\fr{KS}{N_1}}}} \\
    &+ \cO\del{\del{\fr{\log(K)}{\min_{r \in \cR}\sum_{j \in \cBs(r)}N_j}} \wedge \del{\fr{1}{N_1}\log\del{\fr{KS}{N_1}}}} \\
    &+ \cO \del{\fr{1}{KN_1}\log\del{\fr{KS}{N_1}}}
    % \stackrel{}{=}\,& \cO \del{\del{\displaystyle \max_{r \in \cR} \fr{1}{\sum_{j \in \cBs(r)}N_j}\sum_{i \in \cBp(r)}N_i\Delta_i}^2 \wedge \del{\fr{1}{N_1}\log\del{KS}}} \\
    % &+ \cO \del{\del{\max_{r \in \cR} \max_{k=1}^{d(r)} \max_{\substack{S: \cBs(r) \subset \Scal \subseteq \cBp(r) \\ \abs{\Scal}=n_*(r)+k }}\fr{k\sum_{j \in \Scal \sm \cBs(r)}N_j}{\del{\sum_{j \in \Scal}N_j}^2}\log\del{\fr{ed}{k}}\log(K)} \wedge \del{\fr{1}{N_1}\log\del{KS}}} \\
    % &+ \cO\del{\del{\fr{\log(K)}{\min_{r \in \cR}\sum_{j \in \cBs(r)}N_j}} \wedge \del{\fr{1}{N_1}\log\del{KS}}} \\
    % &+ \cO \del{\fr{1}{KN_1}\log\del{KS}} \\
  \end{align*}
\end{proof}

\subsubsection{Lemma for event G0a}

\begin{lemma}\label{lemma_g0a:haver21count2}
  In the event of $G_0 = \cbr{\cB = \cBs(\hr)}$, Haver achieves
  \begin{align*}
    &\int_{0}^{\infty} \PP\del{ \hmuB - \mu_1 < -\eps,\, \hr \in \cR,\, G_0 } \difeps \\
    \stackrel{}{\le}\,& 4\del{\max_{r \in \cR}\fr{1}{\sum_{j \in \cBs(r)}N_j}\sum_{i \in \cBp(r)}N_i\Delta_i}^2 + 48\del{\fr{\log(K)}{\min_{r \in \cR}\sum_{j \in \cBs(r)}N_j}}
  \end{align*}
\end{lemma}

\begin{proof}
  We have
  \begin{align*}
    &\PP\del{ \hmuB - \mu_1 < -\eps,\, \hr \in \cR,\, G_0 } \\
    \stackrel{}{=}\,& \PP\del{ \fr{1}{\sum_{j \in \cB}N_j}\sum_{i \in \cB}N_i\hmu_i - \mu_1 < -\eps,\, \hr \in \cR,\, G_0} \\
    \stackrel{}{=}\,& \PP\del{ \fr{1}{\sum_{j \in \cB}N_j}\sum_{i \in \cB}N_i\del{\hmu_i - \mu_1} < -\eps,\, \hr \in \cR,\, G_0} \\
    \stackrel{}{=}\,& \PP\del{ \fr{1}{\sum_{j \in \cB}N_j}\sum_{i \in \cB}N_i\del{\hmu_i - \mu_i} < -\eps + \fr{1}{\sum_{j \in \cB}N_j}\sum_{i \in \cB}N_i\Delta_i,\, \hr \in \cR,\, G_0} \\
    \stackrel{}{=}\,& \PP\del{ \fr{1}{\sum_{j \in \cBs(\hr)}N_j}\sum_{i \in \cBs(\hr)}N_i\del{\hmu_i - \mu_i} < -\eps + \fr{1}{\sum_{j \in \cBs(\hr)}N_j}\sum_{i \in \cBs(\hr)}N_i\Delta_i,\, \hr \in \cR,\, G_0} \tagcmt{use $G_0 = \cbr{\cB = \cBs(\hr)}$} \\
    \stackrel{}{\le}\,& \sum_{r \in \cR}\PP\del{ \fr{1}{\sum_{j \in \cBs(r)}N_j}\sum_{i \in \cBs(r)}N_i\del{\hmu_i - \mu_i} < -\eps + \fr{1}{\sum_{j \in \cBs(r)}N_j}\sum_{i \in \cBs(r)}N_i\Delta_i,\, G_0}  \\
    \stackrel{}{\le}\,& \sum_{r \in \cR} \exp\del{-\fr{1}{2}\del{\sum_{j \in \cBs(r)}N_j}\del{\eps - \fr{1}{\sum_{j \in \cBs(r)}N_j}\sum_{i \in \cBs(r)}N_i\Delta_i}_+^2} \\
    \stackrel{}{\le}\,& K\exp\del{-\fr{1}{2}\del{\min_{r \in \cR} \sum_{j \in \cBs(r)}N_j}\del{\eps - \max_{r \in \cR}\fr{1}{\sum_{j \in \cBs(r)}N_j}\sum_{i \in \cBs(r)}N_i\Delta_i}_+^2} 
  \end{align*}

  Let $q_1 = q_2 = 1$, $z_1 = \fr{1}{16}\del{\min_{r \in \cR}\sum_{j \in \cBs(r)}N_j}$, and
  \begin{align*}
    \eps_0 = \del{2\max_{r \in \cR}\fr{1}{\sum_{j \in \cBs(r)}N_j}\sum_{i \in \cBs(r)}N_i\Delta_i} \vee \del{\sqrt{\fr{16\log(K)}{\min_{r \in \cR}\sum_{j \in \cBs(r)}N_j}}}
  \end{align*}. We claim that, in the regime of $\eps \ge \eps_0$, we have
  \begin{align*}
    \PP\del{ \hmuB - \mu_1 < -\eps,\, \hr \in \cR,\, G_0 } \le q_1\exp\del{-z_1\eps^2}
  \end{align*}
  and in the regime of $\eps < \eps_0$, we have $\PP\del{ \hmuB - \mu_1 < -\eps,\, \hr \in \cR,\, G_0 } \le q_2$.
  
  The second claim is trivial. We prove the first claim as follows. In the regime of $\eps \ge \eps_0$, we have
  \begin{align*}
    &\PP\del{ \hmuB - \mu_1 < -\eps,\, \hr \in \cR,\, G_0 } \\
    \stackrel{}{\le}\,& K\exp\del{-\fr{1}{2}\del{\min_{r \in \cR} \sum_{j \in \cBs(r)}N_j}\del{\eps - \max_{r \in \cR}\fr{1}{\sum_{j \in \cBs(r)}N_j}\sum_{i \in \cBs(r)}N_i\Delta_i}_+^2} \\
    \stackrel{}{\le}\,& K\exp\del{-\fr{1}{2}\del{\min_{r \in \cR} \sum_{j \in \cBs(r)}N_j}\del{\fr{\eps}{2}}^2} \tagcmt{use $\eps \ge \eps_0$} \\
    \stackrel{}{=}\,& K\exp\del{-\fr{1}{8}\del{\min_{r \in \cR} \sum_{j \in \cBs(r)}N_j}\eps^2} \\
    \stackrel{}{=}\,& \exp\del{-\fr{1}{8}\del{\min_{r \in \cR} \sum_{j \in \cBs(r)}N_j}\eps^2 + \log(K)} \\
    \stackrel{}{\le}\,& \exp\del{-\fr{1}{16}\del{\min_{r \in \cR} \sum_{j \in \cBs(r)}N_j}\eps^2} \tagcmt{use $\eps \ge \eps_0$}
  \end{align*}
  
  With the above claim, we use Lemma~\ref{lemma401:utility_integral_with_eps} to bound the integral
  \begin{align*}
    &\int_{0}^{\infty} \PP\del{ \hmuB - \mu_1 < -\eps,\, \hr \in \cR,\, G_0 } \difeps \\
    \stackrel{}{\le}\,& q_1\eps_0^2 + q_2\fr{1}{z_1} \\
    \stackrel{}{=}\,& \del{\del{2\max_{r \in \cR}\fr{1}{\sum_{j \in \cBs(r)}N_j}\sum_{i \in \cBs(r)}N_i\Delta_i} \vee \del{\sqrt{\fr{16\log(K)}{\min_{r \in \cR}\sum_{j \in \cBs(r)}N_j}}}}^2 + 16\del{\fr{1}{\min_{r \in \cR} \sum_{j \in \cBs(r)}N_j}} \\
    \stackrel{}{\le}\,& 4\del{\max_{r \in \cR}\fr{1}{\sum_{j \in \cBs(r)}N_j}\sum_{i \in \cBp(r)}N_i\Delta_i}^2 + 16\del{\fr{\log(K)}{\min_{r \in \cR}\sum_{j \in \cBs(r)}N_j}} + 16\del{\fr{1}{\min_{r \in \cR} \sum_{j \in \cBs(r)}N_j}} \\
    \stackrel{}{=}\,& 4\del{\max_{r \in \cR}\fr{1}{\sum_{j \in \cBs(r)}N_j}\sum_{i \in \cBp(r)}N_i\Delta_i}^2 + 8\del{\fr{\log(K^2)}{\min_{r \in \cR}\sum_{j \in \cBs(r)}N_j}} + 16\del{\fr{1}{\min_{r \in \cR} \sum_{j \in \cBs(r)}N_j}} \\
    \stackrel{}{\le}\,& 4\del{\max_{r \in \cR}\fr{1}{\sum_{j \in \cBs(r)}N_j}\sum_{i \in \cBp(r)}N_i\Delta_i}^2 + 24\del{\fr{\log(K^2)}{\min_{r \in \cR}\sum_{j \in \cBs(r)}N_j}} \tagcmt{use $1 \le \log(K^2)$ with $K \ge 2$} \\
    \stackrel{}{\le}\,& 4\del{\max_{r \in \cR}\fr{1}{\sum_{j \in \cBs(r)}N_j}\sum_{i \in \cBp(r)}N_i\Delta_i}^2 + 48\del{\fr{\log(K)}{\min_{r \in \cR}\sum_{j \in \cBs(r)}N_j}}.
  \end{align*}

\end{proof}

\subsubsection{Lemma for event G1a}

\begin{lemma}\label{lemma_g1a:haver21count2}
  In the event of $G_1 = \cbr{\cBs(\hr) \subset \cB \subseteq \cBp(\hr)}$, Haver achieves
  \begin{align*}
    &\int_{0}^{\infty} \PP\del{ \hmuB - \mu_1  < -\eps,\, \hr \in \cR,\, G_1 } \difeps \le \\
    \stackrel{}{=}\,& 64\del{\displaystyle \max_{r \in \cR} \max_{\substack{S: \cBs(r) \subseteq \Scal \subseteq \cBp(r) \\ \abs{\Scal}=n_*(r)+k }}\fr{1}{\sum_{j \in \Scal}N_j}\sum_{i \in \Scal}N_i\Delta_i}^2 \\
  &+ 512\del{\max_{r \in \cR} \max_{k=1}^{d(r)} \max_{\substack{S: \cBs(r) \subseteq \Scal \subseteq \cBp(r) \\ \abs{\Scal}=n_*(r)+k }}\fr{k\sum_{j \in \Scal \sm \cBs(r)}N_j}{\del{\sum_{j \in \Scal}N_j}^2}\log\del{\fr{ed}{k}}\log(K)} \\
  &+ 192\del{\fr{\log(K)}{\min_{r \in \cR}\sum_{j \in \cBs(r)}N_j}} 
  \end{align*}
  where $d = \abs{\cBp(r)} - \abs{\cBs(r)}$, $n^* = \abs{\cBs(r)}$
\end{lemma}

\begin{proof}
  % For this Lemma, We denote $n^* = \abs{\cBs}$, $n_+ = \abs{\cBs}$ and $d = n_+ - n^*$
  We decompose the integral as follows
  \begin{align*}
    &\int_{0}^{\infty} \PP\del{ \hmuB - \mu_1 < -\eps,\, \hr \in \cR,\, G_1 } \difeps \\
    \stackrel{}{=}\,& \int_{0}^{\infty} \PP\del{ \fr{1}{\sum_{j \in \cB}N_j}\sum_{i \in \cB}N_i\del{\muhat_i - \mu_1} < -\eps,\, \hr \in \cR,\, G_1 } \difeps \\
    \stackrel{}{\le}\,& \int_{0}^{\infty} \PP\del{ \fr{1}{\sum_{j \in \cB}N_j}\sum_{i \in \cBs(\hr)}N_i\del{\muhat_i - \mu_1} < -\fr{\eps}{2},\, \hr \in \cR,\, G_1 } \difeps \\
    &+ \int_{0}^{\infty} \PP\del{ \fr{1}{\sum_{j \in \cB}N_j}\sum_{i \in \cB \sm \cBs(\hr)}N_i\del{\muhat_i - \mu_1} < -\fr{\eps}{2},\, \hr \in \cR,\, G_1 } \difeps 
  \end{align*}

  We bound the probability and integral of these terms respectively. For the first term, we have
  \begin{align*}
    &\PP\del{ \fr{1}{\sum_{j \in \cB}N_j}\sum_{i \in \cBs(\hr)}N_i\del{\muhat_i - \mu_1} < -\fr{\eps}{2},\, \hr \in \cR,\, G_1 } \\
    \stackrel{}{\le}\,& \sum_{r \in \cR} \PP\del{ \fr{1}{\sum_{j \in \cB}N_j}\sum_{i \in \cBs(r)}N_i\del{\muhat_i - \mu_1} < -\fr{\eps}{2},\, G_1 } \\
    \stackrel{}{=}\,& \sum_{r \in \cR} \PP\del{ \sum_{i \in \cBs(r)}N_i\del{\muhat_i - \mu_1} < -\fr{\eps}{2}\sum_{j \in \cB}N_j,\, G_1 } \\
    \stackrel{}{\le}\,& \sum_{r \in \cR} \PP\del{ \sum_{i \in \cBs(r)}N_i\del{\muhat_i - \mu_1} < -\fr{\eps}{2}\sum_{j \in \cBs(r)}N_j,\, G_1 } \tagcmt{use $\sum_{j \in \cB}N_j < -\sum_{j \in \cBs(r)}N_j$}\\
    \stackrel{}{=}\,& \sum_{r \in \cR} \PP\del{ \sum_{i \in \cBs(r)}N_i\del{\muhat_i - \mu_i} < -\fr{\eps}{2}\sum_{j \in \cBs(r)}N_j + \sum_{i \in \cBs(r)}N_i\Delta_i,\, G_1 } \\
    \stackrel{}{\le}\,& \sum_{r \in \cR} \exp\del{-\fr{1}{2}\fr{1}{\sum_{j \in \cBs(r)}N_j}\del{\fr{\eps}{2}\sum_{j \in \cBs(r)}N_j - \sum_{i \in \cBs(r)}N_i\Delta_i}_+^2} \\
    \stackrel{}{=}\,& \sum_{r \in \cR} \exp\del{-\fr{1}{8}\del{\sum_{j \in \cBs(r)}N_j}\del{\eps - \fr{2}{\sum_{j \in \cBs(r)}N_j}\sum_{i \in \cBs(r)}N_i\Delta_i}_+^2} \\
    \stackrel{}{\le}\,& K \exp\del{-\fr{1}{8}\del{\min_{r \in \cR} \sum_{j \in \cBs(r)}N_j}\del{\eps - \max_{r \in \cR}\fr{2}{\sum_{j \in \cBs(r)}N_j}\sum_{i \in \cBs(r)}N_i\Delta_i}_+^2} 
  \end{align*}

  For this term, let $q_1 = 1$, $q_2 = 1$, $z_1 = \fr{1}{32}\del{\min_{r \in \cR}\sum_{j \in \cBs(r)}N_j}$, and
  \begin{align*}
    \eps_0 = \del{4\max_{r \in \cR}\fr{1}{\sum_{j \in \cBs(r)}N_j}\sum_{i \in \cBs(r)}N_i\Delta_i} \vee \del{\sqrt{\fr{64\log(K)}{\min_{r \in \cR}\sum_{j \in \cBs(r)}N_j}}}
  \end{align*}
  
  We claim that, in the regime of $\eps \ge \eps_0$, we have
  \begin{align*}
    \PP\del{ \fr{1}{\sum_{j \in \cB}N_j}\sum_{i \in \cBs(r)}N_i\del{\muhat_i - \mu_1} < -\fr{\eps}{2},\, \hr \in \cR,\, G_1 } \le q_1\exp\del{-z_1\eps^2}.
  \end{align*}
  and in the regime of regime of $\eps \ge \eps_0$, we have
  \begin{align*}
    \PP\del{ \fr{1}{\sum_{j \in \cB}N_j}\sum_{i \in \cBs(\hr)}N_i\del{\muhat_i - \mu_1} < -\fr{\eps}{2},\, \hr \in \cR,\, G_1 } \le q_2.
  \end{align*}
  The second claim is trivial. We prove the first claim as follows. In the regime of $\eps \ge \eps_0$, we have 
  \begin{align*}
    &\PP\del{ \fr{1}{\sum_{j \in \cB}N_j}\sum_{i \in \cBs}N_i\del{\muhat_i - \mu_1} < -\fr{\eps}{2},\, \hr \in \cR,\, G_1 } \\
    \stackrel{}{\le}\,& K\exp\del{-\fr{1}{8}\del{\min_{r \in \cR} \sum_{j \in \cBs}N_j}\del{\eps - \max_{r \in \cR} \fr{2}{\sum_{j \in \cBs}N_j}\sum_{i \in \cBs}N_i\Delta_i}_+^2} \\
    \stackrel{}{\le}\,& K\exp\del{-\fr{1}{8}\del{\min_{r \in \cR} \sum_{j \in \cBs}N_j}\del{\fr{\eps}{2}}^2} \tagcmt{use $\eps \ge \eps_0$} \\
    \stackrel{}{=}\,& K\exp\del{-\fr{1}{32}\del{\min_{r \in \cR} \sum_{j \in \cBs}N_j}\eps^2} \\
    \stackrel{}{=}\,& \exp\del{-\fr{1}{32}\del{\min_{r \in \cR} \sum_{j \in \cBs}N_j}\eps^2 + \log(K)} \\
    \stackrel{}{\le}\,& \exp\del{-\fr{1}{64}\del{\min_{r \in \cR} \sum_{j \in \cBs}N_j}\eps^2 } \tagcmt{use $\eps \ge \eps_0$}
  \end{align*}
  
  With the above claim, we use Lemma~\ref{lemma401:utility_integral_with_eps} to bound the integral
  \begin{align*}
    &\int_{0}^{\infty} \PP\del{ \fr{1}{\sum_{j \in \cB}N_j}\sum_{i \in \cBs}N_i\del{\muhat_i - \mu_1} < -\fr{\eps}{2},\, \hr \in \cR,\, G_1 } \difeps \\
    \stackrel{}{\le}\,& q_1\eps_0^2 + q_2\fr{1}{z_1} \\
    \stackrel{}{=}\,& \del{\del{4\max_{r \in \cR}\fr{1}{\sum_{j \in \cBs(r)}N_j}\sum_{i \in \cBs(r)}N_i\Delta_i} \vee \del{\sqrt{\fr{64\log(K)}{\min_{r \in \cR}\sum_{j \in \cBs(r)}N_j}}}}^2 + 64\del{\fr{1}{\min_{r \in \cR}\sum_{j \in \cBs(r)}N_j}} \\
    \stackrel{}{\le}\,& 16\del{\max_{r \in \cR}\fr{1}{\sum_{j \in \cBs(r)}N_j}\sum_{i \in \cBs(r)}N_i\Delta_i} + 64\del{\fr{\log(K)}{\min_{r \in \cR}\sum_{j \in \cBs(r)}N_j}} + 64\del{\fr{1}{\min_{r \in \cR}\sum_{j \in \cBs(r)}N_j}} \\
    \stackrel{}{=}\,& 16\del{\max_{r \in \cR}\fr{1}{\sum_{j \in \cBs(r)}N_j}\sum_{i \in \cBs(r)}N_i\Delta_i} + 32\del{\fr{\log(K^2)}{\min_{r \in \cR}\sum_{j \in \cBs(r)}N_j}} + 64\del{\fr{1}{\min_{r \in \cR}\sum_{j \in \cBs(r)}N_j}} \\
    \stackrel{}{\le}\,& 16\del{\max_{r \in \cR}\fr{1}{\sum_{j \in \cBs(r)}N_j}\sum_{i \in \cBs(r)}N_i\Delta_i} + 96\del{\fr{\log(K^2)}{\min_{r \in \cR}\sum_{j \in \cBs(r)}N_j}} \tagcmt{use $1 \le \log(K^2)$ with $K \ge 2$} \\
    \stackrel{}{=}\,& 16\del{\max_{r \in \cR}\fr{1}{\sum_{j \in \cBs(r)}N_j}\sum_{i \in \cBs(r)}N_i\Delta_i} + 192\del{\fr{\log(K)}{\min_{r \in \cR}\sum_{j \in \cBs(r)}N_j}}
  \end{align*}

  For the second term, we have 
  \begin{align*}
    &\PP\del{\fr{1}{\sum_{j \in \cB}N_j} \sum_{i \in \cB \sm \cBs(\hr)}N_i\del{\muhat_i - \mu_1} < -\fr{\eps}{2},\, \hr \in \cR,\, G_1} \\
    % \stackrel{}{\le}\,& \sum_{r \in \cR} \PP\del{\fr{1}{\sum_{j \in \cB}N_j} \sum_{i \in \cB \sm \cBs(r)}N_i\del{\muhat_i - \mu_1} < -\fr{\eps}{2},\, G_1} \\
    \stackrel{}{=}\,& \PP\del{\fr{1}{\sum_{j \in \cB}N_j} \sum_{i \in \cB \sm \cBs(\hr)}N_i\del{\muhat_i - \mu_i} < -\fr{\eps}{2} + \fr{1}{\sum_{j \in \cB}N_j} \sum_{i \in \cB \sm \cBs(\hr)}N_i\Delta_i,\, G_1} \\
    \stackrel{}{\le}\,& \sum_{r \in \cR} \sum_{k=1}^{d}\sum_{\substack{S: \cBs(r) \subset \Scal \subseteq \cBp(r) \\ \abs{\Scal}=n^*+k }} \sum_{r \in \cR} \PP\del{\fr{1}{\sum_{j \in \Scal}N_j} \sum_{i \in \Scal \sm \cBs(r)}N_i\del{\muhat_i - \mu_i} < -\fr{\eps}{2} + \fr{1}{\sum_{j \in \Scal}N_j} \sum_{i \in \Scal \sm \cBs(r)}N_i\Delta_i} \tagcmt{use $d = \abs{\cBp(r)} - \abs{\cBs(r)}$ and $n^* = \abs{\cBs(r)}$} \\
    \stackrel{}{=}\,& \sum_{r \in \cR} \sum_{k=1}^{d}\sum_{\substack{S: \cBs(r) \subset \Scal \subseteq \cBp(r) \\ \abs{\Scal}=n^*+k }} \exp\del{-\fr{1}{2}\del{\fr{\del{\sum_{j \in \Scal}N_j}^2}{\sum_{j \in \Scal \sm \cBs(r)}N_j}}\del{\fr{\eps}{2} - \fr{1}{\sum_{j \in \Scal}N_j}\sum_{i \in \Scal \sm \cBs(r)}N_i\Delta_i}_{+}^2} \\
    \stackrel{}{=}\,& \sum_{r \in \cR} \sum_{k=1}^{d}\sum_{\substack{S: \cBs(r) \subset \Scal \subseteq \cBp(r) \\ \abs{\Scal}=n^*+k }} \exp\del{-\fr{1}{8}\del{\fr{\del{\sum_{j \in \Scal}N_j}^2}{\sum_{j \in \Scal \sm \cBs(r)}N_j}}\del{\eps - \fr{2}{\sum_{j \in \Scal}N_j}\sum_{i \in \Scal \sm \cBs(r)}N_i\Delta_i}_{+}^2} \\
    \stackrel{}{\le}\,& \sum_{r \in \cR} \sum_{k=1}^{d}\sum_{\substack{S: \cBs(r) \subset \Scal \subseteq \cBp(r) \\ \abs{\Scal}=n^*+k }} \exp\del{-\fr{1}{8}\del{\min_{r \in \cR}\min_{k=1}^d\min_{\substack{S: \cBs(r) \subset \Scal \subseteq \cBp(r) \\ \abs{\Scal}=n_*(r)+k }}\fr{\del{\sum_{j \in \Scal}N_j}^2}{\sum_{j \in \Scal \sm \cBs(r)}N_j}}\del{\eps - \max_{r \in \cR}\max_{\substack{S: \cBs(r) \subset \Scal \subseteq \cBp(r) \\ \abs{\Scal}=n_*(r)+k }} \fr{2}{\sum_{j \in \Scal}N_j}\sum_{i \in \Scal \sm \cBs(r)}N_i\Delta_i}_{+}^2} \\
    \stackrel{}{=}\,& \sum_{r \in \cR} \sum_{k=1}^{d}\binom{d}{k} \exp\del{-\fr{1}{8}\del{\min_{r \in \cR}\min_{k=1}^d\min_{\substack{S: \cBs(r) \subset \Scal \subseteq \cBp(r) \\ \abs{\Scal}=n_*(r)+k }}\fr{\del{\sum_{j \in \Scal}N_j}^2}{\sum_{j \in \Scal \sm \cBs(r)}N_j}}\del{\eps - \max_{r \in \cR}\max_{\substack{S: \cBs(r) \subset \Scal \subseteq \cBp(r) \\ \abs{\Scal}=n_*(r)+k }} \fr{2}{\sum_{j \in \Scal}N_j}\sum_{i \in \Scal \sm \cBs(r)}N_i\Delta_i}_{+}^2} \\
  \end{align*}

  For this term, let $q_1 = q_2 = 1$, $z_1 = \fr{1}{128}\del{\displaystyle \min_{r  \in \cR} \min_{k=1}^{d} \min_{\substack{S: \cBs(r) \subset \Scal \subseteq \cBp(r) \\ \abs{\Scal}=n_*(r)+k }}\fr{\del{\sum_{j \in \Scal}N_j}^2}{\sum_{j \in \Scal \sm \cBs(r)}N_j}}$, and
  \begin{align*}
    \eps_0 = \del{4\displaystyle \max_{r  \in \cR} \max_{\substack{S: \cBs(r) \subset \Scal \subseteq \cBp(r)}}\fr{1}{\sum_{j \in \Scal}N_j}\sum_{i \in \Scal}N_i\Delta_i} \vee \del{\sqrt{\displaystyle \max_{r  \in \cR}  \max_{k=1}^{d(r)} \max_{\substack{S: \cBs(r) \subset \Scal \subseteq \cBp(r) \\ \abs{\Scal}=n_*(r)+k }}\fr{128k\sum_{j \in \Scal \sm \cBs(r)}N_j}{\del{\sum_{j \in \Scal}N_j}^2}\log\del{\fr{ed}{k}}\log(K^2)}}
  \end{align*}
  We claim that, in the regime of $\eps \ge \eps_0$, we have
  \begin{align*}
    \PP\del{\fr{1}{\sum_{j \in \cB}N_j} \sum_{i \in \cB \sm \cBs(r)}N_i\del{\muhat_i - \mu_1} < -\fr{\eps}{2},\, \hr \in \cR,\, G_1} \le q_1\exp\del{-z_1\eps^2}
  \end{align*}
  and in the regime of $\eps < \eps_0$, we have
  \begin{align*}
    \PP\del{\fr{1}{\sum_{j \in \cB}N_j} \sum_{i \in \cB \sm \cBs(r)}N_i\del{\muhat_i - \mu_1} < -\fr{\eps}{2},\, \hr \in \cR,\, G_1} \le q_2
  \end{align*}
  The second claim is trivial. We prove the first claim as follows. In the regime of $\eps \ge \eps_0$, we have 
  \begin{align*}
    &\PP\del{\fr{1}{\sum_{j \in \cB}N_j} \sum_{i \in \cB \sm \cBs(r)}N_i\del{\muhat_i - \mu_1} < -\fr{\eps}{2},\, \hr \in \cR,\, G_1} \\
    \stackrel{}{=}\,& \sum_{r \in \cR} \sum_{k=1}^{d}\binom{d}{k} \exp\del{- \fr{1}{8}\del{\min_{r  \in \cR}\min_{k=1}^d\min_{\substack{S: \cBs(r) \subset \Scal \subseteq \cBp(r) \\ \abs{\Scal}=n_*(r)+k }}\fr{\del{\sum_{j \in \Scal}N_j}^2}{\sum_{j \in \Scal \sm \cBs(r)}N_j}}\del{\eps - \max_{r  \in \cR} \max_{\substack{S: \cBs(r) \subset \Scal \subseteq \cBp(r) \\ \abs{\Scal}=n_*(r)+k }} \fr{2}{\sum_{j \in \Scal}N_j}\sum_{i \in \Scal \sm \cBs(r)}N_i\Delta_i}_{+}^2} \\
    \stackrel{}{\le}\,& \sum_{r \in \cR} \sum_{k=1}^{d}\binom{d}{k} \exp\del{-\fr{1}{8}\del{\min_{r  \in \cR} \min_{k=1}^d\min_{\substack{S: \cBs(r) \subset \Scal \subseteq \cBp(r) \\ \abs{\Scal}=n_*(r)+k }}\fr{\del{\sum_{j \in \Scal}N_j}^2}{\sum_{j \in \Scal \sm \cBs(r)}N_j}}\del{\fr{\eps}{2}}^2} \tagcmt{use $\eps \ge \eps_0$} \\
  \stackrel{}{=}\,& \sum_{r \in \cR} \sum_{k=1}^{d}\binom{d}{k} \exp\del{-\fr{1}{32}\del{\min_{r  \in \cR} \min_{k=1}^d\min_{\substack{S: \cBs(r) \subset \Scal \subseteq \cBp(r) \\ \abs{\Scal}=n_*(r)+k }}\fr{\del{\sum_{j \in \Scal}N_j}^2}{\sum_{j \in \Scal \sm \cBs(r)}N_j}}\eps^2} \\
  \stackrel{}{\le}\,& \sum_{r \in \cR} \sum_{k=1}^{d}\del{\fr{ed}{k}}^k \exp\del{-\fr{1}{32}\del{ \min_{r  \in \cR} \min_{k=1}^d\min_{\substack{S: \cBs(r) \subset \Scal \subseteq \cBp(r) \\ \abs{\Scal}=n_*(r)+k }}\fr{\del{\sum_{j \in \Scal}N_j}^2}{\sum_{j \in \Scal \sm \cBs(r)}N_j}}\eps^2} \tagcmt{use Stirling's formula, Lemma~\ref{xlemma:stirling_formula}} \\
  \stackrel{}{=}\,& \sum_{r \in \cR} \sum_{k=1}^{d} \exp\del{-\fr{1}{32}\del{\min_{r  \in \cR} \min_{k=1}^d\min_{\substack{S: \cBs(r) \subset \Scal \subseteq \cBp(r) \\ \abs{\Scal}=n_*(r)+k }}\fr{\del{\sum_{j \in \Scal}N_j}^2}{\sum_{j \in \Scal \sm \cBs(r)}N_j}}\eps^2 + k\log\del{\fr{ed}{k}}} \\
  \stackrel{}{\le}\,& \sum_{r \in \cR} \sum_{k=1}^{d} \exp\del{-\fr{1}{64}\del{ \min_{r  \in \cR} \min_{k=1}^d\min_{\substack{S: \cBs(r) \subset \Scal \subseteq \cBp(r) \\ \abs{\Scal}=n_*(r)+k }}\fr{\del{\sum_{j \in \Scal}N_j}^2}{\sum_{j \in \Scal \sm \cBs(r)}N_j}}\eps^2} \tagcmt{use $\eps \ge \eps_0$} \\
  \stackrel{}{\le}\,& K d \exp\del{-\fr{1}{64}\del{\min_{r  \in \cR}  \min_{k=1}^{d} \min_{\substack{S: \cBs(r) \subset \Scal \subseteq \cBp(r) \\ \abs{\Scal}=n_*(r)+k }}\fr{\del{\sum_{j \in \Scal}N_j}^2}{\sum_{j \in \Scal \sm \cBs(r)}N_j}}\eps^2} \\
  \stackrel{}{=}\,& \exp\del{-\fr{1}{64}\del{\min_{r  \in \cR}  \min_{k=1}^{d} \min_{\substack{S: \cBs(r) \subset \Scal \subseteq \cBp(r) \\ \abs{\Scal}=n_*(r)+k }}\fr{\del{\sum_{j \in \Scal}N_j}^2}{\sum_{j \in \Scal \sm \cBs(r)}N_j}}\eps^2 + \ln(Kd)} \\
  \stackrel{}{\le}\,& \exp\del{-\fr{1}{128}\del{\min_{r  \in \cR} \min_{k=1}^{d} \min_{\substack{S: \cBs(r) \subset \Scal \subseteq \cBp(r) \\ \abs{\Scal}=n_*(r)+k }}\fr{\del{\sum_{j \in \Scal}N_j}^2}{\sum_{j \in \Scal \sm \cBs(r)}N_j}}\eps^2 } \tagcmt{use $\eps \ge \eps_0 $}
\end{align*}
With the above claim, we use Lemma~\ref{lemma401:utility_integral_with_eps} to bound the integral
\begin{align*}
  &\int_{0}^{\infty} \PP\del{\fr{1}{\sum_{j \in \cB}N_j} \sum_{i \in \cB \sm \cBs(r)}N_i\del{\muhat_i - \mu_1} < -\fr{\eps}{2},\, \hr \in \cR,\, G_1} \difeps \\
  \stackrel{}{\le}\,& q_1\eps_0^2 + q_2\fr{1}{z_1} \\
  \stackrel{}{\le}\,& \del{\del{4\displaystyle \max_{r \in \cR} \max_{\substack{S: \cBs(r) \subset \Scal \subseteq \cBp(r)}}\fr{1}{\sum_{j \in \Scal}N_j}\sum_{i \in \Scal}N_i\Delta_i} \vee \del{\sqrt{\displaystyle \max_{r \in \cR} \max_{k=1}^{d(r)} \max_{\substack{S: \cBs(r) \subset \Scal \subseteq \cBp(r) \\ \abs{\Scal}=n_*(r)+k }}\fr{128k\sum_{j \in \Scal \sm \cBs(r)}N_j}{\del{\sum_{j \in \Scal}N_j}^2}\log\del{\fr{ed}{k}}\log(K^2)}}}^2 \\
  &+ 128\del{\max_{r \in \cR} \max_{k=1}^{d(r)} \max_{\substack{S: \cBs(r) \subset \Scal \subseteq \cBp(r) \\ \abs{\Scal}=n_*(r)+k }}\fr{\sum_{j \in \Scal \sm \cBs(r)}N_j}{\del{\sum_{j \in \Scal}N_j}^2}} \\
  \stackrel{}{\le}\,& 16\del{\displaystyle \max_{r \in \cR} \max_{\substack{S: \cBs(r) \subset \Scal \subseteq \cBp(r)}}\fr{1}{\sum_{j \in \Scal}N_j}\sum_{i \in \Scal}N_i\Delta_i}^2 + 128\del{\max_{r \in \cR} \max_{k=1}^{d(r)} \max_{\substack{S: \cBs(r) \subset \Scal \subseteq \cBp(r) \\ \abs{\Scal}=n_*(r)+k }}\fr{k\sum_{j \in \Scal \sm \cBs(r)}N_j}{\del{\sum_{j \in \Scal}N_j}^2}\log\del{\fr{ed}{k}}\log(K^2)} \tagcmt{use  $\del{A \vee B}^2 \le A^2 + B^2$} \\
  &+ 128\del{\max_{r \in \cR} \max_{k=1}^{d(r)} \max_{\substack{S: \cBs(r) \subset \Scal \subseteq \cBp(r) \\ \abs{\Scal}=n_*(r)+k }}\fr{128\sum_{j \in \Scal \sm \cBs(r)}N_j}{\del{\sum_{j \in \Scal}N_j}^2}} \\
  \stackrel{}{=}\,& 16\del{\displaystyle \max_{r \in \cR} \max_{\substack{S: \cBs(r) \subset \Scal \subseteq \cBp(r)}}\fr{1}{\sum_{j \in \Scal}N_j}\sum_{i \in \Scal}N_i\Delta_i}^2 + 256\del{\max_{r \in \cR} \max_{k=1}^{d(r)} \max_{\substack{S: \cBs(r) \subset \Scal \subseteq \cBp(r) \\ \abs{\Scal}=n_*(r)+k }}\fr{k\sum_{j \in \Scal \sm \cBs(r)}N_j}{\del{\sum_{j \in \Scal}N_j}^2}\log\del{\fr{ed}{k}}\log(K^2)} \tagcmt{use $1 \le \log\del{\fr{ed}{k}}\,\forall k \in [1,d]$ and $1 \le \log(K^2)\, \forall K \ge 2$} \\
  \stackrel{}{=}\,& 16\del{\displaystyle \max_{r \in \cR} \max_{\substack{S: \cBs(r) \subset \Scal \subseteq \cBp(r)}}\fr{1}{\sum_{j \in \Scal}N_j}\sum_{i \in \Scal}N_i\Delta_i}^2 + 512\del{\max_{r \in \cR} \max_{k=1}^{d(r)} \max_{\substack{S: \cBs(r) \subset \Scal \subseteq \cBp(r) \\ \abs{\Scal}=n_*(r)+k }}\fr{k\sum_{j \in \Scal \sm \cBs(r)}N_j}{\del{\sum_{j \in \Scal}N_j}^2}\log\del{\fr{ed}{k}}\log(K)}
\end{align*}

Combining the two terms, we have 
\begin{align*}
  &\int_{0}^{\infty} \PP\del{ \hmuB - \mu_1 < -\eps,\, \hr \in \cR,\, G_1 } \difeps \\
  \stackrel{}{\le}\,& \int_{0}^{\infty} \PP\del{ \fr{1}{\sum_{j \in \cB}N_j}\sum_{i \in \cBs(r)}N_i\del{\muhat_i - \mu_1} < -\fr{\eps}{2},\, \hr \in \cR,\, G_1 } \difeps \\
  &+ \int_{0}^{\infty} \PP\del{ \fr{1}{\sum_{j \in \cB}N_j}\sum_{i \in \cB \sm \cBs(r)}N_i\del{\muhat_i - \mu_1} < -\fr{\eps}{2},\, \hr \in \cR,\, G_1 } \difeps \\
  \stackrel{}{\le}\,& 16\del{\max_{r \in \cR}\fr{1}{\sum_{j \in \cBs(r)}N_j}\sum_{i \in \cBs(r)}N_i\Delta_i} + 192\del{\fr{\log(K)}{\min_{r \in \cR}\sum_{j \in \cBs(r)}N_j}} \\
  &+ 16\del{\displaystyle \max_{r \in \cR} \max_{\substack{S: \cBs(r) \subset \Scal \subseteq \cBp(r)}}\fr{1}{\sum_{j \in \Scal}N_j}\sum_{i \in \Scal}N_i\Delta_i}^2 + 512\del{\max_{r \in \cR} \max_{k=1}^{d(r)} \max_{\substack{S: \cBs(r) \subset \Scal \subseteq \cBp(r) \\ \abs{\Scal}=n_*(r)+k }}\fr{k\sum_{j \in \Scal \sm \cBs(r)}N_j}{\del{\sum_{j \in \Scal}N_j}^2}\log\del{\fr{ed}{k}}\log(K)} \\
  \stackrel{}{\le}\,& 16\del{\displaystyle \max_{r \in \cR} \max_{\substack{S: \cBs(r) \subset \Scal \subseteq \cBp(r) \\ \abs{\Scal}=n_*(r)+k }}\fr{1}{\sum_{j \in \Scal}N_j}\sum_{i \in \Scal}N_i\Delta_i + \max_{r \in \cR} \fr{1}{\sum_{j \in \cBs(r)}N_j}\sum_{i \in \cBp(r)}N_i\Delta_i}^2 \tagcmt{use $\forall a,b \ge 0,\, a^2 + b^2 \le (a+b)^2$} \\
  &+ 512\del{\max_{r \in \cR} \max_{k=1}^{d(r)} \max_{\substack{S: \cBs(r) \subset \Scal \subseteq \cBp(r) \\ \abs{\Scal}=n_*(r)+k }}\fr{k\sum_{j \in \Scal \sm \cBs(r)}N_j}{\del{\sum_{j \in \Scal}N_j}^2}\log\del{\fr{ed}{k}}\log(K)} \\
  &+ 192\del{\fr{\log(K)}{\min_{r \in \cR}\sum_{j \in \cBs(r)(r)}N_j}} \\
  \stackrel{}{\le}\,& 64\del{\displaystyle \max_{r \in \cR} \max_{\substack{S: \cBs(r) \subseteq \Scal \subseteq \cBp(r) \\ \abs{\Scal}=n_*(r)+k }}\fr{1}{\sum_{j \in \Scal}N_j}\sum_{i \in \Scal}N_i\Delta_i}^2 \\
  &+ 512\del{\max_{r \in \cR} \max_{k=1}^{d(r)} \max_{\substack{S: \cBs(r) \subseteq \Scal \subseteq \cBp(r) \\ \abs{\Scal}=n_*(r)+k }}\fr{k\sum_{j \in \Scal \sm \cBs(r)}N_j}{\del{\sum_{j \in \Scal}N_j}^2}\log\del{\fr{ed}{k}}\log(K)} \\
  &+ 192\del{\fr{\log(K)}{\min_{r \in \cR}\sum_{j \in \cBs(r)}N_j}} \\
  % \stackrel{}{\le}\,& 64\del{\displaystyle \max_{r \in \cR} \fr{1}{\sum_{j \in \cBs(r)}N_j}\sum_{i \in \cBp(r)}N_i\Delta_i}^2 \\
  % &+ 512\del{\max_{r \in \cR} \max_{k=1}^{d(r)} \max_{\substack{S: \cBs(r) \subset \Scal \subseteq \cBp(r) \\ \abs{\Scal}=n_*(r)+k }}\fr{k\sum_{j \in \Scal \sm \cBs(r)}N_j}{\del{\sum_{j \in \Scal}N_j}^2}\log\del{\fr{ed}{k}}\log(K)} \\
  % &+ 192\del{\fr{\log(K)}{\min_{r \in \cR}\sum_{j \in \cBs(r)}N_j}}
\end{align*}

\end{proof}


\begin{lemma}\label{lemma101.a:haver}
  Let $m \in [K]$ be any arm. In Haver, we have 
  \begin{align*}
    \PP\del{ \hmuB - \mu_1 < -\eps } \le 2\exp\del{-\fr{1}{2}N_{m}\del{\eps - \gam_m - \Delta_m}_+^2} 
  \end{align*}
\end{lemma}


\begin{proof}
  We separate the probability into two terms 
  \begin{align*}
    &\PP\del{ \hmuB - \mu_1 < -\eps } \\
    \stackrel{}{=}\,& \PP\del{\hr =  m,\, \hmuB - \mu_1 < -\eps } + \PP\del{\hr \in [K] \sm \cbr{m},\, \hmuB - \mu_1 < -\eps } 
  \end{align*}

  For the first term, we have
  \begin{align*}
    & \PP\del{\hr =  m,\, \hmuB - \mu_1 < -\eps } \\
    \stackrel{}{=}\,& \PP\del{\hr =  m,\, \fr{N_m}{\sum_{j \in \cB}N_j}\muhat_m + \sum_{i \in \cB \setminus \cbr{m}}\fr{N_i}{\sum_{j \in \cB}N_j}\muhat_i - \mu_1 < -\eps } \\
    \stackrel{}{\le}\,& \PP\del{\hr =  m,\, \fr{N_m}{\sum_{j \in \cB}N_j}\muhat_m + \sum_{i \in \cB \setminus \cbr{m}}\fr{N_i}{\sum_{j \in \cB}N_j}\del{\muhat_m - \gam_m} - \mu_1 < -\eps } \tagcmt{use $\forall i \in \cB,\, \muhat_m - \gam_m \le \muhat_i$} \\
    \stackrel{}{=}\,& \PP\del{\muhat_m - \mu_1 < -\eps + \sum_{i \in \cB \setminus \cbr{m}}\fr{N_i}{\sum_{j \in \cB}N_j}\gam_m } \\
    \stackrel{}{\le}\,& \PP\del{\muhat_m - \mu_1 < -\eps + \gam_m} \tagcmt{use $\sum_{i \in \cB \setminus \cbr{m}}\fr{N_i}{\sum_{j \in \cB}N_j} \le 1$} \\
    \stackrel{}{=}\,& \PP\del{\muhat_m - \mu_m < -\eps + \gam_m + \mu_1 - \mu_m} \\
    \stackrel{}{=}\,& \PP\del{\muhat_m - \mu_m < -\eps + \gam_m + \Delta_m} \\
    \stackrel{}{\le}\,& \exp\del{-\frac{N_m\del{\eps - \gam_m - \Delta_m}_+^2}{2}} \tagcmt{by Hoeffding's inequality} 
  \end{align*}

  For the second term, we have
  \begin{align*}
    & \PP\del{\hr \in [K] \sm \cbr{m},\, \hmuB - \mu_1 < -\eps } \\
    \stackrel{}{=}\,& \PP\del{\hr \in [K] \sm \cbr{m},\, \fr{N_{\hr}}{\sum_{j \in \cB}N_j}\muhat_{\hr} + \sum_{i \in \cB \setminus \cbr{\hr}}\fr{N_i}{\sum_{j \in \cB}N_j}\muhat_i - \mu_1 < -\eps } \\
    \stackrel{}{\le}\,& \PP\del{\hr \in [K] \sm \cbr{m},\, \fr{N_{\hr}}{\sum_{j \in \cB}N_j}\muhat_{\hr} + \sum_{i \in \cB \setminus \cbr{\hr}}\fr{N_i}{\sum_{j \in \cB}N_j}\del{\muhat_{\hr} - \gam_{\hr}} - \mu_1 < -\eps } \tagcmt{use $\forall i \in \cB,\, \muhat_{i} \ge \muhat_{\hr} - \gam_{\hr}$} \\
    \stackrel{}{=}\,& \PP\del{\hr \in [K] \sm \cbr{m},\, \muhat_{\hr} - \mu_1 < -\eps + \sum_{i \in \cB \setminus \cbr{\hr}}\fr{N_i}{\sum_{j \in \cB}N_j}\gam_{\hr}} \\
    \stackrel{}{\le}\,& \PP\del{\hr \in [K] \sm \cbr{m},\, \muhat_{m} - \gam_{m} + \gam_{\hr} - \mu_1 < -\eps + \sum_{i \in \cB \setminus \cbr{\hr}}\fr{N_i}{\sum_{j \in \cB}N_j}\gam_{\hr}} \tagcmt{by def of $\hr$, $\muhat_{\hr} > \muhat_{m} - \gam_{m} + \gam_{\hr}$}\\
    \stackrel{}{=}\,& \PP\del{\hr \in [K] \sm \cbr{m},\, \muhat_{m}  - \mu_1 < -\eps + \gam_{m} - \gam_{\hr} + \sum_{i \in \cB \setminus \cbr{\hr}}\fr{N_i}{\sum_{j \in \cB}N_j}\gam_{\hr}} \\
    \stackrel{}{\le}\,& \PP\del{\hr \in [K] \sm \cbr{m},\, \muhat_{m}  - \mu_1 < -\eps + \gam_{m} - \gam_{\hr} + \gam_{\hr}} \tagcmt{use $\sum_{i \in \cB \setminus \cbr{m}}\fr{N_i}{\sum_{j \in \cB}N_j} \le 1$} \\
    \stackrel{}{=}\,& \PP\del{\hr \in [K] \sm \cbr{m},\, \muhat_{m}  - \mu_1 < -\eps + \gam_{m}} \\
    \stackrel{}{\le}\,& \PP\del{\muhat_m - \mu_1 < -\eps + \gam_m} \\
    \stackrel{}{=}\,& \PP\del{\muhat_m - \mu_m < -\eps + \gam_m + \mu_1 - \mu_m} \\
    \stackrel{}{=}\,& \PP\del{\muhat_m - \mu_m < -\eps + \gam_m + \Delta_m} \\
    \stackrel{}{\le}\,& \exp\del{-\frac{N_m\del{\eps - \gam_m - \Delta_m}_+^2}{2}} \tagcmt{by Hoeffding's inequality} 
  \end{align*}

  Combining two terms, we have
  \begin{align*}
    &\PP\del{ \hmuB - \mu_1 < -\eps } \\
    \stackrel{}{=}\,& \PP\del{\hr =  m,\, \hmuB - \mu_1 < -\eps } + \PP\del{\hr \in [K] \sm \cbr{m},\, \hmuB - \mu_1 < -\eps } \\
    \stackrel{}{\le}\,& 2\exp\del{-\frac{N_m\del{\eps - \gam_m - \Delta_m}_+^2}{2}}
  \end{align*}
  
\end{proof}

\begin{lemma}\label{lemma102.a:haver}
  In Haver, we have
  \begin{align*}
    \int_{0}^{\infty} \PP\del{\hmuB - \mu_1 < -\eps} \difeps \le \min_m \del{\fr{352}{N_m}\log\del{\fr{KS}{N_m}}  + 4\Delta_m^2}
  \end{align*}
\end{lemma}

\begin{proof}
  Lemma~\ref{lemma101.a:haver} states that, for any arm $m \in [K]$,
  \begin{align*}
    \PP\del{ \hmuB - \mu_1 < -\eps } \le 2\exp\del{-\fr{1}{2}N_{m}\del{\eps - \gam_m - \Delta_m}_+^2} 
  \end{align*}
  Let $q_1 = q_2 = 1$, $\eps_0 = 2\del{\gam_m + \Delta_m}$ and $z_1 = \fr{1}{16}N_m$. We claim that, in the regime of $\eps \ge \eps_0$, we have
  \begin{align*}
    \PP\del{ \hmuB - \mu_1 < -\eps } \le q_1\exp\del{-z_1\eps^2}
  \end{align*}
  and in the regime of $\eps < \eps_0$, we have $f(\eps) \le q_2$.

  We prove the claim as follows. In the regime of $\eps \ge \eps_0$, we have
  \begin{align*}
    & \PP\del{ \hmuB - \mu_1 < -\eps }  \\
    \stackrel{}{\le}\,& 2\exp\del{-\fr{1}{2}N_{m}\del{\eps-\gam_{m}-\Delta_{m}}_+^2} \\
    \stackrel{}{\le}\,& 2\exp\del{-\fr{1}{2}N_{m}\del{\fr{\eps}{2}}^2} \tagcmt{use $\eps \ge \eps_0 = 2\del{\gam_m + \Delta_m}$} \\
    \stackrel{}{=}\,& 2\exp\del{-\fr{1}{8}N_{m}\eps^2} \\
    \stackrel{}{=}\,& \exp\del{-\fr{1}{8}N_{m}\eps^2 + \log(2)} \\
    \stackrel{}{\le}\,& \exp\del{-\fr{1}{16}N_{m}\eps^2} \tagcmt{use $\eps \ge \eps_0 \ge \gam_m$}
  \end{align*}
  In the regime of $\eps < \eps_0$, we have $\PP\del{ \hmuB - \mu_1 < -\eps } \le 1$.
  
  With the above claim, we use Lemma~\ref{lemma401:utility_integral_with_eps} to bound the integral
  \begin{align*}
    &\int_{0}^{\infty} \PP\del{ \hmuB - \mu_1 < -\eps } \difeps \\
    \stackrel{}{\le}\,& q_2\eps_0^2 + q_1\fr{1}{z_1} \\
    \stackrel{}{=}\,& \del{2\del{\gam_m + \Delta_m}}^2 + \fr{16}{N_m} \\
    \stackrel{}{\le}\,& 4\gam_m^2  + 4\Delta_m^2 + \fr{16}{N_m} \\
    \stackrel{}{\le}\,& 4\fr{18}{N_m}\log\del{\del{\fr{KS}{N_m}}^{2\lambda}}  + 4\Delta_m^2 + \fr{16}{N_m} \tagcmt{use $\gam_m = \sqrt{\fr{18}{N_m}\log\del{\del{\fr{KS}{N_m}}^{2\lambda}}}$} \\
    \stackrel{}{=}\,& \fr{72}{N_m}\log\del{\del{\fr{KS}{N_m}}^{4}}  + 4\Delta_m^2 + \fr{16}{N_m} \tagcmt{choose $\lambda = 2$} \\
    \stackrel{}{\le}\,& \fr{88}{N_m}\log\del{\del{\fr{KS}{N_m}}^4}  + 4\Delta_m^2 \tagcmt{use $1 \le \log\del{\del{\fr{KS}{N_m}}^4}$ with $K \ge 2$} \\
    \stackrel{}{\le}\,& \fr{352}{N_m}\log\del{\fr{KS}{N_m}}  + 4\Delta_m^2 \\
    \stackrel{}{\le}\,& \min_m \del{\fr{352}{N_m}\log\del{\fr{KS}{N_m}}  + 4\Delta_m^2}
  \end{align*}
  
\end{proof}

\begin{lemma}\label{lemma_g2a:haver21count2}
  If an event $G$ sastisfies $\PP\del{G} \le \fr{2K^2}{K^{2\lambda}}$, then Haver achieves
  \begin{align*}
    \int_{0}^{\infty} \PP\del{ \hmuB - \mu_1 < -\eps,\, G } \dif \eps \le \min_m \del{\fr{704}{K^2N_m}\log\del{\fr{KS}{N_m}}  + \fr{8}{K^{2}}\Delta_m^2}
  \end{align*}
\end{lemma}

\begin{proof}
  For any arm $m$, we have 
  \begin{align*}
    &\PP\del{ \hmuB - \mu_1 < -\eps,\, G} \\
    \stackrel{}{\le}\,& \PP\del{ \hmuB - \mu_1 < -\eps} \\
    \stackrel{}{\le}\,& 2\exp\del{-\fr{1}{2}{N_{m}\del{\eps - \gam_{m} - \Delta_{m}}_+^2}} \tagcmt{use Lemma~\ref{lemma101.a:haver}} \\
  \end{align*}
  We also have
  \begin{align*}
    &\PP\del{ \hmuB - \mu_1 < -\eps,\, G} \le \PP\del{G} \le \fr{2K^2}{K^{2\lambda}}
    % \stackrel{}{\le}\,& \PP\del{G} \\
    % \stackrel{}{\le}\,& \fr{2K^2}{K^{2\lambda}}
  \end{align*}
  Thus,
  \begin{align*}
    &\PP\del{ \hmuB - \mu_1 < -\eps,\, G} \le 2\exp\del{-\fr{1}{2}{N_{m}\del{\eps - \gam_{m} - \Delta_{m}}_+^2}} \wedge \fr{2K^2}{K^{2\lambda}}
  \end{align*}
  % We use Lemma~\ref{lemma103.a:haver} to get the integral bound
  % \begin{align*}
  %    \int_{0}^{\infty} \PP\del{ \hmuB - \mu_1 > \eps,\, G } \le \min_m \del{\fr{704}{K^2N_m}\log\del{\fr{KS}{N_m}}  + \fr{8}{K^{2}}\Delta_m^2}
  % \end{align*}

  Let $q_1 = \fr{2K}{K^{\lambda}}$, $q_2 = \fr{2K^2}{K^{2\lambda}}$, $\eps_0 = 2\del{\gam_m + \Delta_m}$ and $z_1 = \fr{1}{16}N_m$. We claim that, in the regime of $\eps \ge \eps_0$, we have
  \begin{align*}
    \PP\del{ \hmuB - \mu_1 < -\eps,\, G} \le q_1\exp\del{-z_1\eps^2}
  \end{align*}
  and in the regime of $\eps < \eps_0$, we have $\PP\del{ \hmuB - \mu_1 < -\eps,\, G} \le q_2$.

  We prove the claim as follows. In the regime of $\eps \ge \eps_0$, we have
  \begin{align*}
    &\PP\del{ \hmuB - \mu_1 < -\eps,\, G}  \\
    \stackrel{}{\le}\,& 2\exp\del{-\fr{1}{2}N_{m}\del{\eps-\gam_{m}-\Delta_{m}}_+^2} \wedge \frac{2K^2}{K^{2\lambda}} \\
    \stackrel{}{\le}\,& \sqrt{2\exp\del{-\fr{1}{2}N_{m}\del{\eps-\gam_{m}-\Delta_{m}}_+^2} \cdot \frac{2K^2}{K^{2\lambda}}} \\
    \stackrel{}{=}\,& \frac{2K}{K^{\lambda}}\exp\del{-\fr{1}{4}N_{m}\del{\eps-\gam_{m}-\Delta_{m}}_+^2} \\
    \stackrel{}{\le}\,& \frac{2K}{K^{\lambda}}\exp\del{-\fr{1}{4}N_{m}\del{\fr{\eps}{2}}^2} \tagcmt{use $\eps \ge \eps_0 = 2\del{\gam_m + \Delta_m}$} \\
    \stackrel{}{=}\,& \frac{2K}{K^{\lambda}}\exp\del{-\fr{1}{16}N_{m}\eps^2} 
  \end{align*}
  In the regime of $\eps < \eps_0$, we have
  \begin{align*}
    &\PP\del{ \hmuB - \mu_1 < -\eps,\, G} \\
    \stackrel{}{\le}\,& 2\exp\del{-\fr{1}{2}N_{m}\del{\eps - \gam_{m} + \Delta_{m}}_+^2} \wedge \frac{2K^2}{K^{2\lambda}} \\
    \stackrel{}{\le}\,& \fr{2K^2}{K^{2\lambda}}
  \end{align*}
  With the above claim, we use Lemma~\ref{lemma401:utility_integral_with_eps} to bound the integral
  \begin{align*}
    &\int_{0}^{\infty} \PP\del{ \hmuB - \mu_1 < -\eps,\, G} \difeps \\
    \stackrel{}{\le}\,& q_2\eps_0^2 + q_1\fr{1}{z_1} \\
    \stackrel{}{=}\,& \fr{2K^2}{K^{2\lambda}}\del{2\del{\gam_m + \Delta_m}}^2 + \fr{2K}{K^{\lambda}}\fr{16}{N_m} \\
    \stackrel{}{\le}\,& \fr{8K^2}{K^{2\lambda}}\gam_m^2  + \fr{8K}{K^{2\lambda}}\Delta_m^2 + \fr{32}{K^{\lambda}N_m} \\
    \stackrel{}{\le}\,& \fr{8K^2}{K^{2\lambda}}\fr{18}{N_m}\log\del{\del{\fr{KS}{N_m}}^{2\lambda}}  + \fr{8K}{K^{2\lambda}}\Delta_m^2 + \fr{32}{K^{\lambda}N_m} \tagcmt{use $\gam_m = \sqrt{\fr{18}{N_m}\log\del{\del{\fr{KS}{N_m}}^{2\lambda}}}$} \\
    \stackrel{}{=}\,& \fr{144K^2}{K^{4}N_m}\log\del{\del{\fr{KS}{N_m}}^{4}}  + \fr{8K}{K^{4}}\Delta_m^2 + \fr{32}{K^{2}N_m} \tagcmt{choose $\lambda = 2$} \\
    \stackrel{}{\le}\,& \fr{176}{K^2N_m}\log\del{\del{\fr{KS}{N_m}}^4}  + \fr{8}{K^{3}}\Delta_m^2 \tagcmt{use $1 \le \log\del{\del{\fr{KS}{N_m}}^4}$ with $K \ge 2$} \\
    \stackrel{}{\le}\,& \fr{704}{K^2N_m}\log\del{\fr{KS}{N_m}}  + \fr{8}{K^{3}}\Delta_m^2 \\
    \stackrel{}{\le}\,& \min_m \del{\fr{704}{K^2N_m}\log\del{\fr{KS}{N_m}}  + \fr{8}{K^{2}}\Delta_m^2} \\
  \end{align*}
  
\end{proof}


\subsection{Haver's Lemma for upper deviation}

\begin{lemma}\label{lemma_gb:haver21count2}
  Haver achieves
  \begin{align*}
    &\int_{0}^{\infty} \PP\del{ \hmuB - \mu_1 > \eps,\, \hr \in \cR} \difeps \\
    \stackrel{}{=}\,& \cO \del{\del{\max_{r \in \cR} \max_{k=1}^{d(r)} \max_{\substack{S: \cBs(r) \subseteq \Scal \subseteq \cBp(r) \\ \abs{\Scal}=n_*(r)+k }}\fr{k\sum_{j \in \Scal \sm \cBs(r)}N_j}{\del{\sum_{j \in \Scal}N_j}^2}\log\del{\fr{ed}{k}}\log(K)} \wedge \del{\fr{1}{N_1}\log\del{KS}}} \\
    &+ \cO \del{\del{\fr{\log(K)}{\min_{r \in \cR}\sum_{j \in \cBs(r)}N_j}} \wedge \del{\fr{1}{N_1}\log\del{KS}}}  \\
    &+ \cO \del{\fr{1}{KN_1}\log\del{KS}}
  \end{align*}
  where $d = \abs{\cBp(r)} - \abs{\cBs(r)}$, $n^* = \abs{\cBs(r)}$
\end{lemma}

\begin{proof}
  
  We consider 4 complement events
  \begin{itemize}
  \item $G_0 = \cbr{\cB = \cBs(\hr)}$
  \item $G_1 = \cbr{\cBs(\hr) \subset \cB \subseteq \cBp(\hr)}$
  \item $G_2 = \cbr{\cBs(\hr) \subseteq \cB,\, \exists i \not\in \cBs(\hr),\, i \in \cB}$
  \item $G_3 = \cbr{\exists i \in \cBs(\hr),\, i \not\in \cB}$
  \end{itemize}

  We have
  \begin{align*}
    &\int_{0}^{\infty} \PP\del{ \hmuB - \mu_1 > \eps,\, \hr \in \cR} \difeps \\
    \stackrel{}{=}\,& \int_{0}^{\infty} \PP\del{ \hmuB - \mu_1 > \eps,\, \hr \in \cR,\, G_0} \difeps + \int_{0}^{\infty} \PP\del{ \hmuB - \mu_1 > \eps,\, \hr \in \cR,\, G_1} \difeps \\
    &+ \int_{0}^{\infty} \PP\del{ \hmuB - \mu_1 > \eps,\, \hr \in \cR,\, G_2} \difeps + \int_{0}^{\infty} \PP\del{ \hmuB - \mu_1 > \eps,\, \hr \in \cR,\, G_3} \difeps
  \end{align*}
  
  We use Lemma~\ref{lemma_g0b:haver21count2} and ~\ref{lemma_g1b:haver21count2} for event $G_0$ 
  \begin{align*}
    &\int_{0}^{\infty} \PP\del{ \hmuB - \mu_1 > \eps,\, \hr \in \cR,\, G_0} \difeps \\
    \stackrel{}{\le}\,& \cO\del{\fr{\log(K)}{\min_{r \in \cR}\sum_{j \in \cBs(r)}N_j}},
  \end{align*}
  and $G_1$ respectively
  \begin{align*}
    &\int_{0}^{\infty} \PP\del{ \hmuB - \mu_1 > \eps, G_1} \difeps \\
    \stackrel{}{\le}\,& \cO \del{\max_{r \in \cR} \max_{k=1}^{d(r)} \max_{\substack{S: \cBs(r) \subseteq \Scal \subseteq \cBp(r) \\ \abs{\Scal}=n_*(r)+k }}\fr{k\sum_{j \in \Scal \sm \cBs(r)}N_j}{\del{\sum_{j \in \Scal}N_j}^2}\log\del{\fr{ed}{k}}\log(K) + \fr{\log(K)}{\min_{r \in \cR}\sum_{j \in \cBs(r)}N_j}}
  \end{align*}
  We use Lemma~\ref{lemma_g2:haver21count2} and ~\ref{lemma_g3:haver21count2} to show that $\PP\del{G_2} \le \fr{2K^2}{K^{2\lambda}}$ and $\PP\del{G_3} \le \fr{2K^2}{K^{2\lambda}}$ respectively.

  Consequently, we use Lemma~\ref{lemma_g2b:haver21count2} for both event $G_2$ and $G_3$ to obtain the integrals
  \begin{align*}
    &\int_{0}^{\infty} \PP\del{ \hmuB - \mu_1 > \eps, G_2} \difeps \\
    \stackrel{}{\le}\,& \cO \del{\fr{1}{KN_1}\log\del{KS}}
  \end{align*}
  and,
  \begin{align*}
    &\int_{0}^{\infty} \PP\del{ \hmuB - \mu_1 > \eps, G_3} \difeps \\
    \stackrel{}{\le}\,& \cO \del{\fr{1}{KN_1}\log\del{KS}}
  \end{align*}
  Therefore,
  \begin{align*}
    &\int_{0}^{\infty} \PP\del{ \hmuB - \mu_1 > \eps} \difeps \\
    \stackrel{}{\le}\,& \int_{0}^{\infty} \PP\del{ \hmuB - \mu_1 > \eps, G_0} \difeps + \int_{0}^{\infty} \PP\del{ \hmuB - \mu_1 > \eps, G_1} \difeps \\
    &+ \int_{0}^{\infty} \PP\del{ \hmuB - \mu_1 > \eps, G_2} \difeps + \int_{0}^{\infty} \PP\del{ \hmuB - \mu_1 > \eps, G_3} \difeps \\
    \stackrel{}{\le}\,& \cO\del{\fr{\log(K)}{\min_{r \in \cR}\sum_{j \in \cBs(r)}N_j}} \\
    &+ \cO \del{\max_{r \in \cR} \max_{k=1}^{d(r)} \max_{\substack{S: \cBs(r) \subseteq \Scal \subseteq \cBp(r) \\ \abs{\Scal}=n_*(r)+k }}\fr{k\sum_{j \in \Scal \sm \cBs(r)}N_j}{\del{\sum_{j \in \Scal}N_j}^2}\log\del{\fr{ed}{k}}\log(K) + \fr{\log(K)}{\min_{r \in \cR}\sum_{j \in \cBs(r)}N_j}} \\
    &+ \cO \del{\fr{1}{KN_1}\log\del{KS}} \\
    \stackrel{}{=}\,& \cO \del{\max_{r \in \cR}\sup_{k=1}^d \max_{\substack{S: \cBs(r) \subseteq \Scal \subseteq \cBp(r) \\ \abs{\Scal}=n^*+k }}\fr{k \sum_{j \in \Scal \sm \cBs(r)}N_j}{\del{\sum_{j \in \Scal}N_j}^d}\log\del{\fr{ed}{k}}\log(K)} \\
    &+ \cO \del{\fr{\log(K)}{\min_{r \in \cR}\sum_{j \in \cBs(r)}N_j}} \\
    &+ \cO \del{\fr{1}{KN_1}\log\del{KS}} \\
    % \stackrel{}{\le}\,& \cO \del{\max_{r \in \cR}\fr{d \sum_{j \in \cBp(r) \sm \cBs(r)}N_j}{\del{\sum_{j \in \cBp(r)}N_j}^2}\log\del{ed}\log(K)} \\
    % &+ \cO \del{\fr{\log(K)}{\min_{r \in \cR}\sum_{j \in \cBs(r)}N_j}} \\
    % &+ \cO \del{\fr{1}{KN_1}\log\del{KS}}
  \end{align*}
  Furthermore, Lemma~\ref{lemma102.b:haver21count2} states that
  \begin{align*}
    \int_{0}^{\infty} \PP\del{ \hmuB - \mu_1 > \eps} \difeps \le \cO\del{\fr{1}{N_1}\log\del{KS}}
  \end{align*}
  Combining two results, we have
  \begin{align*}
    &\int_{0}^{\infty} \PP\del{ \hmuB - \mu_1 > \eps} \difeps \\
    \stackrel{}{\le}\,& \cO \del{\del{\max_{r \in \cR} \max_{k=1}^{d(r)} \max_{\substack{S: \cBs(r) \subseteq \Scal \subseteq \cBp(r) \\ \abs{\Scal}=n_*(r)+k }}\fr{k\sum_{j \in \Scal \sm \cBs(r)}N_j}{\del{\sum_{j \in \Scal}N_j}^2}\log\del{\fr{ed}{k}}\log(K)} \wedge \del{\fr{1}{N_1}\log\del{KS}}} \\
    &+ \cO \del{\del{\fr{\log(K)}{\min_{r \in \cR}\sum_{j \in \cBs(r)}N_j}} \wedge \del{\fr{1}{N_1}\log\del{KS}}}  \\
    &+ \cO \del{\fr{1}{KN_1}\log\del{KS}}
  \end{align*}
  % \begin{align*}
  %   \int_{0}^{\infty} \PP\del{ \hmuB - \mu_1 > \eps} \difeps \\
  %   % \stackrel{}{\le}\,& \cO \del{{\sup_{k=1}^d \max_{\substack{S: \cBs \subseteq \Scal \subseteq \cBp \\ \abs{\Scal}=n^*+k }}\fr{k \sum_{j \in \Scal \sm \cBs}N_j}{\del{\sum_{j \in \Scal}N_j}^2} + \fr{1}{\sum_{j \in \cBs}N_j}} \wedge \del{\fr{1}{N_1}\log\del{KS}}} \\
  %    % &+ \cO \del{\fr{1}{KN_1}\log\del{KS}}
  % \end{align*}
\end{proof}


\subsubsection{Lemma for event G0b}

\begin{lemma}\label{lemma_g0b:haver21count2}
  In the event of $G_0 = \cbr{\cB = \cBs(\hr)}$, Haver achieves
  \begin{align*}
    &\int_{0}^{\infty} \PP\del{ \hmuB - \mu_1 > \eps,\, \hr \in \cR,\, G_0 } \difeps \le 10\del{\fr{\log(K)}{\min_{r \in \cR}\sum_{j \in \cBs(r)}N_j}}
  \end{align*}
\end{lemma}

\begin{proof}
  We have
  \begin{align*}
    &\PP\del{ \hmuB - \mu_1 > \eps,\, \hr \in \cR,\, G_0 } \\
    \stackrel{}{=}\,& \PP\del{ \fr{1}{\sum_{j \in \cB}N_j}\sum_{i \in \cB}N_i\hmu_i - \mu_1 > \eps,\, \hr \in \cR,\, G_0} \\
    \stackrel{}{=}\,& \PP\del{ \fr{1}{\sum_{j \in \cB}N_j}\sum_{i \in \cB}N_i\del{\hmu_i - \mu_1} > \eps,\, \hr \in \cR,\, G_0} \\
    \stackrel{}{=}\,& \PP\del{ \fr{1}{\sum_{j \in \cB}N_j}\sum_{i \in \cB}N_i\del{\hmu_i - \mu_i} > \eps + \fr{1}{\sum_{j \in \cB}N_j}\sum_{i \in \cB}N_i\Delta_i,\, \hr \in \cR,\, G_0} \\
    \stackrel{}{=}\,& \PP\del{ \fr{1}{\sum_{j \in \cBs(\hr)}N_j}\sum_{i \in \cBs(\hr)}N_i\del{\hmu_i - \mu_i} > \eps + \fr{1}{\sum_{j \in \cBs(\hr)}N_j}\sum_{i \in \cBs(\hr)}N_i\Delta_i,\, \hr \in \cR,\, G_0} \tagcmt{use $G_0 = \cbr{\cB = \cBs(\hr)}$} \\
    \stackrel{}{=}\,& \sum_{r \in \cR} \PP\del{ \fr{1}{\sum_{j \in \cBs(r)}N_j}\sum_{i \in \cBs(r)}N_i\del{\hmu_i - \mu_i} > \eps + \fr{1}{\sum_{j \in \cBs(r)}N_j}\sum_{i \in \cBs(r)}N_i\Delta_i,\, G_0}  \\
    \stackrel{}{\le}\,& \sum_{r \in \cR}\exp\del{-\fr{1}{2}\del{\sum_{j \in \cBs(\hr)}N_j}\del{\eps + \fr{1}{\sum_{j \in \cBs(r)}N_j}\sum_{i \in \cBp(r)}N_i\Delta_i}^2} \\
    \stackrel{}{\le}\,& \sum_{r \in \cR}\exp\del{-\fr{1}{2}\del{\sum_{j \in \cBs(r)}N_j}\eps^2} \\
    \stackrel{}{\le}\,& K\exp\del{-\fr{1}{2}\del{\min_{r \in \cR}\sum_{j \in \cBs(r)}N_j}\eps^2}
  \end{align*}

  Let $q_1 = q_2 = 1$, $z_1 = \fr{1}{4}\del{\min_{r \in \cR}\sum_{j \in \cBs(r)}N_j}$, and $\eps_0 = \sqrt{\fr{4\log(K)}{\min_{r \in \cR}\sum_{j \in \cBs(r)}N_j}}$. We claim that, in the regime of $\eps \ge \eps_0$, we have
  \begin{align*}
    \PP\del{ \hmuB - \mu_1 > \eps,\, \hr \in \cR,\, G_0 } \le q_1\exp\del{-z_1\eps^2}
  \end{align*}
  and in the regime of $\eps < \eps_0$, we have
  \begin{align*}
    \PP\del{ \hmuB - \mu_1 > \eps,\, \hr \in \cR,\, G_0 } \le q_2.
  \end{align*}
  The second claim is trivial. We prove the first claim as follows. In the regime of $\eps \ge \eps_0$, we have
  \begin{align*}
    &\PP\del{ \hmuB - \mu_1 > \eps,\, \hr \in \cR,\, G_0 } \\
    \stackrel{}{\le}\,& K\exp\del{-\fr{1}{2}\del{\min_{r \in \cR}\sum_{j \in \cBs(r)}N_j}\eps^2} \\
    \stackrel{}{\le}\,& \exp\del{-\fr{1}{2}\del{\min_{r \in \cR}\sum_{j \in \cBs(r)}N_j}\eps^2 + \log(K)} \\
    \stackrel{}{\le}\,& \exp\del{-\fr{1}{4}\del{\min_{r \in \cR}\sum_{j \in \cBs(r)}N_j}\eps^2} \tagcmt{use $\eps \ge \eps_0$}
  \end{align*}
  
  With the above claim, we use Lemma~\ref{lemma401:utility_integral_with_eps} to bound the integral
  \begin{align*}
    &\int_{0}^{\infty} \PP\del{ \hmuB - \mu_1 > \eps,\, G_0 } \difeps \\
    \stackrel{}{\le}\,& q_1\eps_0^2 + q_2\fr{1}{z_1} \\
    \stackrel{}{=}\,& 4\del{\fr{\log(K)}{\min_{r \in \cR}\sum_{j \in \cBs(r)}N_j}} + 4\del{\fr{4}{\sum_{r \in \cR}\sum_{j \in \cBs(r)}N_j}} \\
    \stackrel{}{=}\,& 2\del{\fr{\log(K^2)}{\min_{r \in \cR}\sum_{j \in \cBs(r)}N_j}} + 4\del{\fr{4}{\sum_{r \in \cR}\sum_{j \in \cBs(r)}N_j}} \\
    \stackrel{}{\le}\,& 5\del{\fr{\log(K^2)}{\min_{r \in \cR}\sum_{j \in \cBs(r)}N_j}} \tagcmt{use $K \ge 2$} \\
    \stackrel{}{\le}\,& 10\del{\fr{\log(K)}{\min_{r \in \cR}\sum_{j \in \cBs(r)}N_j}}
  \end{align*}

\end{proof}

\subsubsection{Lemma for event G1b}

\begin{lemma}\label{lemma_g1b:haver21count2}
  In the event of $G_1 = \cbr{\cBs(\hr) \subset \cB \subseteq \cBp(\hr)}$, Haver achieves
  \begin{align*}
    &\int_{0}^{\infty} \PP\del{ \hmuB - \mu_1  > \eps,\, \hr \in \cR,\, G_1 } \difeps \\
    \stackrel{}{=}\,& 128\del{\max_{r \in \cR} \max_{k=1}^{d(r)} \max_{\substack{S: \cBs(r) \subseteq \Scal \subseteq \cBp(r) \\ \abs{\Scal}=n_*(r)+k }}\fr{k\sum_{j \in \Scal \sm \cBs(r)}N_j}{\del{\sum_{j \in \Scal}N_j}^2}\log\del{\fr{ed}{k}}\log(K)} + 48\del{\fr{\log(K)}{\min_{r \in \cR}\sum_{j \in \cBs(r)}N_j}}
  \end{align*}
  where $d = \abs{\cBp(r)} - \abs{\cBs(r)}$, $n^* = \abs{\cBs(r)}$
\end{lemma}

\begin{proof}
  % For this Lemma, We denote $n^* = \abs{\cBs}$, $n_+ = \abs{\cBs}$ and $d = n_+ - n^*$
  We decompose the integral as follow:
  \begin{align*}
    &\int_{0}^{\infty} \PP\del{ \hmuB - \mu_1 > \eps,\, \hr \in \cR,\, G_1 } \difeps \\
    \stackrel{}{=}\,& \int_{0}^{\infty} \PP\del{ \fr{1}{\sum_{j \in \cB}N_j}\sum_{i \in \cB}N_i\del{\muhat_i - \mu_1} > \eps,\, \hr \in \cR,\, G_1 } \difeps \\
    \stackrel{}{\le}\,& \int_{0}^{\infty} \PP\del{ \fr{1}{\sum_{j \in \cB}N_j}\sum_{i \in \cBs(\hr)}N_i\del{\muhat_i - \mu_1} > \fr{\eps}{2},\, \hr \in \cR,\, G_1 } \difeps \\
    &+ \int_{0}^{\infty} \PP\del{ \fr{1}{\sum_{j \in \cB}N_j}\sum_{i \in \cB \sm \cBs(\hr)}N_i\del{\muhat_i - \mu_1} > \fr{\eps}{2},\, \hr \in \cR,\, G_1 } \difeps 
  \end{align*}

  We bound the probability and integral of these terms respectively. For the first term, we have  
  \begin{align*}
    &\PP\del{ \fr{1}{\sum_{j \in \cB}N_j}\sum_{i \in \cBs(\hr)}N_i\del{\muhat_i - \mu_1} > \fr{\eps}{2},\, \hr \in \cR,\, G_1 } \\
    \stackrel{}{=}\,& \PP\del{ \sum_{i \in \cBs(\hr)}N_i\del{\muhat_i - \mu_1} > \fr{\eps}{2}\sum_{j \in \cB}N_j,\, \hr \in \cR,\, G_1 } \\
    \stackrel{}{\le}\,& \PP\del{ \sum_{i \in \cBs(\hr)}N_i\del{\muhat_i - \mu_1} \ge \fr{\eps}{2}\sum_{j \in \cBs(\hr)}N_j,\, \hr \in \cR,\, G_1 } \tagcmt{use $\sum_{j \in \cB}N_j \ge \sum_{j \in \cBs(\hr)}N_j$}\\
    \stackrel{}{=}\,& \PP\del{ \sum_{i \in \cBs(\hr)}N_i\del{\muhat_i - \mu_i} \ge \fr{\eps}{2}\sum_{j \in \cBs(\hr)}N_j + \sum_{i \in \cBs(\hr)}N_i\Delta_i,\, \hr \in \cR,\, G_1 } \\
    \stackrel{}{\le}\,& \sum_{r \in \cR} \PP\del{ \sum_{i \in \cBs(r)}N_i\del{\muhat_i - \mu_i} \ge \fr{\eps}{2}\sum_{j \in \cBs(r)}N_j + \sum_{i \in \cBs(r)}N_i\Delta_i,\, G_1 } \\
    \stackrel{}{\le}\,& \sum_{r \in \cR} \exp\del{-\fr{1}{2}\fr{1}{\sum_{j \in \cBs(r)}N_j}\del{\fr{\eps}{2}\sum_{j \in \cBs(r)}N_j + \sum_{i \in \cBs(r)}N_i\Delta_i}^2} \\
    \stackrel{}{\le}\,& \sum_{r \in \cR} \exp\del{-\fr{1}{2}\fr{1}{\sum_{j \in \cBs(r)}N_j}\del{\fr{\eps}{2}\sum_{j \in \cBs(r)}N_j}^2} \\
    \stackrel{}{=}\,& \sum_{r \in \cR} \exp\del{-\fr{1}{8}\del{\sum_{j \in \cBs(r)}N_j}\eps^2} \\
    \stackrel{}{\le}\,& K\exp\del{-\fr{1}{8}\del{\min_{r \in \cR}\sum_{j \in \cBs(r)}N_j}\eps^2}
  \end{align*}

  For this term, let $q_1 = q_2 = 1$, $z_1 = \fr{1}{16}\del{\min_{r \in \cR}\sum_{j \in \cBs(r)}N_j}$, and $\eps_0 = \sqrt{\fr{16\log(K)}{\min_{r \in \cR}\sum_{j \in \cBs(r)}N_j}}$. We claim that, in the regime of $\eps \ge \eps_0$, we have
  \begin{align*}
    \PP\del{ \fr{1}{\sum_{j \in \cB}N_j}\sum_{i \in \cBs(\hr)}N_i\del{\muhat_i - \mu_1} > \fr{\eps}{2},\, \hr \in \cR,\, G_1 } \le q_1\exp\del{-z_1\eps^2}
  \end{align*}
  and in the regime of $\eps < \eps_0$, we have
  \begin{align*}
    \PP\del{ \fr{1}{\sum_{j \in \cB}N_j}\sum_{i \in \cBs(\hr)}N_i\del{\muhat_i - \mu_1} > \fr{\eps}{2},\, \hr \in \cR,\, G_1 } \le q_2.
  \end{align*}
  The second claim is trivial. We prove the first claim as follows. In the regime of $\eps \ge \eps_0$, we have
  \begin{align*}
    & \PP\del{ \fr{1}{\sum_{j \in \cB}N_j}\sum_{i \in \cBs(\hr)}N_i\del{\muhat_i - \mu_1} > \fr{\eps}{2},\, \hr \in \cR,\, G_1 } \\
    \stackrel{}{\le}\,& K\exp\del{-\fr{1}{8}\del{\min_{r \in \cR}\sum_{j \in \cBs(r)}N_j}\eps^2} \\
    \stackrel{}{=}\,& \exp\del{-\fr{1}{8}\del{\min_{r \in \cR}\sum_{j \in \cBs(r)}N_j}\eps^2 + \log(K)} \\
    \stackrel{}{\le}\,& \exp\del{-\fr{1}{16}\del{\min_{r \in \cR}\sum_{j \in \cBs(r)}N_j}\eps^2 } \tagcmt{use $\eps \ge \eps_0$}
  \end{align*}
  With the above claim, we use Lemma~\ref{lemma401:utility_integral_with_eps} to bound the integral
  \begin{align*}
    &\int_{0}^{\infty} \PP\del{ \fr{1}{\sum_{j \in \cB}N_j}\sum_{i \in \cBs(\hr)}N_i\del{\muhat_i - \mu_1} > \fr{\eps}{2},\, \hr \in \cR,\, G_1 } \difeps \\
    \stackrel{}{\le}\,& q_1\eps_0^2 + q_2\fr{1}{z_1} \\
    \stackrel{}{=}\,& 16\del{\fr{\log(K)}{\min_{r \in \cR}\sum_{j \in \cBs(r)}N_j}} + 16\del{\fr{1}{\min_{r \in \cR}\sum_{j \in \cBs(r)}N_j}} \\
    \stackrel{}{=}\,& 8\del{\fr{\log(K^2)}{\min_{r \in \cR}\sum_{j \in \cBs(r)}N_j}} + 16\del{\fr{1}{\min_{r \in \cR}\sum_{j \in \cBs(r)}N_j}} \\
    \stackrel{}{\le}\,& 24\del{\fr{\log(K^2)}{\min_{r \in \cR}\sum_{j \in \cBs(r)}N_j}} \tagcmt{use $K \ge 2$} \\
    \stackrel{}{=}\,& 48\del{\fr{\log(K)}{\min_{r \in \cR}\sum_{j \in \cBs(r)}N_j}}
  \end{align*}

  For the second term, we have
  \begin{align*}
    &\PP\del{\fr{1}{\sum_{j \in \cB}N_j} \sum_{i \in \cB \sm \cBs(\hr)}N_i\del{\muhat_i - \mu_1} > \fr{\eps}{2},\, \hr \in \cR,\, G_1} \\
    \stackrel{}{=}\,& \PP\del{\fr{1}{\sum_{j \in \cB}N_j} \sum_{i \in \cB \sm \cBs(\hr)}N_i\del{\muhat_i - \mu_i} > \fr{\eps}{2} + \fr{1}{\sum_{j \in \cB}N_j} \sum_{i \in \cB \sm \cBs(\hr)}N_i\Delta_i,\, \hr \in \cR,\, G_1} \\
    \stackrel{}{\le}\,& \PP\del{\fr{1}{\sum_{j \in \cB}N_j} \sum_{i \in \cB \sm \cBs(\hr)}N_i\del{\muhat_i - \mu_i} > \fr{\eps}{2},\, \hr \in \cR,\, G_1} \\
    % \stackrel{}{\le}\,& \sum_{r \in \cR} \PP\del{\fr{1}{\sum_{j \in \cB}N_j} \sum_{i \in \cB \sm \cBs(r)}N_i\del{\muhat_i - \mu_i} > \fr{\eps}{2},\, G_1} \\
    \stackrel{}{\le}\,& \sum_{r \in \cR} \sum_{k=1}^{d}\sum_{\substack{S: \cBs(r) \subset \Scal \subseteq \cBp(r) \\ \abs{\Scal}=n^*+k }} \PP\del{\fr{1}{\sum_{j \in \Scal}N_j} \sum_{i \in \Scal \sm \cBs(r)}N_i\del{\muhat_i - \mu_i} > \fr{\eps}{2},\, G_1} \tagcmt{use $d = \abs{\cBp(r)} - \abs{\cBs(r)}$ and $n^* = \abs{\cBs(r)}$} \\
    \stackrel{}{\le}\,& \sum_{r \in \cR} \sum_{k=1}^{d}\sum_{\substack{S: \cBs(r) \subset \Scal \subseteq \cBp(r) \\ \abs{\Scal}=n^*+k }} \exp\del{-\fr{1}{2}\del{\fr{\del{\sum_{j \in \Scal}N_j}^2}{\sum_{j \in \Scal \sm \cBs(\hr)}N_j}}\del{\fr{\eps}{2}}^2} \tagcmt{use Hoeffding's inequality} \\
    \stackrel{}{=}\,& \sum_{r \in \cR} \sum_{k=1}^{d}\sum_{\substack{S: \cBs(r) \subset \Scal \subseteq \cBp(r) \\ \abs{\Scal}=n^*+k }} \exp\del{-\fr{1}{8}\del{\fr{\del{\sum_{j \in \Scal}N_j}^2}{\sum_{j \in \Scal \sm \cBs(r)}N_j}}\eps^2} \\
    \stackrel{}{\le}\,& \sum_{r \in \cR}\sum_{k=1}^{d}\sum_{\substack{S: \cBs(r) \subset \Scal \subseteq \cBp(r) \\ \abs{\Scal}=n^*+k }} \exp\del{-\fr{1}{8}\del{\min_{r \in \cR} \min_{k=1}^d\min_{\substack{S: \cBs(r) \subset \Scal \subseteq \cBp(r) \\ \abs{\Scal}=n_*(r)+k }}\fr{\del{\sum_{j \in \Scal}N_j}^2}{\sum_{j \in \Scal \sm \cBs(r)}N_j}}\eps^2} \\
    \stackrel{}{=}\,& \sum_{r \in \cR}\sum_{k=1}^{d}\binom{d}{k} \exp\del{-\fr{1}{8}\del{\min_{r \in \cR} \min_{k=1}^d\min_{\substack{S: \cBs(r) \subset \Scal \subseteq \cBp(r) \\ \abs{\Scal}=n_*(r)+k }}\fr{\del{\sum_{j \in \Scal}N_j}^2}{\sum_{j \in \Scal \sm \cBs(r)}N_j}}\eps^2}.
  \end{align*}

  For this term, let $q_1 = q_2 = 1$,
  \begin{align*}
    z_1 = \fr{1}{32}\del{\min_{r \in \cR} \min_{k=1}^{d} \min_{\substack{S: \cBs(r) \subset \Scal \subseteq \cBp(r) \\ \abs{\Scal}=n_*(r)+k }}\fr{\del{\sum_{j \in \Scal}N_j}^2}{\sum_{j \in \Scal \sm \cBs(r)}N_j}}
  \end{align*}, and 
  \begin{align*}
    \eps_0 = \sqrt{\displaystyle \max_{r \in \cR} \max_{k=1}^{d(r)} \max_{\substack{S: \cBs(r) \subset \Scal \subseteq \cBp(r) \\ \abs{\Scal}=n_*(r)+k }}\fr{32k\sum_{j \in \Scal \sm \cBs(r)}N_j}{\del{\sum_{j \in \Scal}N_j}^2}\log\del{\fr{ed}{k}}\log\del{K^2}}
  \end{align*}

  We claim that, in the regime of $\eps \ge \eps_0$, we have 
  \begin{align*}
    \PP\del{\fr{1}{\sum_{j \in \cB}N_j} \sum_{i \in \cB \sm \cBs(r)}N_i\del{\muhat_i - \mu_1} > \fr{\eps}{2},\, \hr \in \cR,\, G_1} \le q_1\exp\del{-z_1\eps^2}
  \end{align*}
  and in the regime of $\eps < \eps_0$, we have
  \begin{align*}
    \PP\del{\fr{1}{\sum_{j \in \cB}N_j} \sum_{i \in \cB \sm \cBs(r)}N_i\del{\muhat_i - \mu_1} > \fr{\eps}{2},\, \hr \in \cR,\, G_1} \le q_2
  \end{align*}
  The second claim is trivial. We prove the first claim as follows. In the regime of $\eps \ge \eps_0$, we have 
  \begin{align*}
    &\PP\del{\fr{1}{\sum_{j \in \cB}N_j} \sum_{i \in \cB \sm \cBs(r)}N_i\del{\muhat_i - \mu_1} > \fr{\eps}{2},\, \hr \in \cR,\, G_1} \\
    \stackrel{}{\le}\,& \sum_{r \in \cR} \sum_{k=1}^{d}\binom{d}{k} \exp\del{-\fr{1}{8}\del{\min_{r \in \cR} \min_{k=1}^d\min_{\substack{S: \cBs(r) \subset \Scal \subseteq \cBp(r) \\ \abs{\Scal}=n_*(r)+k }}\fr{\del{\sum_{j \in \Scal}N_j}^2}{\sum_{j \in \Scal \sm \cBs(r)}N_j}}\eps^2} \\
    \stackrel{}{\le}\,& \sum_{r \in \cR} \sum_{k=1}^{d}\del{\fr{ed}{k}}^k \exp\del{-\fr{1}{8}\del{\min_{r \in \cR} \min_{k=1}^d\min_{\substack{S: \cBs(r) \subset \Scal \subseteq \cBp(r) \\ \abs{\Scal}=n_*(r)+k }}\fr{\del{\sum_{j \in \Scal}N_j}^2}{\sum_{j \in \Scal \sm \cBs(r)}N_j}}\eps^2} \tagcmt{use Stirling's formula, Lemma ~\ref{xlemma:stirling_formula}} \\
    \stackrel{}{=}\,& \sum_{r \in \cR} \sum_{k=1}^{d} \exp\del{-\fr{1}{8}\del{\min_{r \in \cR}\min_{k=1}^d\min_{\substack{S: \cBs(r) \subset \Scal \subseteq \cBp(r) \\ \abs{\Scal}=n_*(r)+k }}\fr{\del{\sum_{j \in \Scal}N_j}^2}{\sum_{j \in \Scal \sm \cBs(r)}N_j}}\eps^2 + k\log\del{\fr{ed}{k}}} \\
    \stackrel{}{\le}\,& \sum_{r \in \cR} \sum_{k=1}^{d} \exp\del{-\fr{1}{16}\del{\min_{r \in \cR}\min_{k=1}^d\min_{\substack{S: \cBs(r) \subset \Scal \subseteq \cBp(r) \\ \abs{\Scal}=n_*(r)+k }}\fr{\del{\sum_{j \in \Scal}N_j}^2}{\sum_{j \in \Scal \sm \cBs(r)}N_j}}\eps^2} \tagcmt{use $\eps \ge \eps_0$}\\
    \stackrel{}{\le}\,& \sum_{r \in \cR} \sum_{k=1}^{d} \exp\del{-\fr{1}{16}\del{\min_{r \in \cR}\min_{k=1}^{d} \min_{\substack{S: \cBs(r) \subset \Scal \subseteq \cBp(r) \\ \abs{\Scal}=n_*(r)+k }}\fr{\del{\sum_{j \in \Scal}N_j}^2}{\sum_{j \in \Scal \sm \cBs(r)}N_j}}\eps^2}  \\
    \stackrel{}{=}\,& Kd \exp\del{-\fr{1}{16}\del{\min_{r \in \cR}\min_{k=1}^{d} \min_{\substack{S: \cBs(r) \subset \Scal \subseteq \cBp(r) \\ \abs{\Scal}=n_*(r)+k }}\fr{\del{\sum_{j \in \Scal}N_j}^2}{\sum_{j \in \Scal \sm \cBs(r)}N_j}}\eps^2} \\
    \stackrel{}{=}\,& \exp\del{-\fr{1}{16}\del{\min_{r \in \cR}\min_{k=1}^{d} \min_{\substack{S: \cBs(r) \subset \Scal \subseteq \cBp(r) \\ \abs{\Scal}=n_*(r)+k }}\fr{\del{\sum_{j \in \Scal}N_j}^2}{\sum_{j \in \Scal \sm \cBs(r)}N_j}}\eps^2 + \ln(Kd)} \\
    \stackrel{}{\le}\,& \exp\del{-\fr{1}{32}\del{\min_{r \in \cR}\min_{k=1}^{d} \min_{\substack{S: \cBs(r) \subset \Scal \subseteq \cBp(r) \\ \abs{\Scal}=n_*(r)+k }}\fr{\del{\sum_{j \in \Scal}N_j}^2}{\sum_{j \in \Scal \sm \cBs(r)}N_j}}\eps^2 } \tagcmt{use $\eps \ge \eps_0$}
  \end{align*}

  With the above claim, we use Lemma~\ref{lemma401:utility_integral_with_eps} to bound the integral 
  \begin{align*}
    &\int_{0}^{\infty} \PP\del{\fr{1}{\sum_{j \in \cB}N_j} \sum_{i \in \cB \sm \cBs(r)}N_i\del{\muhat_i - \mu_1} > \fr{\eps}{2},\, \hr \in \cR,\, G_1} \difeps \\
    \stackrel{}{\le}\,& q_1\eps_0^2 + q_2\fr{1}{z_1} \\
    \stackrel{}{\le}\,& \del{\sqrt{\displaystyle \max_{r \in \cR} \max_{k=1}^{d(r)} \max_{\substack{S: \cBs(r) \subset \Scal \subseteq \cBp(r) \\ \abs{\Scal}=n_*(r)+k }}\fr{32k\sum_{j \in \Scal \sm \cBs(r)}N_j}{\del{\sum_{j \in \Scal}N_j}^2}\log\del{\fr{ed}{k}}\log\del{K^2}}}^2 + \max_{r \in \cR} \max_{k=1}^{d(r)} \max_{\substack{S: \cBs(r) \subset \Scal \subseteq \cBp(r) \\ \abs{\Scal}=n_*(r)+k }}\fr{32\sum_{j \in \Scal \sm \cBs(r)}N_j}{\del{\sum_{j \in \Scal}N_j}^2} \\
    \stackrel{}{\le}\,& 64\del{\displaystyle \max_{r \in \cR} \max_{k=1}^{d(r)} \max_{\substack{S: \cBs(r) \subset \Scal \subseteq \cBp(r) \\ \abs{\Scal}=n_*(r)+k }}\fr{k\sum_{j \in \Scal \sm \cBs(r)}N_j}{\del{\sum_{j \in \Scal}N_j}^2}\log\del{\fr{ed}{k}}\log\del{K^2}} \tagcmt{use $1 \le \log\del{\fr{ed}{k}}\, \forall k \in [1,d]$ and $1 \le \log(K^2)\, \forall K \ge 2$} \\
    \stackrel{}{\le}\,& 128\del{\displaystyle \max_{r \in \cR} \max_{k=1}^{d(r)} \max_{\substack{S: \cBs(r) \subset \Scal \subseteq \cBp(r) \\ \abs{\Scal}=n_*(r)+k }}\fr{k\sum_{j \in \Scal \sm \cBs(r)}N_j}{\del{\sum_{j \in \Scal}N_j}^2}\log\del{\fr{ed}{k}}\log(K)}.
  \end{align*}

Finally, we combine the first and second integrals
\begin{align*}
  &\int_{0}^{\infty} \PP\del{ \hmuB - \mu_1 > \eps,\, G_1 } \difeps \\
  \stackrel{}{\le}\,& \int_{0}^{\infty} \PP\del{ \fr{1}{\sum_{j \in \cB}N_j}\sum_{i \in \cBs(r)}N_i\del{\muhat_i - \mu_1} > \fr{\eps}{2},\, G_1 } \difeps \\
  &+ \int_{0}^{\infty} \PP\del{ \fr{1}{\sum_{j \in \cB}N_j}\sum_{i \in \cB \sm \cBs(r)}N_i\del{\muhat_i - \mu_1} > \fr{\eps}{2},\, G_1 } \difeps \\
  \stackrel{}{\le}\,& 48\del{\fr{\log(K)}{\min_{r \in \cR}\sum_{j \in \cBs(r)}N_j}} + 128\del{\max_{r \in \cR} \max_{k=1}^{d(r)} \max_{\substack{S: \cBs(r) \subseteq \Scal \subseteq \cBp(r) \\ \abs{\Scal}=n_*(r)+k }}\fr{k\sum_{j \in \Scal \sm \cBs(r)}N_j}{\del{\sum_{j \in \Scal}N_j}^2}\log\del{\fr{ed}{k}}\log(K)}
\end{align*}

\end{proof}

\begin{lemma}\label{lemma_g2b:haver21count2}
  If event $G$ sastisfies $\PP\del{G} \le \fr{2K^2}{K^{2\lambda}}$, then Haver achieves
  \begin{align*}
    \int_{0}^{\infty} \PP\del{ \hmuB - \mu_1 > \eps,\, G } \dif \eps = \fr{3088}{KN_1}\log\del{KS}
  \end{align*}
\end{lemma}

\begin{proof}
  We have
  \begin{align*}
    &\int_{0}^{\infty} \PP\del{ \hmuB - \mu_1 > \eps, G } \difeps \\
    \stackrel{}{\le}\,& \int_{0}^{\infty} \PP\del{\hr =  1,\, \hmuB - \mu_1 > \eps, G } \difeps \\
    &+ \int_{0}^{\infty} \sum_{\substack{i: i \ne 1, \\ \gam_i \le 2\gam_1}}\PP\del{\hr = i,\, \hmuB - \mu_{i} > \eps, G} \difeps \\
    &+ \int_{0}^{\infty} \sum_{\substack{i: i \ne 1, \\ \gam_i > 2\gam_1}}\PP\del{\hr = i,\, \hmuB - \mu_{i} > \eps, G} \difeps
  \end{align*}

  For the first term, we have
  \begin{align*}
    &\PP\del{\hr =  1,\, \hmuB - \mu_1 > \eps, G } \\
    \stackrel{}{\le}\,& \PP\del{\hr =  1,\, \hmuB - \mu_1 > \eps } \\
    \stackrel{}{\le}\,& \exp\del{-\fr{1}{2}N_1\del{\eps - \fr{1}{2}\gam_1}_+^2} \tagcmt{use Lemma~\ref{lemma101.b.1:haver}} 
  \end{align*}
  We also have $\PP\del{G} \le \fr{2K^2}{K^{2\lambda}}$, thus
  \begin{align*}
    \PP\del{\hr =  1,\, \hmuB - \mu_1 > \eps, G } \le \exp\del{-\fr{1}{2}N_1\del{\eps - \gam_1}_+^2} \wedge \fr{2K^2}{K^{2\lambda}}
  \end{align*}
  Let $q_1 = \fr{2K}{K^{\lambda}}$, $q_2 = \fr{2K^2}{K^{2\lambda}}$, $z_1 = \fr{N_1}{16}$, and $\eps_0 = \gam_1$
  We claim that in the regime of $\eps \ge \eps_0$, we have
  \begin{align*}
    \PP\del{\hr =  1,\, \hmuB - \mu_1 > \eps, G } \le q_1\exp\del{-z_1\eps^2}
  \end{align*}
  and in the regime of $\eps < \eps_0$, we have $\PP\del{\hr =  1,\, \hmuB - \mu_1 > \eps, G } \le q_2$

  We prove the claim as follows. In the regime of $\eps \ge \eps_0$, we have 
  \begin{align*}
    &\PP\del{\hr =  1,\, \hmuB - \mu_1 > \eps, G } \\
    \stackrel{}{\le}\,& \exp\del{-\fr{1}{2}N_1\del{\eps - \fr{1}{2}\gam_1}_+^2} \wedge \fr{2K^2}{K^{2\lambda}} \\
    \stackrel{}{\le}\,& \sqrt{\exp\del{-\fr{1}{2}N_1\del{\eps - \fr{1}{2}\gam_1}_+^2} \cdot \fr{2K^2}{K^{2\lambda}}} \\
    \stackrel{}{=}\,& \fr{2K}{K^{\lambda}}\exp\del{-\fr{1}{4}N_1\del{\eps - \fr{1}{2}\gam_1}_+^2} \\
    \stackrel{}{\le}\,& \fr{2K}{K^{\lambda}}\exp\del{-\fr{1}{4}N_1\del{\fr{\eps}{2}}^2} \tagcmt{use $\eps \ge \gam_1$}\\
    \stackrel{}{=}\,& \fr{2K}{K^{\lambda}}\exp\del{-\fr{1}{16}N_1\eps^2} 
  \end{align*}
  In the regime of $\eps < \eps_0$, we have
  \begin{align*}
    &\PP\del{\hr = 1,\, \hmuB - \mu_1 > \eps, G } \\
    \stackrel{}{\le}\,& \exp\del{-\fr{1}{2}N_1\del{\eps - \fr{1}{2}\gam_1}_+^2} \wedge \fr{2K^2}{K^{2\lambda}} \\
    \stackrel{}{\le}\,& \fr{2K^2}{K^{2\lambda}} 
  \end{align*}
  With the above claim, we use Lemma~\ref{lemma401:utility_integral_with_eps} to bound the integral
  \begin{align*}
    &\int_{0}^{\infty}\PP\del{\hr = 1,\, \hmuB - \mu_1 > \eps, G } \difeps \\
    \stackrel{}{\le}\,& q_2\eps_0^2 + q_1\fr{1}{z_1}  \\
    \stackrel{}{=}\,& \fr{2K^2}{K^{2\lambda}}\gam_1^2 + \fr{2K}{K^{\lambda}}\fr{16}{N_1}  \\
    \stackrel{}{=}\,& \fr{2K^2}{K^{2\lambda}}\fr{18}{N_1}\log\del{\del{\fr{KS}{N_1}}^{2\lambda}} + \fr{2K}{K^{\lambda}}\fr{16}{N_1} \tagcmt{use $\gam_i = \sqrt{\fr{18}{N_i}\log\del{\del{\fr{KS}{N_i}}^{2\lambda}}}$} \\
    \stackrel{}{=}\,& \fr{36K^2}{K^{4}N_1}\log\del{\del{\fr{KS}{N_1}}^{4}} + \fr{32K}{K^{2}N_1} \tagcmt{choose $\lambda = 2$} \\
    \stackrel{}{=}\,& \fr{36}{K^{2}N_1}\log\del{\del{\fr{KS}{N_1}}^{4}} + \fr{32}{KN_1}  \\
    \stackrel{}{=}\,& \fr{68}{KN_1}\log\del{\del{\fr{KS}{N_1}}^{4}} \tagcmt{use $1 \le \log\del{\del{\fr{KS}{N_1}}^{4}}$ with $K \ge 2$}  \\
    \stackrel{}{=}\,& \fr{272}{KN_1}\log\del{\fr{KS}{N_1}}
  \end{align*}

  For the second term, we denote 
  \begin{align*}
    h(\eps) = \sum_{\substack{i: i \ne 1, \\ \gam_i \le 2\gam_1}}\PP\del{\hr = i,\, \hmuB - \mu_{i} > \eps, G}
  \end{align*}
  by the probability of interest. We have
  \begin{align*}
    &h(\eps) \\
    \stackrel{}{=}\,& \sum_{\substack{i: i \ne 1, \\ \gam_i \le 2\gam_1}}\PP\del{\hr = i,\, \hmuB - \mu_{i} > \eps, G} \\
    \stackrel{}{\le}\,& \sum_{\substack{i: i \ne 1, \\ \gam_i \le 2\gam_1}}\PP\del{\hr = i,\, \hmuB - \mu_{i} > \eps} \\
    \stackrel{}{\le}\,& \sum_{\substack{i: i \ne 1, \\ \gam_i \le 2\gam_1}} \exp\del{-\fr{1}{2}N_i\del{\eps - \gam_1 + \Delta_i}_+^2} \tagcmt{use Lemma~\ref{lemma101.b.2:haver}} \\
    \stackrel{}{\le}\,& \sum_{\substack{i: i \ne 1, \\ \gam_i \le 2\gam_1}} \exp\del{-\fr{1}{2}N_i\del{\eps - \gam_1}_+^2} \\
    \stackrel{}{\le}\,& K \exp\del{-\fr{1}{2}\min_{\substack{i: i \ne 1, \\ \gam_i \le 2\gam_1}}\del{\eps - \gam_1}_+^2} \\
    \stackrel{}{=}\,& K \exp\del{-\fr{1}{2}N_u\del{\eps - \gam_1}_+^2} 
  \end{align*}
  We also have $\PP\del{G} \le \fr{2K^2}{K^{2\lambda}}$ thus
  \begin{align*}
    &h(\eps) \\
    \stackrel{}{=}\,& \sum_{\substack{i: i \ne 1, \\ \gam_i \le 2\gam_1}}\PP\del{\hr = i,\, \hmuB - \mu_{i} > \eps, G} \\
    \stackrel{}{\le}\,& \sum_{\substack{i: i \ne 1, \\ \gam_i \le 2\gam_1}}\PP\del{G} \\
    \stackrel{}{\le}\,& \sum_{\substack{i: i \ne 1, \\ \gam_i \le 2\gam_1}} \fr{2K^2}{K^{2\lambda}} \tagcmt{use $\PP\del{G} \le \fr{2K^2}{K^{2\lambda}}$} \\
    \stackrel{}{\le}\,& \fr{2K^3}{K^{2\lambda}}  
  \end{align*}
  Let $q_1 = \fr{2K}{K^{\lambda}}$, $q_2 = \fr{2K^3}{K^{2\lambda}}$, $z_1 = \fr{N_u}{32}$, and $\eps_0 = 2\gam_1 \vee \sqrt{\fr{32\log(K)}{N_u}}$
  We claim that in the regime of $\eps \ge \eps_0$, we have
  \begin{align*}
    h(\eps) \le q_1\exp\del{-z_1\eps^2}
  \end{align*}
  and in the regime of $\eps < \eps_0$, we have $h(\eps) \le q_2$

  We prove the claim as follows. In the regime of $\eps \ge \eps_0$, we have 
  \begin{align*}
    &h(\eps) \\
    \stackrel{}{\le}\,& K\exp\del{-\fr{1}{2}N_u\del{\eps - \gam_1}_+^2} \wedge \fr{2K^3}{K^{2\lambda}} \\
    \stackrel{}{\le}\,& \sqrt{K\exp\del{-\fr{1}{2}N_u\del{\eps - \gam_1}_+^2} \cdot \fr{2K^3}{K^{2\lambda}}} \\
    \stackrel{}{=}\,& \exp\del{-\fr{1}{4}N_u\del{\eps - \gam_1}_+^2} \\
    \stackrel{}{\le}\,& \fr{2K^2}{K^{\lambda}}\exp\del{-\fr{1}{4}N_u\del{\fr{\eps}{2}}^2} \tagcmt{use $\eps \ge \eps_0 = 2\gam_1$}\\
    \stackrel{}{=}\,& \fr{2K^2}{K^{\lambda}}\exp\del{-\fr{1}{16}N_u\eps^2} \\
    \stackrel{}{=}\,& \fr{2K}{K^{\lambda}}\exp\del{-\fr{1}{16}N_u\eps^2 + \log(K)} \\
    \stackrel{}{\le}\,& \fr{2K}{K^{\lambda}}\exp\del{-\fr{1}{32}N_u\eps^2} \tagcmt{use $\eps \ge \eps_0 \ge \sqrt{\fr{32\log(K)}{N_u}}$} 
  \end{align*}
  In the regime of $\eps < \eps_0$, we have
  \begin{align*}
    &h(\eps) \\
    \stackrel{}{\le}\,& \exp\del{-\fr{1}{2}N_u\del{\eps - \gam_1}_+^2} \wedge \fr{2K^3}{K^{2\lambda}} \\
    \stackrel{}{\le}\,& \fr{2K^3}{K^{2\lambda}} 
  \end{align*}
  With the above claim, we use Lemma~\ref{lemma401:utility_integral_with_eps} to bound the integral
  \begin{align*}
    &\int_{0}^{\infty}h(\eps) \difeps \\
    \stackrel{}{\le}\,& q_2\eps_0^2 + q_1\fr{1}{z_1}  \\
    \stackrel{}{=}\,& \fr{2K^3}{K^{2\lambda}}\del{2\gam_1 \vee \sqrt{\fr{32\log(K)}{N_u}}}^2 + \fr{2K}{K^{\lambda}}\fr{32}{N_u} \\
    \stackrel{}{\le}\,& \gam_1^2 + \fr{8K^3}{K^{2\lambda}}\fr{32\log(K)}{N_u} + \fr{2K}{K^{\lambda}}\fr{32}{N_u}  \\
    \stackrel{}{=}\,& \fr{8K^3}{K^{2\lambda}}\fr{18}{N_1}\log\del{\del{\fr{KS}{N_1}}^{2\lambda}} + \fr{8K^3}{K^{2\lambda}}\fr{32\log(K)}{N_u} + \fr{2K}{K^{\lambda}}\fr{32}{N_u} \tagcmt{use $\gam_i = \sqrt{\fr{18}{N_i}\log\del{\del{\fr{KS}{N_i}}^{2\lambda}}}$} \\
    \stackrel{}{=}\,& \fr{144K^3}{K^{4}N_1}\log\del{\del{\fr{KS}{N_1}}^{4}} + \fr{256K^3\log(K)}{K^{4}N_u} + \fr{64K}{K^{2}N_u} \tagcmt{choose $\lambda = 2$} \\
    \stackrel{}{=}\,& \fr{144}{KN_1}\log\del{\del{\fr{KS}{N_1}}^{4}} + \fr{128\log(K^2)}{KN_u} + \fr{64}{KN_u} \\
    \stackrel{}{\le}\,& \fr{144}{KN_1}\log\del{\del{\fr{KS}{N_1}}^{4}} + \fr{192\log(K^2)}{KN_u} \tagcmt{use $1 \le \log(K^2)$ with $K \ge 2$} \\
    \stackrel{}{\le}\,& \fr{144}{KN_1}\log\del{\del{\fr{KS}{N_1}}^{4}} + \fr{384\log(K)}{KN_u} 
  \end{align*}

  Lemma~\ref{lemma:maxlcb_101} states that for any $i \ne 1$ the condition $\gam_i < 2\gam_1$ implies that $N_i > \fr{N_1}{4} \fr{\log\del{K}}{\log\del{\fr{KS}{N_1}}}$. Thus, $N_u \ge \fr{N_1}{4} \fr{\log\del{K}}{\log\del{\fr{KS}{N_1}}}$.
  \begin{align*}
    &\fr{144}{KN_1}\log\del{\del{\fr{KS}{N_1}}^{4}} + \fr{384\log(K)}{KN_u} \\
    \stackrel{}{\le}\,& \fr{144}{KN_1}\log\del{\del{\fr{KS}{N_1}}^{4}} + \fr{384\log(K)}{KN_1}\fr{4\log\del{\fr{KS}{N_1}}}{\log\del{K}} \\
    \stackrel{}{=}\,& \fr{144}{KN_1}\log\del{\del{\fr{KS}{N_1}}^{4}} + \fr{1436}{KN_1}\log\del{\fr{KS}{N_1}} \\
    \stackrel{}{=}\,& \fr{2112}{KN_1}\log\del{\fr{KS}{N_1}} 
  \end{align*}

  For the third term, we focus on arm $i$ such that $i \ne 1,\, \gam_i > 2\gam_1$. We have 
  \begin{align*}
    &\PP\del{\hr = i, \hmuB - \mu_{i} > \eps, G} \\
    \stackrel{}{\le}\,& \PP\del{\hr = i, \hmuB - \mu_{i} > \eps} \\
    \stackrel{}{\le}\,& \PP\del{\hr = i, \hmu_{i} - \mu_{i} > \eps - \fr{1}{2}\gam_{i} + \Delta_{i}} \tagcmt{use Lemma~\ref{lemma100.b:haver21count2}} \\
    \stackrel{}{\le}\,& \exp\del{-\fr{1}{2}N_i\del{\eps - \gam_i + \Delta_i}_+^2} 
  \end{align*}
  Lemma~\ref{lemma109:haver} states that
  \begin{align*}
    \PP\del{\hr = i,\, \hmu_{\hr} - \gam_{\hr} > \hmu_1 - \gam_1 } \le \del{\fr{N_i}{KS}}^{2\lambda} 
  \end{align*}
  We also have 
  \begin{align*}
    &\PP\del{\hr = i, \hmuB - \mu_{i} > \eps, G} \\
    \stackrel{}{\le}\,& \PP\del{G} \\
    \stackrel{}{\le}\,& \fr{2K^2}{K^{2\lambda}} 
  \end{align*}
  Thus, we have
  \begin{align*}
    &\PP\del{\hr = i, \hmuB - \mu_{i} > \eps, G} \\
    \stackrel{}{\le}\,& \exp\del{-\fr{1}{2}N_i\del{\eps - \gam_i + \Delta_i}_+^2} \wedge \del{\fr{N_i}{KS}}^{2\lambda} \wedge \fr{2K^2}{K^{2\lambda}} 
  \end{align*}

  Let $q_1 = \fr{2K}{K^{\lambda}}\del{\fr{N_i}{KS}}^{\lambda}$, $q_2 = \fr{2K}{K^{\lambda}}\del{\fr{N_i}{KS}}^{\lambda}$, $z_1 = \fr{N_i}{16}$, and $\eps_0 = 2\gam_i$
  We claim that in the regime of $\eps \ge \eps_0$, we have
  \begin{align*}
    \PP\del{\hr = i, \hmuB - \mu_{i} > \eps, G} \le q_1\exp\del{-z_1\eps^2}
  \end{align*}
  and in the regime of $\eps < \eps_0$, we have $h(\eps) \le q_2$

  We prove the claim as follows. In the regime of $\eps \ge \eps_0$, we have 
  \begin{align*}
    &\PP\del{\hr = i, \hmuB - \mu_{i} > \eps, G} \\
    \stackrel{}{\le}\,& \exp\del{-\fr{1}{2}N_i\del{\eps - \gam_i}_+^2} \wedge \del{\fr{N_i}{KS}}^{2\lambda} \wedge \fr{2K^2}{K^{2\lambda}} \\
    \stackrel{}{\le}\,& \sqrt{\exp\del{-\fr{1}{2}N_i\del{\eps - \gam_i}_+^2} \cdot \del{\fr{N_i}{KS}}^{2\lambda} \cdot \fr{2K^2}{K^{2\lambda}}} \\
    \stackrel{}{\le}\,& \del{\fr{N_i}{KS}}^{\lambda}\fr{2K}{K^{\lambda}}\exp\del{-\fr{1}{4}N_i\del{\eps - \gam_i}_+^2} \\
    \stackrel{}{\le}\,& \fr{2K}{K^{\lambda}}\del{\fr{N_i}{KS}}^{\lambda}\exp\del{-\fr{1}{16}N_i\eps^2} \tagcmt{use $\eps \ge eps_0 = 2\gam_i$}
  \end{align*}

  In the regime of $\eps < \eps_0$, we have 
  \begin{align*}
    &\PP\del{\hr = i, \hmuB - \mu_{i} > \eps, G} \\
    \stackrel{}{\le}\,& \del{\fr{N_i}{KS}}^{2\lambda} \wedge \fr{2K^2}{K^{2\lambda}} \\
    \stackrel{}{\le}\,& \sqrt{\del{\fr{N_i}{KS}}^{2\lambda} \cdot \fr{2K^2}{K^{2\lambda}}} \\
    \stackrel{}{\le}\,& \fr{2K}{K^{\lambda}} \del{\fr{N_i}{KS}}^{\lambda} 
  \end{align*}
  With the claim above, we use Lemma~\ref{lemma401:utility_integral_with_eps} to bound the integral
  \begin{align*}
    &\int_{0}^{\infty} \PP\del{\hr = i,\, \hmuB - \mu_1 > \eps, G} \difeps \\
    \stackrel{}{\le}\,& q_2\eps_0^2 + q_1\fr{1}{z_1} \\
    \stackrel{}{\le}\,& \fr{2K}{K^{\lambda}}\del{\fr{N_i}{KS}}^{\lambda}4\gam_i^2 + \fr{2K}{K^{\lambda}}\del{\fr{N_i}{KS}}^{\lambda}\fr{16}{N_i} \\
    \stackrel{}{\le}\,& \fr{8K}{K^{\lambda}}\del{\fr{N_i}{KS}}^{\lambda}\fr{18}{N_i}\log\del{\del{\fr{KS}{N_i}}^{2\lambda}} + \fr{2K}{K^{\lambda}}\del{\fr{N_i}{KS}}^{\lambda}\fr{16}{N_i} \\
    \stackrel{}{=}\,& \fr{8K}{K^{\lambda}}\del{\fr{N_i}{K\Nmax\sum_{j \in [K]}N_j}}^{\lambda}\fr{18}{N_i}\log\del{\del{\fr{KS}{N_i}}^{2\lambda}} + \fr{2K}{K^{\lambda}}\del{\fr{N_i}{K\Nmax\sum_{j \in [K]}N_j}}^{\lambda}\fr{16}{N_i} \tagcmt{use $S = \Nmax\sum_{j \in [K]}N_j$} \\
    \stackrel{}{\le}\,& \fr{144K}{K^{\lambda}N_i}\del{\fr{1}{K\sum_{j \in [K]}N_j}}^{\lambda}\log\del{\del{\fr{KS}{N_i}}^{2\lambda}} + \fr{32K}{K^{\lambda}N_i}\del{\fr{1}{K\sum_{j \in [K]}N_j}}^{\lambda} \\
    \stackrel{}{=}\,& \fr{144K}{K^{2}N_i}\del{\fr{1}{K\sum_{j \in [K]}N_j}}^{2}\log\del{\del{\fr{KS}{N_i}}^{4}} + \fr{32K}{K^{2}N_i}\del{\fr{1}{K\sum_{j \in [K]}N_j}}^{2} \tagcmt{choose $\lambda = 2$} \\
    \stackrel{}{=}\,& \fr{144}{K^3\del{\sum_{j \in [K]}N_j}^2}\log\del{\del{KS}^{4}} + \fr{32}{K^3\del{\sum_{j \in [K]}N_j}^2} \tagcmt{use $N_i \ge 1$} \\
    \stackrel{}{\le}\,& \fr{176}{K^3\del{\sum_{j \in [K]}N_j}^2}\log\del{\del{KS}^{4}} \tagcmt{use $1 \le \log(\del{KS}^4)$ with $K \ge 2$} \\
    \stackrel{}{=}\,& \fr{704}{K^3\del{\sum_{j \in [K]}N_j}^2}\log\del{\del{KS}}
  \end{align*}

  Thus, for the third term, we obtain the integral
  \begin{align*}
    &\sum_{\substack{i: i \ne 1, \\ \gam_i > 2\gam_1}} \int_{0}^{\infty} \PP\del{\hr = i,\, \hmuB - \mu_1 > \eps, G} \difeps \\
    \stackrel{}{\le}\,& \sum_{\substack{i: i \ne 1, \\ \gam_i > 2\gam_1}} \fr{704}{K^3\del{\sum_{j \in [K]}N_j}^2}\log\del{KS} \\
    \stackrel{}{\le}\,& \fr{704}{K^2\del{\sum_{j \in [K]}N_j}^2}\log\del{KS} 
  \end{align*}

  Combining all together, we have
  \begin{align*}
    &\int_{0}^{\infty} \PP\del{ \hmuB - \mu_1 > \eps, G } \difeps \\
    \stackrel{}{\le}\,& \int_{0}^{\infty} \PP\del{\hr =  1,\, \hmuB - \mu_1 > \eps, G } \difeps \\
    &+ \int_{0}^{\infty} \sum_{\substack{i: i \ne 1, \\ \gam_i \le 2\gam_1}}\PP\del{\hr = i,\, \hmuB - \mu_{i} > \eps, G} \difeps \\
    &+ \int_{0}^{\infty} \sum_{\substack{i: i \ne 1, \\ \gam_i > 2\gam_1}}\PP\del{\hr = i,\, \hmuB - \mu_{i} > \eps, G} \difeps \\
    \stackrel{}{\le}\,& \fr{272}{KN_1}\log\del{\fr{KS}{N_1}} \\
    &+ \fr{2112}{KN_1}\log\del{\fr{KS}{N_1}} \\
    &+ \fr{704}{K^2\del{\sum_{j \in [K]}N_j}^2}\log\del{KS} \\
    \stackrel{}{\le}\,& \fr{3088}{KN_1}\log\del{KS}
  \end{align*}
  
\end{proof}

\begin{lemma}\label{lemma100.b:haver21count2}
  In Haver, we have
  \begin{align*}
    \hmu_{\hr} - \gam_{\hr} \le \hmuB \le \hmu_{\hr} + \fr{1}{2}\gam_{\hr}
  \end{align*}
\end{lemma}

\begin{proof}
  For the first inequality, by the definition of $\cB$, $\forall i \in \cB,\, \hmu_i \ge \hmu_{\hr} - \gam_{\hr}$, therefore
  \begin{align*}
    &\sum_{i \in \cB} w_i \hmu_i \ge \hmu_{\hr} - \gam_{\hr} \\
    \stackrel{}{\Leftrightarrow}\,& \hmuB \ge \hmu_{\hr} - \gam_{\hr}
  \end{align*}

  For the second inequality, by the definition of $\hr$, $\forall i \in \cB,\, \hmu_{\hr} - \gam_{\hr} \ge \hmu_i - \gam_i$, therefore $\forall i \in \cB$,
  \begin{align*}
    &\hmu_i \le \hmu_{\hr} - \gam_{\hr} + \gam_i \\
    \stackrel{}{\Rightarrow}\,& \hmu_i \le \hmu_{\hr} - \gam_{\hr} + \fgam \gam_{\hr}  \tagcmt{use $\forall i \in \cB,\, \gam_i  \le \fgam \gam_{\hr}$} \\
    \stackrel{}{\Leftrightarrow}\,& \hmu_i \le \hmu_{\hr} + \fr{1}{2} \gam_{\hr} \\
    \stackrel{}{\Leftrightarrow}\,& \sum_{i \in \cB} w_i \hmu_i \le \hmu_{\hr} + \fr{1}{2} \gam_{\hr} \\
    \stackrel{}{\Leftrightarrow}\,& \hmuB \le \hmu_{\hr} + \fr{1}{2} \gam_{\hr} 
  \end{align*}
  
\end{proof}

\begin{lemma}\label{lemma101.b.1:haver}
  In Haver, we have
  \begin{align*}
    \PP\del{\hr = 1,\, \hmuB - \mu_1 > \eps } \le \exp\del{-\fr{1}{2}N_1\del{\eps - \fr{1}{2}\gam_1}_+^2}
  \end{align*}
\end{lemma}

\begin{proof}
  We have
  \begin{align*}
    &\PP\del{\hr =  1,\, \hmuB - \mu_1 > \eps } \\
    \stackrel{}{\le}\,& \PP\del{\hr =  1,\, \hmu_{\hr} + \fr{1}{2}\gam_{\hr} - \mu_1 > \eps} \tagcmt{use Lemma~\ref{lemma100.b:haver21count2}, $\hmuB \le \hmu_{\hr} + \fr{1}{2}\gam_{\hr}$} \\
    \stackrel{}{=}\,& \PP\del{\hr =  1,\, \hmu_{1} - \mu_1 > \eps - \fr{1}{2}\gam_1} \\
    \stackrel{}{\le}\,& \exp\del{-\fr{1}{2}N_1\del{\eps - \fr{1}{2}\gam_1}_+^2}
  \end{align*}
\end{proof}

\begin{lemma}\label{lemma101.b.2:haver}
  Let $i \in [K]$ be any arm such that $i \ne 1,\, \gam_i \le 2\gam_1$. In Haver, we have
  \begin{align*}
    \PP\del{\hr = i,\, \hmuB - \mu_1 > \eps } \le \exp\del{-\fr{1}{2}N_i\del{\eps - \gam_1 + \Delta_i}_+^2}
  \end{align*}
\end{lemma}

\begin{proof}
  We have
  \begin{align*}
    &\PP\del{\hr = i,\, \hmuB - \mu_{1} > \eps} \\
    \stackrel{}{\le}\,& \PP\del{\hr = i,\, \hmu_{\hr} + \fr{1}{2}\gam_{\hr} - \mu_{1} > \eps} \tagcmt{use Lemma~\ref{lemma100.b:haver21count2}, $\hmuB \le \hmu_{\hr} + \fr{1}{2}\gam_{\hr}$} \\
    \stackrel{}{=}\,& \PP\del{\hr = i,\, \hmu_{i} + \fr{1}{2}\gam_{i} - \mu_{1} > \eps } \\
    \stackrel{}{=}\,& \PP\del{\hr = i,\, \hmu_{i} - \mu_{1} > \eps - \fr{1}{2}\gam_{i}} \\
    \stackrel{}{\le}\,& \PP\del{\hr = i,\, \hmu_{i} - \mu_{i} > \eps - \fr{1}{2}\gam_{i} + \Delta_{i}} \\
    \stackrel{}{\le}\,& \PP\del{\hr = i,\, \hmu_{i} - \mu_{i} > \eps - \gam_{1} + \Delta_{i}} \tagcmt{use  $\gam_i \le 2\gam_1$} \\
    \stackrel{}{\le}\,& \exp\del{-\fr{1}{2}N_i\del{\eps - \gam_1 + \Delta_i}_+^2} 
  \end{align*}
\end{proof}

\begin{lemma}\label{lemma101.b.3:haver}
  Let $i \in [K]$ be any arm such that $i \ne 1,\, \gam_i > 2\gam_1$. In Haver, we have 
  \begin{align*}
    \PP\del{\hr = i,\, \hmuB - \mu_1 > \eps } \le \exp\del{-\fr{1}{2}N_i\del{\eps - \gam_i + \Delta_i}_+^2}
  \end{align*}
\end{lemma}

\begin{proof}
  We have 
  \begin{align*}
    &\PP\del{\hr = i, \hmuB - \mu_{1} > \eps} \\
    \stackrel{}{\le}\,& \PP\del{\hr = i,\, \hmu_{\hr} + \fr{1}{2}\gam_{\hr} - \mu_{1} > \eps} \tagcmt{use Lemma~\ref{lemma100.b:haver21count2}, $\hmuB \le \hmu_{\hr} + \fr{1}{2}\gam_{\hr}$} \\
    \stackrel{}{=}\,& \PP\del{\hr = i,\, \hmu_{i} + \fr{1}{2}\gam_{i} - \mu_{1} > \eps} \\
    \stackrel{}{=}\,& \PP\del{\hr = i,\, \hmu_{i} - \mu_{1} > \eps - \fr{1}{2}\gam_{i} } \\
    \stackrel{}{=}\,& \PP\del{\hr = i,\, \hmu_{i} - \mu_{i} > \eps - \fr{1}{2}\gam_{i} + \Delta_i } \\
    \stackrel{}{\le}\,& \exp\del{-\fr{1}{2}N_i\del{\eps - \fr{1}{2}\gam_i + \Delta_i}_+^2} \\
    \stackrel{}{\le}\,& \exp\del{-\fr{1}{2}N_i\del{\eps - \gam_i + \Delta_i}_+^2} 
  \end{align*}
\end{proof}

\begin{lemma}\label{lemma102.b:haver21count2}
  In Haver, we have
  \begin{align*}
    \int_{0}^{\infty} \PP\del{ \hmuB - \mu_1 > \eps } \difeps \le \fr{720}{N_1}\log\del{KS}
  \end{align*}
\end{lemma}

\begin{proof}
  We have
  \begin{align*}
    &\int_{0}^{\infty} \PP\del{ \hmuB - \mu_1 > \eps } \difeps \\
    \stackrel{}{\le}\,& \int_{0}^{\infty} \PP\del{\hr =  1,\, \hmuB - \mu_1 > \eps } \difeps \\
    &+ \int_{0}^{\infty} \sum_{\substack{i: i \ne 1, \\ \gam_i \le 2\gam_1}}\PP\del{\hr = i,\, \hmuB - \mu_{i} > \eps, G} \difeps \\
    &+ \int_{0}^{\infty} \sum_{\substack{i: i \ne 1, \\ \gam_i > 2\gam_1}}\PP\del{\hr = i,\, \hmuB - \mu_{i} > \eps, G} \difeps
  \end{align*}

  For the first term, from Lemma~\ref{lemma101.b.1:haver}, we have
  \begin{align*}
    &\PP\del{\hr =  1,\, \hmuB - \mu_1 > \eps } \\
    \stackrel{}{\le}\,& \exp\del{-\fr{1}{2}N_1\del{\eps - \fr{1}{2}\gam_1}_+^2} 
  \end{align*}
  Let $q_1 = q_2 = 1$, $z_1 = \fr{N_1}{8}$, and $\eps_0 = \gam_1$
  We claim that in the regime of $\eps \ge \eps_0$, we have
  \begin{align*}
    \PP\del{\hr =  1,\, \hmuB - \mu_1 > \eps} \le q_1\exp\del{-z_1\eps^2}
  \end{align*}
  and in the regime of $\eps < \eps_0$, we have $\PP\del{\hr =  1,\, \hmuB - \mu_1 > \eps, G } \le q_2$

  We prove the claim as follows. In the regime of $\eps \ge \eps_0$, we have 
  \begin{align*}
    &\PP\del{\hr =  1,\, \hmuB - \mu_1 > \eps} \\
    \stackrel{}{\le}\,& \exp\del{-\fr{1}{2}N_1\del{\eps - \fr{1}{2}\gam_1}_+^2} \\
    \stackrel{}{\le}\,& \exp\del{-\fr{1}{2}N_1\del{\fr{\eps}{2}}^2} \tagcmt{use $\eps \ge \eps_0 = \gam_1$}\\
    \stackrel{}{=}\,& \exp\del{-\fr{1}{8}N_1\eps^2} 
  \end{align*}
  In the regime of $\eps < \eps_0$, we have $\PP\del{\hr = 1,\, \hmuB - \mu_1 > \eps} \le 1$
 
  With the above claim, we use Lemma~\ref{lemma401:utility_integral_with_eps} to bound the integral
  \begin{align*}
    &\int_{0}^{\infty}\PP\del{\hr = 1,\, \hmuB - \mu_1 > \eps} \difeps \\
    \stackrel{}{\le}\,& q_2\eps_0^2 + q_1\fr{1}{z_1}  \\
    \stackrel{}{=}\,& \gam_1^2 + \fr{16}{N_1}  \\
    \stackrel{}{=}\,& \fr{18}{N_1}\log\del{\del{\fr{KS}{N_1}}^{2\lambda}} + \fr{8}{N_1} \tagcmt{use $\gam_i = \sqrt{\fr{18}{N_i}\log\del{\del{\fr{KS}{N_i}}^{2\lambda}}}$} \\
    \stackrel{}{=}\,& \fr{18}{N_1}\log\del{\del{\fr{KS}{N_1}}^{4}} + \fr{8}{N_1} \tagcmt{choose $\lambda = 2$} \\
    \stackrel{}{=}\,& \fr{26}{N_1}\log\del{\del{\fr{KS}{N_1}}^{4}} \tagcmt{use $1 \le \log\del{\del{\fr{KS}{N_1}}^{4}}$ with $K \ge 2$}  \\
    \stackrel{}{=}\,& \fr{104}{N_1}\log\del{\fr{KS}{N_1}}
  \end{align*}

  For the second term, we denote 
  \begin{align*}
    h(\eps) = \sum_{\substack{i: i \ne 1, \\ \gam_i \le 2\gam_1}}\PP\del{\hr = i,\, \hmuB - \mu_{i} > \eps}
  \end{align*}
  by the probability of interest. We have
  \begin{align*}
    &h(\eps) \\
    \stackrel{}{=}\,& \sum_{\substack{i: i \ne 1, \\ \gam_i \le 2\gam_1}}\PP\del{\hr = i,\, \hmuB - \mu_{i} > \eps} \\
    \stackrel{}{\le}\,& \sum_{\substack{i: i \ne 1, \\ \gam_i \le 2\gam_1}} \exp\del{-\fr{1}{2}N_i\del{\eps - \gam_1 + \Delta_i}_+^2} \tagcmt{use Lemma~\ref{lemma101.b.2:haver}} \\
    \stackrel{}{\le}\,& \sum_{\substack{i: i \ne 1, \\ \gam_i \le 2\gam_1}} \exp\del{-\fr{1}{2}N_i\del{\eps - \gam_1}_+^2} \\
    \stackrel{}{\le}\,& K \exp\del{-\fr{1}{2}\min_{\substack{i: i \ne 1, \\ \gam_i \le 2\gam_1}}\del{\eps - \gam_1}_+^2} \\
    \stackrel{}{=}\,& K \exp\del{-\fr{1}{2}N_u\del{\eps - \gam_1}_+^2} 
  \end{align*}
  Let $q_1 = q_2 = 1$, $z_1 = \fr{N_u}{16}$, and $\eps_0 = 2\gam_1 \vee \sqrt{\fr{16\log(K)}{N_u}}$.
  We claim that in the regime of $\eps \ge \eps_0$, we have
  \begin{align*}
    h(\eps) \le q_1\exp\del{-z_1\eps^2}
  \end{align*}
  and in the regime of $\eps < \eps_0$, we have $h(\eps) \le q_2$

  We prove the claim as follows. In the regime of $\eps \ge \eps_0$, we have 
  \begin{align*}
    &h(\eps) \\
    \stackrel{}{=}\,& \exp\del{-\fr{1}{2}N_u\del{\eps - \gam_1}_+^2} \\
    \stackrel{}{\le}\,& \exp\del{-\fr{1}{2}N_u\del{\fr{\eps}{2}}^2} \tagcmt{use $\eps \ge \eps_0 = 2\gam_1$}\\
    \stackrel{}{=}\,& \exp\del{-\fr{1}{8}N_u\eps^2} \\
    \stackrel{}{=}\,& \exp\del{-\fr{1}{8}N_u\eps^2 + \log(K)} \\
    \stackrel{}{\le}\,& \exp\del{-\fr{1}{16}N_u\eps^2} \tagcmt{use $\eps \ge \eps_0 \ge \sqrt{\fr{16\log(K)}{N_u}}$} 
  \end{align*}
  In the regime of $\eps < \eps_0$, since $h(\eps)$ is a probability function, we have $h(\eps) \le 1$
  
  With the above claim, we use Lemma~\ref{lemma401:utility_integral_with_eps} to bound the integral
  \begin{align*}
    &\int_{0}^{\infty}h(\eps) \difeps \\
    \stackrel{}{\le}\,& q_2\eps_0^2 + q_1\fr{1}{z_1}  \\
    \stackrel{}{=}\,& \del{2\gam_1 \vee \sqrt{\fr{16\log(K)}{N_u}}}^2 + \fr{16}{N_u} \\
    \stackrel{}{\le}\,& 4\gam_1^2 + \fr{16\log(K)}{N_u} + \fr{16}{N_u}  \\
    \stackrel{}{=}\,& 4\fr{18}{N_1}\log\del{\del{\fr{KS}{N_1}}^{2\lambda}} + \fr{16\log(K)}{N_u} + \fr{16}{N_u} \tagcmt{use $\gam_i = \sqrt{\fr{18}{N_i}\log\del{\del{\fr{KS}{N_i}}^{2\lambda}}}$} \\
    \stackrel{}{=}\,& \fr{72}{N_1}\log\del{\del{\fr{KS}{N_1}}^{4}} + \fr{16\log(K)}{N_u} + \fr{16}{N_u} \tagcmt{choose $\lambda = 2$} \\
    \stackrel{}{=}\,& \fr{72}{N_1}\log\del{\del{\fr{KS}{N_1}}^{4}} + \fr{8\log(K^2)}{N_u} + \fr{16}{N_u} \\
    \stackrel{}{\le}\,& \fr{72}{N_1}\log\del{\del{\fr{KS}{N_1}}^{4}} + \fr{24\log(K^2)}{N_u} \tagcmt{use $1 \le \log(K^2)$ with $K \ge 2$}\\
    \stackrel{}{=}\,& \fr{72}{N_1}\log\del{\del{\fr{KS}{N_1}}^{4}} + \fr{48\log(K)}{N_u} 
  \end{align*}

  Lemma~\ref{lemma:maxlcb_101} states that for any $i \ne 1$ the condition $\gam_i < 2\gam_1$ implies that $N_i > \fr{N_1}{4} \fr{\log\del{K}}{\log\del{\fr{KS}{N_1}}}$. Thus, $N_u \ge \fr{N_1}{4} \fr{\log\del{K}}{\log\del{\fr{KS}{N_1}}}$.
  \begin{align*}
    & \fr{72}{N_1}\log\del{\del{\fr{KS}{N_1}}^{4}} + \fr{48\log(K)}{N_u} \\
    \stackrel{}{\le}\,& \fr{72}{N_1}\log\del{\del{\fr{KS}{N_1}}^{4}} + \fr{48\log(K)}{N_1}\fr{4\log\del{\fr{KS}{N_1}}}{\log\del{K}} \\
    \stackrel{}{=}\,& \fr{72}{N_1}\log\del{\del{\fr{KS}{N_1}}^{4}} + \fr{192}{N_1}\log\del{\fr{KS}{N_1}} \\
    \stackrel{}{=}\,& \fr{480}{N_1}\log\del{\fr{KS}{N_1}} 
  \end{align*}

  For the third term, we focus on arm $i \in [K]$ such that $i \ne 1,\, \gam_i > 2\gam_1$. From Lemma~\ref{lemma101.b.3:haver}, we have 
  \begin{align*}
    &\PP\del{\hr = i, \hmuB - \mu_{i} > \eps} \\
    \stackrel{}{\le}\,& \exp\del{-\fr{1}{2}N_i\del{\eps - \gam_i + \Delta_i}_+^2} 
  \end{align*}
  Lemma~\ref{lemma109:haver} states that
  \begin{align*}
    \PP\del{\hr = i,\, \hmu_{\hr} - \gam_{\hr} > \hmu_1 - \gam_1 } \le \del{\fr{N_i}{KS}}^{2\lambda} 
  \end{align*}
  Thus, we have
  \begin{align*}
    &\PP\del{\hr = i, \hmuB - \mu_{i} > \eps} \\
    \stackrel{}{\le}\,& \exp\del{-\fr{1}{2}N_i\del{\eps - \gam_i + \Delta_i}_+^2} \wedge \del{\fr{N_i}{KS}}^{2\lambda} 
  \end{align*}
  Let $q_1 = \del{\fr{N_i}{KS}}^{\lambda}$, $q_2 = \del{\fr{N_i}{KS}}^{2\lambda}$, $z_1 = \fr{N_i}{16}$, and $\eps_0 = 2\gam_i$
  We claim that in the regime of $\eps \ge \eps_0$, we have
  \begin{align*}
    \PP\del{\hr = i, \hmuB - \mu_{i} > \eps} \le q_1\exp\del{-z_1\eps^2}
  \end{align*}
  and in the regime of $\eps < \eps_0$, we have $h(\eps) \le q_2$

  We prove the claim as follows. In the regime of $\eps \ge \eps_0$, we have 
  \begin{align*}
    &\PP\del{\hr = i, \hmuB - \mu_{i} > \eps} \\
    \stackrel{}{\le}\,& \exp\del{-\fr{1}{2}N_i\del{\eps - \gam_i}_+^2} \wedge \del{\fr{N_i}{KS}}^{2\lambda} \\
    \stackrel{}{\le}\,& \sqrt{\exp\del{-\fr{1}{2}N_i\del{\eps - \gam_i}_+^2} \cdot \del{\fr{N_i}{KS}}^{2\lambda}} \\
    \stackrel{}{\le}\,& \del{\fr{N_i}{KS}}^{\lambda}\exp\del{-\fr{1}{4}N_i\del{\eps - \gam_i}_+^2} \\
    \stackrel{}{\le}\,& \del{\fr{N_i}{KS}}^{\lambda}\exp\del{-\fr{1}{8}N_i\eps^2} \tagcmt{use $\eps \ge \eps_0 = 2\gam_i$}
  \end{align*}

  In the regime of $\eps < \eps_0$, we have $\PP\del{\hr = i, \hmuB - \mu_{i} > \eps} \le \del{\fr{N_i}{KS}}^{2\lambda}$
 
  With the above claim, we use Lemma~\ref{lemma401:utility_integral_with_eps} to bound the integral
  \begin{align*}
    &\int_{0}^{\infty} \PP\del{\hr = i,\, \hmuB - \mu_1 > \eps, G} \difeps \\
    \stackrel{}{\le}\,& q_2\eps_0^2 + q_1\fr{1}{z_1} \\
    \stackrel{}{\le}\,& \del{\fr{N_i}{KS}}^{\lambda}4\gam_i^2 + \del{\fr{N_i}{KS}}^{2\lambda}\fr{16}{N_i} \\
    \stackrel{}{\le}\,& \del{\fr{N_i}{KS}}^{\lambda}\fr{18}{N_i}\log\del{\del{\fr{KS}{N_i}}^{2\lambda}} + \del{\fr{N_i}{KS}}^{2\lambda}\fr{16}{N_i} \\
    \stackrel{}{=}\,& \del{\fr{N_i}{K\Nmax\sum_{j \in [K]}N_j}}^{\lambda}\fr{18}{N_i}\log\del{\del{\fr{KS}{N_i}}^{2\lambda}} + \del{\fr{N_i}{K\Nmax\sum_{j \in [K]}N_j}}^{\lambda}\fr{16}{N_i} \tagcmt{use $S = \Nmax\sum_{j \in [K]}N_j$} \\
    \stackrel{}{\le}\,& \fr{18}{N_i}\del{\fr{1}{K\sum_{j \in [K]}N_j}}^{\lambda}\log\del{\del{\fr{KS}{N_i}}^{2\lambda}} + \fr{16}{N_i}\del{\fr{1}{K\sum_{j \in [K]}N_j}}^{\lambda} \tagcmt{use $N_i \le \Nmax$} \\
    \stackrel{}{=}\,& \fr{18}{N_i}\del{\fr{1}{K\sum_{j \in [K]}N_j}}^{2}\log\del{\del{\fr{KS}{N_i}}^{4}} + \fr{16}{N_i}\del{\fr{1}{K\sum_{j \in [K]}N_j}}^{2} \tagcmt{choose $\lambda = 2$} \\
    \stackrel{}{=}\,& \fr{18}{K\del{\sum_{j \in [K]}N_j}^2}\log\del{\del{KS}^{4}} + \fr{16}{K\del{\sum_{j \in [K]}N_j}^2} \tagcmt{use $N_i \ge 1$} \\
    \stackrel{}{\le}\,& \fr{34}{K\del{\sum_{j \in [K]}N_j}^2}\log\del{\del{KS}^{4}} \tagcmt{use $1 \le \log(\del{KS}^4)$ with $K \ge 2$} \\
    \stackrel{}{=}\,& \fr{136}{K\del{\sum_{j \in [K]}N_j}^2}\log\del{\del{KS}}
  \end{align*}

  Thus, for the third term, we obtain the integral
  \begin{align*}
    &\sum_{\substack{i: i \ne 1, \\ \gam_i > 2\gam_1}} \int_{0}^{\infty} \PP\del{\hr = i,\, \hmuB - \mu_1 > \eps, G} \difeps \\
    \stackrel{}{\le}\,& \sum_{\substack{i: i \ne 1, \\ \gam_i > 2\gam_1}} \fr{136}{K\del{\sum_{j \in [K]}N_j}^2}\log\del{\del{KS}} \\
    \stackrel{}{\le}\,& \fr{136}{\del{\sum_{j \in [K]}N_j}^2}\log\del{\del{KS}} 
  \end{align*}

  Combining all together, we have
  \begin{align*}
    &\int_{0}^{\infty} \PP\del{ \hmuB - \mu_1 > \eps, G } \difeps \\
    \stackrel{}{\le}\,& \int_{0}^{\infty} \PP\del{\hr =  1,\, \hmuB - \mu_1 > \eps, G } \difeps \\
    &+ \int_{0}^{\infty} \sum_{\substack{i: i \ne 1, \\ \gam_i \le 2\gam_1}}\PP\del{\hr = i,\, \hmuB - \mu_{i} > \eps, G} \difeps \\
    &+ \int_{0}^{\infty} \sum_{\substack{i: i \ne 1, \\ \gam_i > 2\gam_1}}\PP\del{\hr = i,\, \hmuB - \mu_{i} > \eps, G} \difeps \\
    \stackrel{}{\le}\,& \fr{104}{N_1}\log\del{\fr{KS}{N_1}} \\
    &+ \fr{480}{N_1}\log\del{\fr{KS}{N_1}}  \\
    &+ \fr{136}{\del{\sum_{j \in [K]}N_j}^2}\log\del{\del{KS}} \\
    \stackrel{}{\le}\,& \fr{720}{N_1}\log\del{KS}
  \end{align*}

\end{proof}


\subsection{Other Lemmas}

\begin{lemma}\label{lemma_g2:haver21count2}
  In the event of $G_2 = \cbr{\exists i \in \cBs(\hr),\, i \not\in \cB}$, Haver achieves
  \begin{align*}
    \PP\del{G_2} \le \frac{2K^2}{K^{2\lambda}}
  \end{align*}
\end{lemma}

\begin{proof}
  Let $i$ be an arm that satisfies the event $G_2$, i.e., $i \in \cBs(\hr),\, i \not\in \cB$.

  By the definition of $\cB$, $i \not\in \cB$ means either (1) $\del{\hmu_i < \hmu_{\hr} - \gam_{\hr},\, \gam_i \le \fgam \gam_{\hr}}$ or (2) $(\gam_i > f \gam_{\hr})$

  The condition (1) implies that
  \begin{align*}
    &\hmu_i < \hmu_{\hr} - \gam_{\hr} \\
    \stackrel{}{\Leftrightarrow}\,& \hmu_i - \mu_i - \hmu_{\hr} + \mu_{\hr} \le -\gam_{\hr} - \mu_i + \mu_{\hr} \\
    \stackrel{}{\Rightarrow}\,& \hmu_i - \mu_i - \hmu_{\hr} + \mu_{\hr} \le -\gam_{\hr} + \mu_{\hr} - \mu_s + \cstar\gam_s \tagcmt{use $i \in \cBs(\hr),\, \mu_i \ge \mu_s - \cstar\gam_s$} \\
    \stackrel{}{\Rightarrow}\,& \hmu_i - \mu_i - \hmu_{\hr} + \mu_{\hr} \le -\gam_{\hr}  + \cstar\gam_s - \cs\gam_s + \cs\gam_{\hr} \tagcmt{by def of $s$, $\mu_s - \cs\gam_s \ge \mu_{\hr} - \cs\gam_{\hr}$}\\
    % \stackrel{}{\Leftrightarrow}\,& \hmu_i - \mu_i - \hmu_{\hr} + \mu_{\hr} \le -(1 - \cs)\gam_{\hr} - (\cs - \cstar)\gam_s \\
    \stackrel{}{\Leftrightarrow}\,& \hmu_i - \mu_i - \hmu_{\hr} + \mu_{\hr} \le -\fr{5}{6}\gam_{\hr} 
  \end{align*}
  Thus, we have
  \begin{align*}
    % & \PP\del{ \exists i \in \cBs(\hr),\, i \not\in \cB,\, \hmu_{i} - \mu_{i} + \mu_{\hr} - \hmu_{\hr} < -\fr{5}{6}\gam_{\hr} - \fr{1}{2}\gam_{s} } \\
    & \PP\del{ \exists i \in \cBs(\hr),\, i \not\in \cB,\, \hmu_{i} - \mu_{i} + \mu_{\hr} - \hmu_{\hr} < -\fr{5}{6}\gam_{\hr} } \\
    \stackrel{}{\le}\,& \sum_{\substack{r \in [K]}} \sum_{i \in \cBs(r)} \PP\del{ \hmu_{i} - \mu_{i} + \mu_{r} - \hmu_{r} < -\fr{5}{6}\gam_{r} } \\
    \stackrel{}{\le}\,& \sum_{\substack{r \in [K]}} \sum_{i \in \cBs(r)} \del{\PP\del{ \mu_{r} - \hmu_{r} < -\fr{1}{3}\gam_{r} } + \PP\del{ \hmu_{i} - \mu_{i}  < -\fr{1}{2}\gam_{r} }} \\
    \stackrel{}{\le}\,& \sum_{\substack{r \in [K]}} \sum_{i \in \cBs(r)} \del{ \exp\del{\frac{-N_{r}\gam_{r}^2}{18}} + \exp\del{\frac{-N_{i}\gam_{r}^2}{8}}} \\
    \stackrel{}{\le}\,& \sum_{\substack{r \in [K]}} \sum_{i \in \cBs(r)} \del{ \exp\del{\frac{-N_{r}\gam_{r}^2}{18}} + \exp\del{\frac{- N_{i}\del{\fgaminv}^{2} \gam_{i}^2}{8}}} \tagcmt{use $i \in \cBs(r),\, \gam_i \le \fgam\gam_{r}$} \\
    \stackrel{}{=}\,& \sum_{\substack{r \in [K]}} \sum_{i \in \cBs(r)} \del{ \exp\del{\frac{-N_{r}\gam_{r}^2}{18}} + \exp\del{\frac{-N_{i}\gam_{i}^2}{18}}} \\
    \stackrel{}{\le}\,& \sum_{\substack{r \in [K]}} \sum_{i \in \cBs(r)}\del{\del{\fr{N_r}{KS}}^{2\lambda} + \del{\fr{N_s}{KS}}^{2\lambda}} \tagcmt{by def $\forall i \in [K],\, \gam_{i} = \sqrt{\frac{18}{N_{i}}\log\del{\del{\fr{KS}{N_i}}^{2\lambda}}}$} \\
    \stackrel{}{\le}\,& \sum_{\substack{r \in [K]}} \sum_{i \in \cBs(r)} \frac{2}{K^{2\lambda}} \tagcmt{use $\forall i,\, N_i \le S$} \\
    \stackrel{}{\le}\,& \frac{2K^2}{K^{2\lambda}} 
  \end{align*}
  
  The condition (2) contradicts with $i \in \cBs(\hr)$ (i.e, $\gam_i \le \fgam \gam_{\hr}$), thus, 
  \begin{align*}
    \PP\del{\exists i \in \cBs(\hr),\, i \not\in \cB,\, \gam_i > f \gam_{\hr}} = 0
  \end{align*}
  Therefore,
  \begin{align*}
    &\PP\del{G_2} \\
    \stackrel{}{\le}\,& \PP\del{ \exists i \in \cBs(\hr),\, i \not\in \cB,\, \hmu_i < \hmu_{\hr} - \gam_{\hr},\, \gam_i \le \fgam \gam_{\hr} } + \PP\del{\exists i \in \cBs(\hr),\, i \not\in \cB,\, \gam_i > \fgam \gam_{\hr}} \\
    \stackrel{}{\le}\,& \fr{2K^2}{K^{2\lambda}}
  \end{align*}
  
\end{proof}

\begin{lemma}\label{lemma_g3:haver21count2}
  In the event of $G_3 = \cbr{\cBs(\hr) \subseteq \cB,\, \exists i \not\in \cBp,\, i \in \cB}$, Haver achieves
  \begin{align*}
    \PP\del{G_3} \le \frac{2K^2}{K^{2\lambda}}
  \end{align*}
\end{lemma}

\begin{proof}
  Let $i$ be an arm that satisfies the event $G_3$, i.e., $i \not\in \cBp(r),\, i \in \cB$.

  By the definition of $\cBp(r)$, $i \not\in \cBp(r)$ means either (1) ($\mu_i < \mu_s - \cplus\gam_s - \cplus\gam_i,\, \gam_i \le \fgam \gam_{\hr}$) or (2) ($\gam_i > \fgam \gam_{\hr}$)
  
  By the definition of $\cB$, since $i \in \cB$, we have $\hmu_i \ge \hmu_{\hr} - \gam_{\hr}$. With the condition (1), we have 
  \begin{align*}
    &\hmu_i \ge \hmu_{\hr} - \gam_{\hr} \\
    \stackrel{}{\Leftrightarrow}\,&  \hmu_i - \hmu_{\hr} \ge - \gam_{\hr} \\
    \stackrel{}{\Rightarrow}\,& \hmu_i - \hmu_s + \gam_{s} - \gam_{\hr} \ge -\gam_{\hr} \tagcmt{by def of $\hr$, $\hmu_{\hr} \ge \hmu_{s} - \gam_{s} + \gam_{\hr}$} \\
    \stackrel{}{\Leftrightarrow}\,& \hmu_i - \hmu_s \ge -\gam_s \\
    \stackrel{}{\Leftrightarrow}\,& \hmu_i - \mu_i + \mu_s - \hmu_s \ge -\gam_s + \mu_s - \mu_i \\
    \stackrel{}{\Rightarrow}\,& \hmu_i - \mu_i + \mu_s - \hmu_s \ge -\gam_s + \cplus\gam_s + \cplus\gam_i \tagcmt{use condition (1)} \\
    % \stackrel{}{\Leftrightarrow}\,& \hmu_i - \mu_i + \mu_s - \hmu_s \ge + (\cplus - 1)\gam_s + \cplus\gam_i \\
    \stackrel{}{\Leftrightarrow}\,& \hmu_i - \mu_i + \mu_s - \hmu_s \ge \fr{1}{3}\gam_s + \fr{4}{3}\gam_i 
  \end{align*}
  Thus, we have
  \begin{align*}
    &\PP\del{G_3} \\
    \stackrel{}{=}\,& \PP\del{\exists i \not\in \cBp,\, i \in \cB,\, \hmu_{i} - \hmu_{\hr} \ge -\gam_{\hr} } \\
    \stackrel{}{\le}\,& \PP\del{\exists i \not\in \cBp,\, i \in \cB,\, \hmu_i - \mu_i + \mu_s - \hmu_s \ge \fr{1}{3}\gam_s + \fr{4}{3}\gam_i} \\
    \stackrel{}{\le}\,& \sum_{i \not\in \cBp} \PP\del{\hmu_i - \mu_i + \mu_s - \hmu_s \ge \fr{1}{3}\gam_s + \fr{4}{3}\gam_i} \\
    \stackrel{}{\le}\,& \sum_{i \not\in \cBp} \del{\PP\del{\mu_s - \hmu_s \ge \fr{1}{3}\gam_s} + \PP\del{\hmu_i - \mu_i \ge \fr{4}{3}\gam_i}} \\
    \stackrel{}{\le}\,& \sum_{i \not\in \cBp}\del{\exp\del{-\fr{N_{s}\gam_{s}^2}{18}} + \exp\del{-\fr{16N_{i}\gam_{i}^2}{18}}} \\
    \stackrel{}{\le}\,& \sum_{i \not\in \cBp}\del{\exp\del{-\fr{N_{s}\gam_{s}^2}{18}} + \exp\del{-\fr{N_{i}\gam_{i}^2}{18}}} \\
    \stackrel{}{=}\,& \sum_{i \not\in \cBp}\del{\del{\fr{N_s}{KS}}^{2\lambda} + \del{\fr{N_i}{KS}}^{2\lambda} } \tagcmt{by def $\forall i \in [K],\, \gam_{i} = \sqrt{\frac{18}{N_{i}}\log\del{\del{\fr{KS}{N_i}}^{2\lambda}}}$} \\
    \stackrel{}{\le}\,& \sum_{i \not\in \cBp} \frac{2}{K^{2\lambda}} \tagcmt{use $\forall i,\, N_i \le S$} \\
    \stackrel{}{\le}\,&\frac{2K^2}{K^{2\lambda}}  
  \end{align*}
  The condition (2) contradicts with $i \in \cB$ (i.e., $\gam_i \le \fgam \gam_{\hr}$), thus,
  \begin{align*}
    \PP\del{\exists i \not\in \cBp,\, i \in \cB,\, \gam_i > \fgam \gam_{\hr}} = 0
  \end{align*}
  Therefore,
  \begin{align*}
    &\PP\del{G_3} \\
    \stackrel{}{\le}\,& \PP\del{\exists i \not\in \cBp,\, i \in \cB,\, \mu_i < \mu_s - \cplus\gam_s - \cplus\gam_i,\, \gam_i \le \fgam \gam_{\hr}} + \PP\del{\exists i \not\in \cBp,\, i \in \cB,\, \gam_i > \fgam \gam_{\hr}} \\
    \stackrel{}{\le}\,& \fr{2K^2}{K^{2\lambda}}
  \end{align*}
\end{proof}

\begin{lemma}\label{lemma109:haver}
  Let any arm $i$ such that $i \ne 1,\, \gam_i > 2\gam_1$, Haver achieves
  \begin{align*}
    \PP\del{\hr = i,\, \hmu_{\hr} - \gam_{\hr} > \hmu_1 - \gam_1 } \le \del{\fr{N_i}{KS}}^{2\lambda}
  \end{align*}
\end{lemma}

\begin{proof}
  By the definition of $\hr$, we have $\hmu_{\hr} - \gam_{\hr} \ge \hmu_1 - \gam_1$. Therefore, with $\hr = i$, we have
  \begin{align*}
    &\PP\del{\hr = i,\, \hmu_{\hr} - \gam_{\hr} \ge \hmu_1 - \gam_1} \\
    \stackrel{}{\le}\,& \PP\del{\hr = i,\, \hmu_i - \mu_i - \hmu_1 + \mu_1 \ge \gam_i - \gam_1 + \Delta_i} \\
    \stackrel{}{\le}\,& \PP\del{\hr = i,\, \hmu_i - \mu_i - \hmu_1 + \mu_1 \ge \fr{1}{2}\gam_i + \Delta_i} \tagcmt{use $\gam_i > 2\gam_1$} \\
    \stackrel{}{\le}\,& \exp\del{-\fr{1}{2}\fr{1}{\del{\fr{1}{N_i} + \fr{1}{N_1}}}\del{\fr{1}{2}\gam_i + \Delta_i}^2} \\
    \stackrel{}{\le}\,& \exp\del{-\fr{1}{8}\fr{1}{\del{\fr{1}{N_i} + \fr{1}{N_1}}}\del{\gam_i + \Delta_i}^2}
  \end{align*}

  Lemma~\ref{lemma:maxlcb_102} states that for any $i \ne 1$ the condition $\gam_i > 2\gam_1$ implies that $N_i < N_1$. Therefore,
  \begin{align*}
    &\exp\del{-\fr{1}{8}\fr{1}{\del{\fr{1}{N_i} + \fr{1}{N_1}}}\del{\gam_i + \Delta_i}^2} \\
    \stackrel{}{\le}\,& \exp\del{-\fr{1}{8}\fr{1}{\del{\fr{1}{N_i} + \fr{1}{N_i}}}\del{\gam_i + \Delta_i}^2} \\
    \stackrel{}{=}\,& \exp\del{-\fr{1}{16}N_i\del{\gam_i + \Delta_i}^2} \\
    \stackrel{}{\le}\,& \exp\del{-\fr{1}{16}N_i\gam_i^2} \tagcmt{use $\Delta_i \ge 1$} \\
    \stackrel{}{\le}\,& \exp\del{-\fr{1}{18}N_i\gam_i^2} \\
    \stackrel{}{=}\,& \del{\fr{N_i}{KS}}^{2\lambda} \tagcmt{use $\gam_i = \sqrt{\fr{18}{N_i}\log\del{\del{\fr{KS}{N_i}}^{2\lambda}}}$} \\
  \end{align*}
  
\end{proof}



\section{General Lemmata}

\begin{lemma}\label{lemma401:utility_integral_with_eps}
  Let $q_1$, $q_2$, $z_1$, and $\eps_0$ be some positive values. Let $f$ be a probability function of $\eps$ such that in the regime of $\eps \ge \eps_0$, we have 
  \begin{align*}
    f(\eps) \le q_1\exp\del{-z_1\eps^2}.
  \end{align*}
  and in the regime of $\eps < \eps_0$, we have $f(\eps) \le q_2$.
  Then, we can bound the integral
  \begin{align*}
    \int_{0}^{\infty} f(\eps) \difeps \le q_2\eps_0^2 + q_1\fr{1}{z_1}.
  \end{align*}
\end{lemma}

\begin{proof}
  We bound the integral as follows
  \begin{align*}
    &\int_{0}^{\infty} f(\eps) \difeps \\
    \stackrel{}{=}\,& \int_{0}^{\eps_0} f(\eps) \difeps + \int_{\eps_0}^{\infty} f(\eps)  \difeps \\
    \stackrel{}{\le}\,& \int_{0}^{\eps_0} f(\eps) \difeps + \int_{\eps_0}^{\infty} q_1\exp\del{-z_1\eps^2} \difeps \tagcmt{in the regime $\eps \ge \eps_0$, use $f(\eps) \le q_1\exp\del{-z_1\eps^2}$} \\
    \stackrel{}{\le}\,& \int_{0}^{\eps_0} q_2\difeps + \int_{\eps_0}^{\infty} q_1\exp\del{-z_1\eps^2} \difeps \tagcmt{in the regime $\eps \le \eps_0$, use $f(\eps) \le q_2$} \\
    \stackrel{}{=}\,& q_2\eps^2 \Big|_{0}^{\eps_0} - \fr{q_1}{z_1}\exp\del{-z_1\eps^2} \Big|_{\eps_0}^{\infty} \\
    \stackrel{}{=}\,& q_2\eps_0^2 + q_1\fr{1}{z_1}\exp\del{-z_1\eps_0^2} \\
    \stackrel{}{\le}\,& q_2\eps_0^2 + q_1\fr{1}{z_1} \tagcmt{use $\exp\del{-z_1\eps_0^2} \le 1$}.
  \end{align*}
  
\end{proof}

\begin{lemma}\label{lemma401:utility_integral_without_eps}
  Let $q_1$ and $z_1$ be some positive values. Let $f$ be a probability function of $\eps$. If we have 
  \begin{align*}
    f(\eps) \le q_1\exp\del{-z_1\eps^2}.
  \end{align*}
  Then, we can bound the integral
  \begin{align*}
    \int_{0}^{\infty} f(\eps) \difeps \le q_1\fr{1}{z_1}.
  \end{align*}
\end{lemma}

\begin{proof}
  We bound the integral as follows
  \begin{align*}
    &\int_{0}^{\infty} f(\eps) \difeps \\
    \stackrel{}{\le}\,& \int_{0}^{\infty} q_1\exp\del{-z_1\eps^2} \difeps \\
    \stackrel{}{=}\,& - q_1\fr{1}{z_1}\exp\del{-z_1\eps^2} \Big|_{0}^{\infty} \\
    \stackrel{}{=}\,& q_1\fr{1}{z_1} 
  \end{align*}
  
\end{proof}


\begin{lemma}\label{lemma200.a:haver21count2}
  With $q^2 \ge \fr{1}{9}$, in Haver, we have
  \begin{align*}
    \int_{0}^{\infty} \PP\del{ \abs{\hmuB - \mu_1} < \eps,\, \exists i \in [K],\, \abs{\hmu_i - \mu_i} \ge q\gam_i} \difeps \le \fr{3792}{KN_1}\log\del{KS}
  \end{align*}
\end{lemma}

\begin{proof}
  We denote $G = \cbr{\exists i \in [K],\, \abs{\hmu_{i} - \mu_i} \ge q \gam_i}$. We have
  \begin{align*}
    &\PP\del{\exists i \in [K],\, \abs{\hmu_{i} - \mu_i} \ge q \gam_i} \\
    \stackrel{}{\le}\,& \sum_{i \in [K]}\PP\del{\abs{\hmu_{i} - \mu_i} \ge q \gam_i} \\
    \stackrel{}{\le}\,& \sum_{i \in [K]}2\exp\del{-\fr{1}{2}N_iq^2\gam_i^2} \\
    \stackrel{}{=}\,& \sum_{i \in [K]}2\exp\del{-\fr{1}{2}N_i q^2 \fr{18}{N_i}\ln\del{\del{\fr{KS}{N_i}}^{2\lam}}} \tagcmt{use $\gam_i = \sqrt{\fr{18}{N_i}\ln\del{\del{\fr{KS}{N_i}}^{2\lam}}}$} \\
    \stackrel{}{\le}\,& \sum_{i \in [K]}2\del{\fr{N_i}{KS}}^{2\lam} \tag{use $q^2 \ge \fr{1}{9} $} \\
    \stackrel{}{\le}\,& \sum_{i \in [K]}2\del{\fr{1}{K}}^{2\lam} \tagcmt{use $\forall i \in [K],\, N_i \le S$} \\
    % \stackrel{}{\le}\,& \fr{2K}{K^{2\lam}} \\
    \stackrel{}{\le}\,& \fr{2K^2}{K^{2\lam}}
  \end{align*}

  Since $G$ satisfies $\PP\del{G} \le \fr{2K^2}{K^{2\lam}}$, we use Lemma~\ref{lemma_g2a:haver21count2} to obtain
  \begin{align*}
    &\int_{0}^{\infty} \PP\del{ \hmuB - \mu_1 > \eps,\, G } \difeps \\
    \stackrel{}{\le}\,& \min_m \del{\fr{704}{K^2N_m}\log\del{\fr{KS}{N_m}}  + \fr{8}{K^{2}}\Delta_m^2} \\
    \stackrel{}{\le}\,& \fr{704}{K^2N_1}\log\del{\fr{KS}{N_1}} \tagcmt{choose $m = 1$}
  \end{align*}

  Also, we use Lemma~\ref{lemma_g2b:haver21count2} to obtain
  \begin{align*}
    \int_{0}^{\infty} \PP\del{ \hmuB - \mu_1 > \eps,\, G } \difeps \le \fr{3088}{KN_1}\log\del{KS}
  \end{align*}
  Therefore,
  \begin{align*}
    &\int_{0}^{\infty} \PP\del{ \abs{\hmuB - \mu_1} < \eps,\, G } \difeps \\
    \stackrel{}{=}\,& \PP\del{ \hmuB - \mu_1 < -\eps,\, G } \difeps \\
    &+ \int_{0}^{\infty} \PP\del{ \hmuB - \mu_1 > \eps,\, G } \difeps \\
    \stackrel{}{\le}\,& \fr{704}{K^2N_1}\log\del{\fr{KS}{N_1}} + \fr{3088}{KN_1}\log\del{KS} \\
    \stackrel{}{\le}\,& \fr{3792}{KN_1}\log\del{KS}
  \end{align*}
    
\end{proof}

\begin{lemma}\label{xlemma:max_bound}
  Let $n,d \ge 1$ be two integers. Then,
  \begin{align*}
    \max_{k=1}^{d(r)} \fr{k^2}{\del{n+k}^2} \le \del{\log\del{\fr{n+d}{n}}}^2
  \end{align*}
\end{lemma}

\begin{proof}
  We have
  \begin{align*}
    &\max_{k=1}^{d(r)} \fr{k^2}{\del{n+k}^2} \\
    \stackrel{}{\le}\,& \del{\max_{k=1}^{d(r)} \fr{k}{\del{n+k}}}^2 \\
    \stackrel{}{\le}\,& \del{\sum_{k=1}^d \fr{1}{\del{n+k}}}^2 \\
  \end{align*}
  Then, we bound the summation term with integral
  \begin{align*}
    &\sum_{k=1}^d \fr{1}{\del{n+k}} \\
    \stackrel{}{\le}\,& \int_{k=0}^d \fr{1}{\del{n+k}} \\
    \stackrel{}{=}\,& \log\del{n+k} \Big|_{0}^{d} \\
    \stackrel{}{=}\,& \log\del{\fr{n+d}{n}}.
  \end{align*}
  Therefore,
  \begin{align*}
    \max_{k=1}^{d(r)} \fr{k^2}{\del{n+k}^2} \le \del{\log\del{\fr{n+d}{n}}}^2.
  \end{align*}
\end{proof}


\begin{lemma}[Stirling's formula]
  \label{xlemma:stirling_formula}
  Let $k, d$ be two positive integers such that $1 \le k \le n$. Then,
  \begin{align*}
    \del{\fr{n}{k}}^k \le \binom{n}{k} \le \del{\fr{en}{k}}^k
  \end{align*}
\end{lemma}

\begin{lemma}[Anti-concentration inequality (cite abramowitz1968handbook)]
  \label{xlemma:anti_concentration_inequality}
  For a Gaussian random variable $X \sim \mathcal{N}(\mu, \sigma^2)$ and any $z > 0$, we have
  \begin{align*}
    \PP\del{\abs{X - \mu} > \eps} > \fr{1}{4\sqrt{\pi}}\ep{-\fr{7\eps^2}{2\sigma^2}}.
  \end{align*}
\end{lemma}

\begin{lemma}\label{lemma301:bcals}
  Consider the Poly($\alpha$) instance where $\forall i \ge 2,\, \Delta_i = \del{\fr{i}{K}}^{\alpha}$. Suppose $\cS = \cbr{i: \Delta_i \le c\sqrt{\frac{1}{N}}}$, then
  \begin{align*}
    \abs{\cS} = \floor{\frac{Kc^{\fr{1}{\alpha}}}{N^{\frac{1}{2\alpha}}} }
  \end{align*}
\end{lemma}

\begin{proof}
  
We have
\begin{align*}
  &\Delta_i \le c\sqrt{\frac{1}{N}} \\
  \stackrel{}{\Leftrightarrow}\,& \del{\frac{i}{K}}^{\alpha} \le c\sqrt{\frac{1}{N}} \\
  \stackrel{}{\Leftrightarrow}\,& \frac{i}{K} \le \frac{c^{\fr{1}{\alpha}}}{N^{\frac{1}{2\alpha}}} \\
  \stackrel{}{\Leftrightarrow}\,& i \le \frac{Kc^{\fr{1}{\alpha}}}{N^{\frac{1}{2\alpha}}}
\end{align*}

Therefore, $\abs{\cS} = \max\cbr{i: \Delta_i \le \fr{1}{c}\sqrt{\fr{1}{N}}} = \floor{\frac{Kc^{\fr{1}{\alpha}}}{N^{\frac{1}{2\alpha}}}} $

\end{proof}

\begin{lemma}\label{lemma302:bcals}
  Consider the Poly($\alpha$) instance where $\forall i \ge 2,\, \Delta_i = \del{\fr{i}{K}}^{\alpha}$. Suppose $\Bcalp = \cbr{i: \Delta_i \le c\sqrt{\frac{1}{N}}}$, then
  \begin{align*}
    \displaystyle \frac{1}{\abs{\Bcalp}}\sum_{i = 1}^{\abs{\Bcalp}}\Delta_i \le \frac{c}{\del{\alpha+1}\sqrt{N}}.
  \end{align*}
\end{lemma}

\begin{proof}
  
We have 
\begin{align*}
  &\frac{1}{\abs{\Bcalp}}\sum_{i = 1}^{\abs{\Bcalp}}\Delta_i \\
  \stackrel{}{=}\,& \frac{1}{\abs{\Bcalp}}\sum_{i = 1}^{\abs{\Bcalp}}\del{\frac{i}{K}}^{\alpha} \\
  \stackrel{}{=}\,& \frac{1}{K^{\alpha}}\frac{1}{\abs{\Bcalp}}\sum_{i = 1}^{\abs{\Bcalp}}i^{\alpha} \\
  \stackrel{}{\le}\,& \frac{1}{K^{\alpha}}\frac{1}{\abs{\Bcalp}}\int_{i = 1}^{\abs{\Bcalp}}i^{\alpha} \\
  \stackrel{}{=}\,& \frac{1}{K^{\alpha}}\frac{1}{\abs{\Bcalp}}\frac{\abs{\Bcalp}^{\alpha+1} - 1}{\alpha+1} \\
  \stackrel{}{\le}\,& \frac{1}{K^{\alpha}}\frac{1}{\abs{\Bcalp}}\frac{\abs{\Bcalp}^{\alpha+1}}{\alpha+1} \\
  \stackrel{}{=}\,& \frac{1}{K^{\alpha}}\frac{\abs{\Bcalp}^{\alpha}}{\alpha+1}.
\end{align*}

From Lemma \ref{lemma301:bcals}, we have $\abs{\Bcalp} = \floor{\frac{Kc^{\fr{1}{\alpha}}}{N^{\frac{1}{2\alpha}}}}  \le \frac{Kc^{\fr{1}{\alpha}}}{N^{\frac{1}{2\alpha}}}$. Therefore,
\begin{align*}
  &\frac{1}{K^{\alpha}}\frac{\abs{\Bcalp}^{\alpha}}{\alpha+1} \\
  \stackrel{}{\le}\,& \frac{1}{K^{\alpha}}\frac{\del{\frac{Kc^{\fr{1}{\alpha}}}{N^{\frac{1}{2\alpha}}}}^{\alpha}}{\alpha+1} \\
  \stackrel{}{=}\,& \frac{c}{\del{\alpha+1}\sqrt{N}}.
\end{align*}

\end{proof}

\begin{lemma}\label{lemma303:bcals}
  Consider the Poly($\alpha$) instance where $\forall i \ge 2,\, \Delta_i = \del{\fr{i}{K}}^{\alpha}$. Suppose $\Bcals = \cbr{i: \Delta_i \le \fr{1}{a_1}\gam}$ and $\Bcalp := \cbr{i: \Delta_i \le a_2\gam}$. Assuming that $N$ is not too large, i.e., $N \le \fr{1}{4a_1^2}\del{K\fr{\ln(2)}{\alpha}}^{2\alpha}$, then
  \begin{align*}
    \fr{1}{\abs{\Bcals}} \le \fr{1}{K\del{\fr{1}{2a_1}\sqrt{\fr{1}{N}}}^{\fr{1}{\alpha}}}
  \end{align*}
  and
  \begin{align*}
    \fr{\abs{\Bcalp}}{\abs{\Bcals}} \le \del{2a_1a_2}^{\fr{1}{\alpha}}.
  \end{align*}
\end{lemma}

\begin{proof}
  From Lemma \ref{lemma301:bcals}, we have $\abs{\Bcalp} = \floor{\frac{Ka_2^{\fr{1}{\alpha}}}{N^{\frac{1}{2\alpha}}}} \le K\del{a_2\sqrt{\fr{1}{N}}}^{\fr{1}{\alpha}}$ and
  $\abs{\Bcals} = \floor{\frac{K\del{\fr{1}{a_1}}^{\fr{1}{\alpha}}}{N^{\frac{1}{2\alpha}}}} \ge K\del{\fr{1}{a_1}\sqrt{\fr{1}{N}}}^{\fr{1}{\alpha}}-1$.

  From the assumption $N \le \fr{1}{4a_1^2}\del{K\fr{\ln(2)}{\alpha}}^{2\alpha}$, we have
\begin{align*}
  \del{\fr{1}{a_1}\sqrt{\fr{1}{N}}}^{\fr{1}{\alpha}} - \fr{1}{K} \ge \del{\fr{1}{2a_1}\sqrt{\fr{1}{N}}}^{\fr{1}{\alpha}}
\end{align*}

Therefore,
\begin{align*}
  \fr{\abs{\Bcalp}}{\abs{\Bcals}}
  \stackrel{}{\le}\,& \fr{K\del{a_2\sqrt{\fr{1}{N}}}^{\fr{1}{\alpha}}}{K\del{\fr{1}{a_1}\sqrt{\fr{1}{N}}}^{\fr{1}{\alpha}}-1} \\
  \stackrel{}{\le}\,& \fr{K\del{a_2\sqrt{\fr{1}{N}}}^{\fr{1}{\alpha}}}{K\del{\fr{1}{2a_1}\sqrt{\fr{1}{N}}}^{\fr{1}{\alpha}}} \\
  \stackrel{}{=}\,& \del{2a_1a_2}^{\fr{1}{\alpha}}.
\end{align*}


% We have
% \begin{align*}
%   &\sum_{k=1}^{\abs{\Bcalp} - \abs{\Bcals}}\fr{1}{\del{\abs{\Bcals}+k}N} \\
%   \stackrel{}{\le}\,&\fr{1}{N}\log\del{\fr{\abs{\Bcalp}}{\abs{\Bcals}}} \tagcmt{todo: more details} \\
%   \stackrel{}{\le}\,&\fr{1}{N}\log\del{2cd^{\fr{1}{\alpha}}} \\
%   \stackrel{}{\le}\,&\fr{1}{\alpha N}.
% \end{align*}

\end{proof}



\begin{lemma}\label{lemma304:bcals}
  Consider the Poly($\alpha$) instance where $\forall i \ge 2,\, \Delta_i = \del{\fr{i}{K}}^{\alpha}$. Suppose $\Bcals = \cbr{i: \Delta_i \le \fr{1}{a_1}\gam}$ and $\Bcalp := \cbr{i: \Delta_i \le a_2\gam}$. Assuming that $N$ is not too large, i.e., $N \le \fr{1}{4a_1^2}\del{K\fr{\ln(2)}{\alpha}}^{2\alpha}$, then
  \begin{align*}
    \frac{1}{\abs{\Bcals}}\sum_{i = 1}^{\abs{\Bcalp}}\Delta_i \le \fr{a_2\del{2a_1a_2}^{\fr{1}{\alpha}}}{\del{\alpha+1}\sqrt{N}}.
  \end{align*}
\end{lemma}

\begin{proof}

We have
\begin{align*}
  &\frac{1}{\abs{\Bcals}}\sum_{i = 1}^{\abs{\Bcalp}}\Delta_i \\
  \stackrel{}{\le}\,& \del{2a_1a_2}^{\fr{1}{\alpha}}\fr{1}{\abs{\Bcalp}}\sum_{i = 1}^{\abs{\Bcalp}}\Delta_i \tagcmt{from Lemma \ref{lemma303:bcals}} \\
  \stackrel{}{\le}\,& \del{2a_1a_2}^{\fr{1}{\alpha}}\fr{a_2}{\del{\alpha+1}\sqrt{N}} \tagcmt{from Lemma \ref{lemma302:bcals}} \\
  \stackrel{}{=}\,& \fr{a_2\del{2a_1a_2}^{\fr{1}{\alpha}}}{\del{\alpha+1}\sqrt{N}}.
\end{align*}

\end{proof}


% \begin{lemma}\label{lemma301:bcals}
%   Consider the Polynomial($\alpha$) instance where $\forall i \ge 2,\, \Delta_i = \del{\fr{i}{K}}^{\alpha}$
%   In the  $\cB = \cbr{i: \Delta_i \le c\sqrt{\frac{1}{N}}}$, where $\Delta_i = \del{\fr{i}{K}}^{\alpha}$. We have
%   \begin{align*}
%     \abs{\cB} = \floor{\frac{Kc^{\fr{1}{\alpha}}}{N^{\frac{1}{2\alpha}}} }
%   \end{align*}
% \end{lemma}

% \textit{Proof}

% We have
% \begin{align*}
%   &\Delta_i \le c\sqrt{\frac{1}{N}} \\
%   \stackrel{}{\Leftrightarrow}\,& \del{\frac{i}{K}}^{\alpha} \le c\sqrt{\frac{1}{N}} \\
%   \stackrel{}{\Leftrightarrow}\,& \frac{i}{K} \le \frac{c^{\fr{1}{\alpha}}}{N^{\frac{1}{2\alpha}}} \\
%   \stackrel{}{\Leftrightarrow}\,& i \le \frac{Kc^{\fr{1}{\alpha}}}{N^{\frac{1}{2\alpha}}}
% \end{align*}

% Therefore, $\abs{\cBs}  = \max\cbr{i: \Delta_i \le \fr{1}{c}\sqrt{\fr{1}{N}}} = \floor*{\frac{Kc^{\fr{1}{\alpha}}}{N^{\frac{1}{2\alpha}}}} $

% \begin{lemma}\label{lemma302:bcals}
%   Suppose $\cBs = \cbr{i: \Delta_i \le c\sqrt{\frac{1}{N}}}$, where $\Delta_i = \del{\fr{i}{K}}^{\alpha}$. We have
%   \begin{align*}
%     \displaystyle \frac{1}{\abs{\cBs}}\sum_{i = 1}^{\abs{\cBs}}\Delta_i \lsim \frac{1}{\del{\alpha+1}\sqrt{N}}
%   \end{align*}
% \end{lemma}

% \textit{Proof}

% We have 
% \begin{align*}
%   &\frac{1}{\abs{\cBs}}\sum_{i = 1}^{\abs{\cBs}}\Delta_i \\
%   \stackrel{}{=}\,& \frac{1}{\abs{\cBs}}\sum_{i = 1}^{\abs{\cBs}}\del{\frac{i}{K}}^{\alpha} \\
%   \stackrel{}{=}\,& \frac{1}{K^{\alpha}}\frac{1}{\abs{\cBs}}\sum_{i = 1}^{\abs{\cBs}}i^{\alpha} \\
%   \stackrel{}{\approx}\,& \frac{1}{K^{\alpha}}\frac{1}{\abs{\cBs}}\int_{i = 1}^{\abs{\cBs}}i^{\alpha} \\
%   \stackrel{}{=}\,& \frac{1}{K^{\alpha}}\frac{1}{\abs{\cBs}}\frac{\abs{\cBs}^{\alpha+1} - 1}{\alpha+1} \\
%   \stackrel{}{\le}\,& \frac{1}{K^{\alpha}}\frac{1}{\abs{\cBs}}\frac{\abs{\cBs}^{\alpha+1}}{\alpha+1} \\
%   \stackrel{}{=}\,& \frac{1}{K^{\alpha}}\frac{\abs{\cBs}^{\alpha}}{\alpha+1} \\
%   \stackrel{}{=}\,& \frac{1}{K^{\alpha}}\frac{\del{\frac{Kc^{\fr{1}{\alpha}}}{N^{\frac{1}{2\alpha}}}}^{\alpha}}{\alpha+1} \\
%   \stackrel{}{=}\,& \frac{c}{\del{\alpha+1}\sqrt{N}} \\
% \end{align*}

% \begin{lemma}\label{lemma303:bcals}
%   Suppose $\cBs = \cbr{i: \Delta_i \le \fr{1}{d}\sqrt{\frac{1}{N}}}$ and $\cBp := \cbr{i: \Delta_i \le c\sqrt{\frac{1}{N}}}$, where $\Delta_i = \del{\fr{i}{K}}^{\alpha}$. Suppose $\abs{\cBs} > 2$, we have
%   \begin{align*}
%     \frac{1}{\abs{\cBs}}\sum_{i = 1}^{\abs{\cBp}}\Delta_i \le \fr{2dc^2}{\del{a+1}\sqrt{N}}
%   \end{align*}
% \end{lemma}

% \textit{Proof}

% We have
% \begin{align*}
%   &\abs{\cBs} > 2 \\
%   \stackrel{}{\Rightarrow}\,&\floor*{K\del{\fr{1}{d}\sqrt{\fr{1}{N}}}^{\fr{1}{\alpha}}} > 2 \\
%   \stackrel{}{\Rightarrow}\,& K\del{\fr{1}{d}\sqrt{\fr{1}{N}}}^{\fr{1}{\alpha}} \ge 2 \\
%   \stackrel{}{\Rightarrow}\,& K\del{\fr{1}{d}\sqrt{\fr{1}{N}}}^{\fr{1}{\alpha}} - 2 \ge \fr{1}{2}K\del{\fr{1}{d}\sqrt{\fr{1}{N}}}^{\fr{1}{\alpha}} \tagcmt{$1$}
% \end{align*}


% We have
% \begin{align*}
%   \fr{\abs{\cBp}}{\abs{\cBs}}
%   \stackrel{}{\le}\,& \fr{K\del{c\sqrt{\fr{1}{N}}}^{\fr{1}{\alpha}}}{K\del{\fr{1}{d}\sqrt{\fr{1}{N}}}^{\fr{1}{\alpha}}-1} \\
%   \stackrel{}{\le}\,& \fr{K\del{c\sqrt{\fr{1}{N}}}^{\fr{1}{\alpha}}}{\fr{1}{2}K\del{\fr{1}{d}\sqrt{\fr{1}{N}}}^{\fr{1}{\alpha}}} \tagcmt{from $(1)$} \\
%   \stackrel{}{=}\,& 2\del{cd}^{\fr{1}{\alpha}} \\
%   \stackrel{}{\le}\,& 2cd \\
% \end{align*}

% Therefore,
% \begin{align*}
%   \frac{1}{\abs{\cBs}}\sum_{i = 1}^{\abs{\cBp}}\Delta_i \\
%   \stackrel{}{\le}\,& \fr{\abs{\cBp}}{\abs{\cBs}}\fr{1}{\abs{\cBp}}\sum_{i = 1}^{\abs{\cBp}}\Delta_i \\
%   \stackrel{}{\le}\,& 2cd\fr{1}{\abs{\cBp}}\sum_{i = 1}^{\abs{\cBp}}\Delta_i \\
%   \stackrel{}{\le}\,& 2cd\fr{c}{\del{\alpha+1}\sqrt{N}} \\
%   \stackrel{}{=}\,& \fr{2dc^2}{\del{\alpha+1}\sqrt{N}} \\
% \end{align*}

% \begin{lemma}\label{lemma304:bcals}
%   Suppose $\cBs = \cbr{i: \Delta_i \le \fr{1}{d}\sqrt{\frac{1}{N}}}$ and $\cBp := \cbr{i: \Delta_i \le c\sqrt{\frac{1}{N}}}$, where $\Delta_i = \del{\fr{i}{K}}^{\alpha}$. Suppose $\abs{\cBs} > 2$, we have
%   \begin{align*}
%     \sum_{k=1}^{\abs{\cBp} - \abs{\cBs}}\fr{1}{\del{\abs{\cBs}+k}N} \le \fr{1}{\alpha N}
%   \end{align*}
% \end{lemma}

% We have
% \begin{align*}
%   &\sum_{k=1}^{\abs{\cBp} - \abs{\cBs}}\fr{1}{\del{\abs{\cBs}+k}N} \\
%   \stackrel{}{\le}\,&\fr{1}{N}\log\del{\fr{\abs{\cBp}}{\abs{\cBs}}} \tagcmt{todo: more details} \\
%   \stackrel{}{\le}\,&\fr{1}{N}\log\del{2cd^{\fr{1}{\alpha}}} \\
%   \stackrel{}{\le}\,&\fr{1}{\alpha N} \\
% \end{align*}



\section{Theorems for the MaxLCB Estimator}
\label{thm_proof:maxlcb}

\newtheorem*{thm-2}{Theorem ~\ref{thm:maxlcb}}
\begin{thm-2}
  MaxLCB achieves
  \begin{align*}
    &\int_{0}^{\infty} \PP\del{ \abs{\hmu_{\hr} - \mu_1} < \eps} \difeps \\
    \stackrel{}{=}\,& \fr{144}{N_1}\log\del{\fr{KS}{N_1}}
  \end{align*}
\end{thm-2}

\begin{proof}
  We have
  \begin{align*}
    &\int_{0}^{\infty} \PP\del{ \abs{\hmu_{\hr} - \mu_1} < \eps} \difeps \\
    \stackrel{}{=}\,& \int_{0}^{\infty} \PP\del{ \hmu_{\hr} - \mu_1 < -\eps} \difeps \\
    &+ \int_{0}^{\infty} \PP\del{ \hmu_{\hr} - \mu_1 > \eps} \difeps \\
  \end{align*}
  We use claim Lemma~\ref{lemma:maxlcb_under} for the first term
  \begin{align*}
    &\int_{0}^{\infty} \PP\del{ \hmu_{\hr} - \mu_1 < -\eps} \difeps \le \fr{84}{N_1}\log\del{\fr{KS}{N_1}} 
  \end{align*}
  and use claim Lemma~\ref{lemma:maxlcb_upper} for the second term
  \begin{align*}
    &\int_0^{\infty} \PP\del{\hmu_{\hr} - \mu_1 > \eps} \difeps \le \fr{60}{N_1}\log\del{\fr{KS}{N_1}}
  \end{align*}
  Therefore,
  \begin{align*}
    &\int_{0}^{\infty} \PP\del{ \abs{\hmu_{\hr} - \mu_1} < \eps} \difeps \\
    \stackrel{}{=}\,& \int_{0}^{\infty} \PP\del{ \hmu_{\hr} - \mu_1 < -\eps} \difeps \\
    &+ \int_{0}^{\infty} \PP\del{ \hmu_{\hr} - \mu_1 > \eps} \difeps \\
    \stackrel{}{\le}\,& \fr{84}{N_1}\log\del{\fr{KS}{N_1}} + \fr{60}{N_1}\log\del{\fr{KS}{N_1}} \\
    \stackrel{}{=}\,& \fr{144}{N_1}\log\del{\fr{KS}{N_1}}
  \end{align*}
\end{proof}
% \textbf{Claim 0}: MaxLCB achieves
% \begin{align*}
%   \int_0^{\infty} \PP\del{\abs{\hmu_{\hr} - \mu_1} > \eps} \difeps \le \fr{112}{N_1}\log\del{\fr{K\sum_{j \in [K]}N_j}{N_1}}
% \end{align*}

\begin{lemma}\label{lemma:maxlcb_under}
  MaxLCB achieves
  \begin{align*}
  \int_0^{\infty} \PP\del{\hmu_{\hr} - \mu_1 <- \eps} \difeps \le \fr{84}{N_1}\log\del{\fr{KS}{N_1}}
  \end{align*}
  where $\hmu_{\hr} = \max_{i} \hmu_i - \gam_i$
\end{lemma}

\begin{proof}
  We start off by decomposing the integral
  \begin{align*}
    &\int_0^{\infty} \PP\del{\hmu_{\hr} - \mu_1 < -\eps} \difeps \\
    \stackrel{}{\le}\,& \int_0^{\infty} \PP\del{\hr = 1,\, \hmu_{\hr} - \mu_1 < -\eps} \difeps \\
    &+ \int_0^{\infty} \PP\del{\hr \ne 1,\, \hmu_{\hr} - \mu_1 < -\eps} \difeps
  \end{align*}

  For the first term, we have
  \begin{align*}
    &\PP\del{\hr = 1,\, \hmu_{\hr} - \mu_1 < -\eps} \\
    \stackrel{}{=}\,& \PP\del{\hr = 1,\, \hmu_{1} - \mu_1 < -\eps} \\
    \stackrel{}{\le}\,& \exp\del{-\fr{1}{2}N_1\eps^2}
  \end{align*}
  
  We use Lemma~\ref{lemma401:utility_integral_without_eps} (with $q_1 = 1$ and $z_1 = \fr{1}{2}N_1$) to bound the integral
  \begin{align*}
    & \int_0^{\infty} \PP\del{\hr = 1,\, \hmu_{\hr} - \mu_1 < -\eps} \difeps \\
    \stackrel{}{\le}\,& q_1\fr{1}{z_1} \\
    \stackrel{}{=}\,& \fr{2}{N_1}
  \end{align*}

  For the second term, we have
  \begin{align*}
    &\PP\del{\hr \ne 1,\, \hmu_{\hr} - \mu_1 < -\eps} \\
    \stackrel{}{\le}\,& \PP\del{\hr \ne 1,\, \hmu_{\hr} - \mu_1 < -\eps} \\
    \stackrel{}{\le}\,& \PP\del{\hr \ne 1,\, \hmu_{1} - \gam_1 + \gam_{\hr} - \mu_1 < -\eps} \tagcmt{use def of $\hr$, $\hmu_{\hr} \ge \hmu_{1} - \gam_1 + \gam_{\hr}$} \\
    \stackrel{}{=}\,& \PP\del{\hr \ne 1,\, \hmu_{1} - \mu_1 < -\eps + \gam_1 - \gam_{\hr}} \\
    \stackrel{}{\le}\,& \PP\del{\hr \ne 1,\, \hmu_{1} - \mu_1 < -\eps + \gam_1} \\
    \stackrel{}{\le}\,& \PP\del{\hmu_{1} - \mu_1 < -\eps + \gam_1} \\
    \stackrel{}{\le}\,& \exp\del{-\fr{1}{2}N_1\del{\eps - \gam_1}_+^2}
  \end{align*}

  Let $q_1 = q_2 = 1$, $z_1 = \fr{1}{8}N_1$, and $\eps_0 = 2\gam_1$. We claim that, in the regime of $\eps \ge \eps_0$, we have
  \begin{align*}
    \PP\del{\hr \ne 1,\, \hmu_{\hr} - \mu_1 < -\eps} \le q_1\exp\del{-z_1\eps^2}
  \end{align*}
  and in the regime of $\eps < \eps_0$, we have 
  \begin{align*}
    \PP\del{\hr \ne 1,\, \hmu_{\hr} - \mu_1 < -\eps} \le q_2
  \end{align*}
  The second claim is trivial. We prove the first claim as follows. In the regime of $\eps \ge \eps_0$, we have
  \begin{align*}
    &\PP\del{\hr \ne 1,\, \hmu_{\hr} - \mu_1 < -\eps} \\
    \stackrel{}{\le}\,& \exp\del{-\fr{1}{2}N_1\del{\eps - \gam_1}_+^2} \\
    \stackrel{}{\le}\,& \exp\del{-\fr{1}{2}N_1\del{\fr{\eps}{2}}^2} \tagcmt{use $\eps \ge \eps_0$} \\
    \stackrel{}{=}\,& \exp\del{-\fr{1}{8}N_1\eps^2}
  \end{align*}
  With the above claim, we use Lemma~\ref{lemma401:utility_integral_with_eps} to bound the integral
  \begin{align*}
    &\int_0^{\infty} \PP\del{\hr \ne 1,\, \hmu_{\hr} - \mu_1 < -\eps} \difeps \\
    \stackrel{}{\le}\,& q_2\eps_0^2 + q_1\fr{1}{z_1} \\
    \stackrel{}{=}\,& 4\gam_1^2 + \fr{8}{N_1} \\
    \stackrel{}{=}\,& 4\fr{16}{N_1}\log\del{\fr{KS}{N_1}} + \fr{8}{N_1} \\
    \stackrel{}{=}\,& \fr{64}{N_1}\log\del{\fr{KS}{N_1}} + \fr{8}{N_1}
  \end{align*}

  Combining the two terms above, we have
  \begin{align*}
    &\int_0^{\infty} \PP\del{\hmu_{\hr} - \mu_1 < -\eps} \difeps \\
    \stackrel{}{\le}\,& \int_0^{\infty} \PP\del{\hr = 1,\, \hmu_{\hr} - \mu_1 < -\eps} \difeps \\
    &+ \int_0^{\infty} \PP\del{\hr \ne 1,\, \hmu_{\hr} - \mu_1 < -\eps} \difeps \\
    \stackrel{}{\le}\,& \fr{2}{N_1} + \fr{64}{N_1}\log\del{\fr{KS}{N_1}} + \fr{8}{N_1} \\
    \stackrel{}{=}\,& \fr{2}{N_1} + \fr{32}{N_1}\log\del{\del{\fr{KS}{N_1}}^2} + \fr{8}{N_1} \\
    \stackrel{}{\le}\,& \fr{42}{N_1}\log\del{\del{\fr{KS}{N_1}}^2} \tagcmt{use $1 \le \log(K^2)$ with $K \ge 2$} \\
    \stackrel{}{=}\,& \fr{84}{N_1}\log\del{\fr{KS}{N_1}}
  \end{align*}
  
\end{proof}

\begin{lemma}\label{lemma:maxlcb_upper}
  MaxLCB achieves
  \begin{align*}
  &\int_0^{\infty} \PP\del{\hmu_{\hr} - \mu_1 > \eps} \difeps \le \fr{60}{N_1}\log\del{\fr{KS}{N_1}}.
  \end{align*}
  where $\hmu_{\hr} = \max_{i} \hmu_i - \gam_i$
\end{lemma}


\begin{proof}
  % For brevity, we denote $S := \sum_{j \in [K]}N_j$ in this proof.
  We start off by decomposing the integral
  \begin{align*}
    & \int_0^{\infty} \PP\del{\hmu_{\hr} - \mu_1 > \eps} \difeps  \\
    \stackrel{}{\le}\,& \int_0^{\infty} \PP\del{\hr = 1,\, \hmu_{1} - \mu_1 > \eps} \difeps \\
    &+ \sum_{\substack{i: i \ne 1, \\ \gam_i < 2\gam_1}} \int_0^{\infty} \PP\del{\hr = i,\, \hmu_{i} - \mu_1 > \eps} \difeps + \sum_{\substack{i: i \ne 1, \\ \gam_i > 2\gam_1}} \int_0^{\infty} \PP\del{\hr = i,\, \hmu_{i} - \mu_1 > \eps} \difeps 
  \end{align*}

  We bound the probability and integral of each term separately as follows

  For the first term, we have
  \begin{align*}
    &\PP\del{\hr = 1,\, \hmu_{\hr} - \mu_1 > \eps} \\
    \stackrel{}{=}\,& \PP\del{\hr = 1,\, \hmu_{1} - \mu_1 > \eps} \\
    \stackrel{}{\le}\,& \exp\del{-\fr{1}{2}N_1\eps^2}
  \end{align*}

  We use Lemma~\ref{lemma401:utility_integral_without_eps} (with $q_1 = 1$ and $z_1 = \fr{1}{2}N_1$) to bound the integral
  \begin{align*}
    & \int_0^{\infty} \PP\del{\hr = 1,\, \hmu_{\hr} - \mu_1 > \eps} \difeps \le \fr{2}{N_1}
  \end{align*}
  
  For the second term, for any $i \ne 1,\, \gam_i < 2\gam_1$ we have
  \begin{align*}
    &\sum_{\substack{i: i \ne 1, \\ \gam_i < 2\gam_1}} \PP\del{\hr = i,\, \hmu_{i} - \mu_1 > \eps} \\
    \stackrel{}{=}\,& \sum_{\substack{i: i \ne 1, \\ \gam_i < 2\gam_1}} \PP\del{\hr = i,\, \hmu_{i} - \mu_i > \eps + \Delta_i} \\
    \stackrel{}{\le}\,& \sum_{\substack{i: i \ne 1, \\ \gam_i < 2\gam_1}} \exp\del{-\fr{1}{2}N_i\del{\eps + \Delta_i}^2} \\
    \stackrel{}{\le}\,& \sum_{\substack{i: i \ne 1, \\ \gam_i < 2\gam_1}} \exp\del{-\fr{1}{2}N_i\eps^2} \\
    \stackrel{}{\le}\,& \sum_{\substack{i: i \ne 1, \\ \gam_i < 2\gam_1}} \exp\del{-\fr{1}{2}\min_{\substack{i: i \ne 1, \\ \gam_i < 2\gam_1}}N_i\eps^2} \\
    \stackrel{}{\le}\,& K\exp\del{-\fr{1}{2}\min_{\substack{i: i \ne 1, \\ \gam_i < 2\gam_1}}N_i\eps^2}
  \end{align*}

  For this term, let $q_1 = q_2 = 1$, $z_1 = \displaystyle \fr{1}{4}\min_{\substack{i: i \ne 1, \\ \gam_i < 2\gam_1}}N_i$, and $\eps_0 = \displaystyle \sqrt{\max_{\substack{i: i \ne 1, \\ \gam_i < 2\gam_1}}\fr{4\log(K)}{N_i}}$. We claim that, in the regime of $\eps \ge \eps_0$, we have
  \begin{align*}
    \sum_{\substack{i: i \ne 1, \\ \gam_i < 2\gam_1}} \PP\del{\hr = i,\, \hmu_{i} - \mu_1 > \eps} \le \exp\del{-z_1\eps^2} 
  \end{align*}
  and, in the regime of $\eps < \eps_0$, we have
  \begin{align*}
    \sum_{\substack{i: i \ne 1, \\ \gam_i < 2\gam_1}} \PP\del{\hr = i,\, \hmu_{i} - \mu_1 > \eps} \le q_2
  \end{align*}
  The second claim is trivial. We prove the first claim as follows. In the regime of $\eps \ge \eps_0$, we have
  \begin{align*}
    &\sum_{\substack{i: i \ne 1, \\ \gam_i < 2\gam_1}} \PP\del{\hr = i,\, \hmu_{i} - \mu_1 > \eps} \\
    \stackrel{}{\le}\,& K\exp\del{-\fr{1}{2}\min_{\substack{i: i \ne 1, \\ \gam_i < 2\gam_1}}N_i\eps^2} \\
    \stackrel{}{\le}\,& \exp\del{-\fr{1}{2}\min_{\substack{i: i \ne 1, \\ \gam_i < 2\gam_1}}N_i\eps^2 + \log(K)} \\
    \stackrel{}{\le}\,& \exp\del{-\fr{1}{4}\min_{\substack{i: i \ne 1, \\ \gam_i < 2\gam_1}}N_i\eps^2} \tagcmt{use $\eps \ge \eps_0$}
  \end{align*}

  With the above claim, we use Lemma~\ref{lemma401:utility_integral_with_eps} to bound the integral
  \begin{align*}
    &\int_{0}^{\infty} \sum_{\substack{i: i \ne 1, \\ \gam_i < 2\gam_1}} \PP\del{\hr = i,\, \hmu_{i} - \mu_1 > \eps} \difeps \\
    \stackrel{}{\le}\,& q_2\eps_0^2 + q_1\fr{1}{z_1} \\
    \stackrel{}{=}\,& \max_{\substack{i: i \ne 1, \\ \gam_i < 2\gam_1}}\fr{4\log(K)}{N_i} + \max_{\substack{i: i \ne 1, \\ \gam_i < 2\gam_1}} \fr{4}{N_i} \\
    \stackrel{}{=}\,& \max_{\substack{i: i \ne 1, \\ \gam_i < 2\gam_1}}\fr{2\log(K^2)}{N_i} + \max_{\substack{i: i \ne 1, \\ \gam_i < 2\gam_1}} \fr{4}{N_i} \\
    \stackrel{}{\le}\,& \max_{\substack{i: i \ne 1, \\ \gam_i < 2\gam_1}}\fr{6\log(K^2)}{N_i} \tagcmt{use $1 \le \log(K^2)$ with $K \ge 2$} \\
    \stackrel{}{=}\,& \max_{\substack{i: i \ne 1, \\ \gam_i < 2\gam_1}}\fr{12\log(K)}{N_i}
  \end{align*}
  
  Lemma~\ref{lemma:maxlcb_101} states that for any $i \ne 1$ the condition $\gam_i < 2\gam_1$ implies that $N_i > \fr{N_1}{4} \fr{\log\del{K}}{\log\del{\fr{KS}{N_1}}}$. Therefore,
  \begin{align*}
    &\max_{\substack{i: i \ne 1, \\ \gam_i < 2\gam_1}}\fr{12\log(K)}{N_i} \\
    \stackrel{}{\le}\,& \max_{\substack{i: i \ne 1, \\ \gam_i < 2\gam_1}}\fr{12\log(K)}{N_1}\fr{4\log\del{\fr{KS}{N_1}}}{\log\del{K}} \\
    \stackrel{}{=}\,& \fr{48}{N_1}\log\del{\fr{KS}{N_1}}
  \end{align*}

  From this point, let $i$ be an arm such that $i \ne 1,\, \gam_i > 2\gam_1$.
  For the third term, we have
  \begin{align*}
    &\PP\del{\hr = i,\, \hmu_{i} - \mu_1 > \eps} \\
    \stackrel{}{=}\,& \PP\del{\hr = i,\, \hmu_{i} - \mu_i > \eps + \Delta_i} \\
    \stackrel{}{\le}\,& \exp\del{-\fr{1}{2}N_i\del{\eps + \Delta_i}^2} \\
    \stackrel{}{\le}\,& \exp\del{-\fr{1}{2}N_i\eps^2}
  \end{align*}

  In addition, we have
  \begin{align*}
    &\PP\del{\hr = i} \\
    \stackrel{}{\le}\,& \PP\del{\hr = i,\, \hmu_i - \gam_i > \hmu_1 - \gam_1} \\
    \stackrel{}{=}\,& \PP\del{\hr = i,\, \hmu_i - \mu_i - \hmu_1 + \mu_1 > \gam_i - \gam_1 + \Delta_i} \\
    \stackrel{}{\le}\,& \PP\del{\hr = i,\, \hmu_i - \mu_i - \hmu_1 + \mu_1 > \fr{1}{2}\gam_i + \Delta_i} \tagcmt{use $\gam_i > 2\gam_1$} \\
    \stackrel{}{\le}\,& \exp\del{-\fr{1}{2}\fr{1}{\del{\fr{1}{N_i} + \fr{1}{N_1}}}\del{\fr{1}{2}\gam_i + \Delta_i}^2} \\
    \stackrel{}{\le}\,& \exp\del{-\fr{1}{8}\fr{1}{\del{\fr{1}{N_i} + \fr{1}{N_1}}}\gam_1^2} 
  \end{align*}
  
  Lemma~\ref{lemma:maxlcb_102} states that for any $i \ne 1$ the condition $\gam_i > 2\gam_1$ implies that $N_i < N_1$. Therefore,
  \begin{align*}
    &\exp\del{-\fr{1}{8}\fr{1}{\del{\fr{1}{N_i} + \fr{1}{N_1}}}\gam_i^2} \\
    \stackrel{}{\le}\,& \exp\del{-\fr{1}{8}\fr{1}{\del{\fr{1}{N_i} + \fr{1}{N_i}}}\gam_i^2} \tagcmt{use $N_i < N_1$} \\
    \stackrel{}{=}\,& \exp\del{-\fr{1}{16}N_i\gam_i^2} \\
    \stackrel{}{=}\,& \exp\del{-\fr{1}{16}N_i\fr{16}{N_i}\log\del{\del{\fr{KS}{N_i}}^2}} \\
    \stackrel{}{=}\,& \del{\fr{N_i}{KS}}^2
  \end{align*}

  % ==
  
  % Therefore, for any $i \ne 1,\, \gam_i > 2\gam_1$, we have
  % \begin{align*}
  %   & \PP\del{\hr = i,\, \hmu_{i} - \mu_1 > \eps} \\
  %   \stackrel{}{\le}\,& \fr{N_i}{K\sum_{j \in [K]}N_j} \wedge \exp\del{-\fr{1}{2}N_i\eps^2} 
  % \end{align*}
  % For any $i \ne 1,\, \gam_i > 2\gam_1$, we use Lemma~\ref{lemma403:utility_integral_with_eps} (with $q = \fr{N_i}{K\sum_{j \in [K]}N_j}$, $v = 0$, and $z_1 = \fr{1}{4}N_i$) to bound the integral
  % \begin{align*}
  %   &\int_{0}^{\infty} \PP\del{\hr = i,\, \hmu_{i} - \mu_1 > \eps} \difeps \\
  %   \stackrel{}{\le}\,& \fr{2}{N_i}\fr{N_i}{K\sum_{j \in [K]}N_j}\log\del{\fr{K\sum_{j \in [K]}N_j}{N_i}} + \fr{2}{N_i}\fr{N_i}{K\sum_{j \in [K]}N_j} 
  % \end{align*}
  % This proof is not good since the denominator of the log contains $N_i$ not $N_1$. We use below proof.
  
  % ==

  Combining two inequalities above, we have
  \begin{align*}
    & \PP\del{\hr = i,\, \hmu_{i} - \mu_1 > \eps} \\
    \stackrel{}{\le}\,& \del{\fr{N_i}{KS}}^2 \wedge \exp\del{-\fr{1}{2}N_i\eps^2} \\
    \stackrel{}{\le}\,& \sqrt{\del{\fr{N_i}{KS}}^2\exp\del{-\fr{1}{2}N_i\eps^2}} \\
    \stackrel{}{=}\,& \fr{N_i}{KS} \exp\del{-\fr{1}{4}N_i\eps^2} 
  \end{align*}

  We use Lemma~\ref{lemma401:utility_integral_without_eps} (with $q_1 = \fr{N_i}{KS}$ and $z_1 = \fr{1}{4}N_i$) to bound the integral
  \begin{align*}
    &\int_{0}^{\infty} \PP\del{\hr = i,\, \hmu_{i} - \mu_1 > \eps} \difeps \\
    \stackrel{}{\le}\,& q\fr{1}{z_1} \\
    \stackrel{}{\le}\,& \fr{N_i}{KS} \fr{4}{N_i} \\
    \stackrel{}{\le}\,& \fr{4}{KS}
  \end{align*}
  
  Therefore, for the third term, we obtain the integral
  \begin{align*}
    &\sum_{\substack{i: i \ne 1, \\ \gam_i > 2\gam_1}} \int_{0}^{\infty} \PP\del{\hr = i,\, \hmu_{i} - \mu_1 > \eps} \difeps \\
    \stackrel{}{\le}\,& \sum_{\substack{i: i \ne 1, \\ \gam_i > 2\gam_1}} \fr{4}{K\sum_{j \in [K]}N_j} \\
    \stackrel{}{\le}\,& K\fr{4}{KS} \\
    \stackrel{}{=}\,& \fr{4}{S}
    % \stackrel{}{=}\,& \fr{4}{\sum_{j \in [K]}N_j} \tagcmt{use $S = \$}
  \end{align*}

  Combining all terms together, we have
  \begin{align*}
    & \int_0^{\infty} \PP\del{\hmu_{\hr} - \mu_1 > \eps} \difeps  \\
    \stackrel{}{\le}\,& \int_0^{\infty} \PP\del{\hr = 1,\, \hmu_{1} - \mu_1 > \eps} \difeps \\
    &+ \sum_{\substack{i: i \ne 1, \\ \gam_i < 2\gam_1}} \int_0^{\infty} \PP\del{\hr = i,\, \hmu_{i} - \mu_1 > \eps} \difeps + \sum_{\substack{i: i \ne 1, \\ \gam_i > 2\gam_1}} \int_0^{\infty} \PP\del{\hr \ne i,\, \hmu_{i} - \mu_1 > \eps} \difeps \\
    \stackrel{}{\le}\,& \fr{2}{N_1} + \fr{48}{N_1}\log\del{\fr{KS}{N_1}} + \fr{4}{S} \\
    \stackrel{}{=}\,& \fr{2}{N_1} + \fr{48}{N_1}\log\del{\fr{KS}{N_1}} + \fr{4}{\sum_{j \in [K]}N_j} \tagcmt{use $S = \sum_{j \in [K]}N_j$} \\
    \stackrel{}{=}\,& \fr{2}{N_1} + \fr{24}{N_1}\log\del{\del{\fr{KS}{N_1}}^2} + \fr{4}{\sum_{j \in [K]}N_j} \\
    \stackrel{}{\le}\,& \fr{30}{N_1}\log\del{\del{\fr{KS}{N_1}}^2} \tagcmt{use $1 \le \log(K^2)$ with $K \ge 2$} \\
    \stackrel{}{=}\,& \fr{60}{N_1}\log\del{\fr{KS}{N_1}} 
  \end{align*}
  

\end{proof}


\begin{lemma}\label{lemma:maxlcb_101}
  Let $\gam_i = \sqrt{\fr{a}{N_i}\log\del{\del{\fr{KS}{N_i}}^{s}}}$ where $S \ge N_i$ and $s \ge 1$. For any $i \ne 1$, the condition $\gam_i < b\gam_1$ implies that $N_i > \fr{N_1}{b^2} \fr{\log\del{K}}{\log\del{\fr{KS}{N_1}}}$.
\end{lemma}

\begin{proof}
  % By def, we have $\gam_i = \sqrt{\fr{a}{N_i}\log\del{\fr{K\sum_{j \in [K]}N_j}{N_i}}}$.
  
  % For brevity, we denote $S = \sum_{j \in [K]}N_j$ in this proof.
  
  We have
  \begin{align*}
    &\gam_i < b\gam_1 \\
    \stackrel{}{\Leftrightarrow}\,& \fr{a}{N_i}\log\del{\del{\fr{KS}{N_i}}^{s}} < b^2\fr{a}{N_1}\log\del{\del{\fr{KS}{N_1}}^{s}} \\
    \stackrel{}{\Leftrightarrow}\,& \fr{1}{N_i}\log\del{\fr{KS}{N_i}} < \fr{b^2}{N_1}\log\del{\fr{KS}{N_1}} \\
    \stackrel{}{\Leftrightarrow}\,& N_i > \fr{N_1}{b^2} \fr{\log\del{\fr{KS}{N_i}}}{\log\del{\fr{KS}{N_1}}} \\
    \stackrel{}{\Rightarrow}\,& N_i > \fr{N_1}{b^2} \fr{\log\del{K}}{\log\del{\fr{KS}{N_1}}} \tagcmt{use $N_i \le S$}
  \end{align*}
\end{proof}

\begin{lemma}\label{lemma:maxlcb_102}
  Let $\gam_i = \sqrt{\fr{a}{N_i}\log\del{\del{\fr{KS}{N_i}}^{s}}}$ where $S \ge N_i$ and $s \ge 1$. For $b \ge 2$, for any $i \ne 1$, the condition $\gam_i > b\gam_1$ implies that $N_i < N_1$.
\end{lemma}

\begin{proof}
  % By def, we have $\gam_i = \sqrt{\fr{16}{N_i}\log\del{\fr{K\sum_{j \in [K]}N_j}{N_i}}}$.
  
  % For brevity, we denote $S = \sum_{j \in [K]}N_j$ in this proof.
  
  We have
  \begin{align*}
    &\gam_i > b\gam_1 \\
    \stackrel{}{\Leftrightarrow}\,& \fr{a}{N_i}\log\del{\del{\fr{KS}{N_i}}^s} > b^2\fr{a}{N_1}\log\del{\del{\fr{KS}{N_1}}^s} \\
    \stackrel{}{\Leftrightarrow}\,& \fr{1}{N_i}\log\del{\fr{KS}{N_i}} > \fr{b^2}{N_1}\log\del{\fr{KS}{N_1}} \\
    \stackrel{}{\Leftrightarrow}\,& N_i < \fr{N_1}{b^2} \fr{\log\del{\fr{KS}{N_i}}}{\log\del{\fr{KS}{N_1}}} \\
  \end{align*}

  For any $c \ge 0$, there are two cases: (1) $N_i \ge c$ and (2) $N_i < c$.

  The case $N_i \ge c$ implies that
  \begin{align*}
    N_i < \fr{N_1}{b^2} \fr{\log\del{\fr{KS}{N_i}}}{\log\del{\fr{KS}{N_1}}} < \fr{N_1}{b^2} \fr{\log\del{\fr{KS}{c}}}{\log\del{\fr{KS}{N_1}}}
  \end{align*}

  Therefore, for any $c \ge 0$, we have
  \begin{align*}
    N_i < \fr{N_1}{b^2} \fr{\log\del{\fr{KS}{c}}}{\log\del{\fr{KS}{N_1}}} \vee c
  \end{align*}

  Choosing $c = N_1$, we have
  \begin{align*}
    N_i &< \fr{N_1}{b^2} \fr{\log\del{\fr{KS}{N_1}}}{\log\del{\fr{KS}{N_1}}} \vee N_1 < \fr{N_1}{b^2} \vee N_1 \le N_1 
  \end{align*}
  
\end{proof}




\section{Theorems for the empirical maximum estimator}

\begin{theorem}\label{thm:empmax_lower_bound_generic}
  For Gaussian rewards, the empirical maximum estimator's MSE is lower bounded by
  \begin{align*}
    \MSE = \tilcOmega \del{\sum_{i \in [K]}\frac{1}{N_i}}
  \end{align*}
\end{theorem}
The proof is in Appendix ~\ref{thm_proof:empmax_lower_bound_generic}

\section{Proof of Theorem ~\ref{thm:empmax_lower_bound_generic}}
\label{thm_proof:empmax_lower_bound_generic}

\newtheorem*{thm-3}{Theorem ~\ref{thm:empmax_lower_bound_generic}}
\begin{thm-3}
  The empirical maximum estimator's MSE is lower bounded by
  \begin{align*}
    \MSE = \tilcOmega \del{\sum_{i \in [K]}\frac{1}{N_i}}
  \end{align*}
\end{thm-3}

\begin{proof}
  We denote $\hmume$ to be output of the maximum empirical estimator and denote $\ha = \argmax_{i \in [K]} \hmu_i$ to be the arm with the highest empirical mean ($\ha$ is a random variable). That means $\hmume = \hmu_{\ha}$.
  
  We decompose the MSE as follows
\begin{align*}
  &\EE\sbr{\del{\hmume - \mu_1}^2} \\
  \stackrel{}{=}\,&\int_{0}^{\infty} \PP\del{\del{\hmume - \mu_1}^2 > \eps^2 } \dif \eps \\
  \stackrel{}{=}\,&\int_{0}^{\infty} \PP\del{\abs{\hmume - \mu_1} > \eps } 2\eps \dif \eps \tagcmt{change of variable} \\
  \stackrel{}{=}\,&\int_{0}^{\infty} \PP\del{\abs{\hmu_{\ha} - \mu_1} > \eps } 2\eps \dif \eps \\
  \stackrel{}{=}\,&\int_{0}^{\infty} \del{\PP\del{\hmu_{\ha} - \mu_1 > \eps } + \PP\del{\hmu_{\ha} - \mu_1 < -\eps } }2\eps \dif \eps \\
  \stackrel{}{\ge}\,&\int_{0}^{\infty} \PP\del{\hmu_{\ha} - \mu_1 > \eps } 2\eps \dif \eps \\
  \stackrel{}{=}\,& \int_{0}^{\infty} \PP\del{\ha = 1,\, \muhat_i - \mu_1 > \eps} 2\eps \dif \eps + \sum_{i \in [2,K]} \int_{0}^{\infty} \PP\del{\ha = i,\, \muhat_i - \mu_1 > \eps} 2\eps \dif \eps.
\end{align*}

% We bound the probability terms inside the integral.
We bound the first probability as follows,
\begin{align*}
  &\PP\del{\ha = 1,\, \muhat_1 - \mu_1 > \eps} \\
  \stackrel{}{=}\,&\PP\del{\muhat_1 - \muhat_2 \ge 0,\, \muhat_1 - \mu_1 > \eps} \tagcmt{by def $\ha = \argmax_i \hmu_i$} \\
  \stackrel{}{=}\,&\PP\del{\muhat_1 - \mu_1 - \muhat_2 + \mu_2 \ge -\Delta_2,\, \muhat_1 - \mu_1 > \eps}.
\end{align*}

Let $X_1 = \hmu_1 - \mu_1$ and $X_2 = \muhat_2 - \mu_2$, we further have
\begin{align*}
  &\PP\del{X_1 - X_2 \ge -\Delta_2,\, X_1 > \eps} \\
  \stackrel{}{=}\,& \int_{x_1,x_2} \idt{x_1 - x_2 \ge -\Delta_2,\, x_1 > \eps}\dif \PP(x_2) \dif \PP(x_1) \\
  \stackrel{}{=}\,& \int_{x_1=\eps}^{\infty} \int_{x_2=-\infty}^{x_1 + \Delta_2} 1 \dif \PP(x_1)\dif \PP(x_2) \\
  \stackrel{}{\ge}\,& \int_{x_1=\eps}^{\infty} \int_{x_2=-\infty}^{0} 1 \dif \PP(x_1)\dif \PP(x_2) \tagcmt{since $x_1 + \Delta_2 \ge \eps + \Delta_2 \ge 0$} \\
  \stackrel{}{=}\,&\int_{x_1=\eps}^{\infty} \frac{1}{2} \dif \PP(x_2) \tagcmt{$x_1$ is of Gaussian distribution with zero mean} \\
  \stackrel{}{=}\,& \frac{1}{2}\PP\del{X_1 \ge \eps} \\
  \stackrel{}{=}\,& \frac{1}{2}\PP\del{\hmu_1 -  \mu_1 \ge \eps} \\
  \stackrel{}{\ge}\,& \frac{1}{2}\frac{1}{4\sqrt{\pi}}\exp\del{-\frac{7N_1\eps^2}{2}}  \tagcmt{use Lemma ~\ref{xlemma:anti_concentration_inequality} with variance $\sigma^2 = \fr{1}{N_1}$} \\
  \stackrel{}{=}\,& \frac{1}{8\sqrt{\pi}}\exp\del{-\frac{7N_{1}\eps^2}{2}}.
\end{align*}

Next, we bound the second probability term, $\forall i \in [2,K]$,
\begin{align*}
  &\PP\del{\ha = i,\, \muhat_{i} - \mu_1 > \eps} \\
  \stackrel{}{=}\,& \PP\del{\muhat_{i} - \muhat_1 \ge 0,\, \muhat_{i} - \mu_{1} > \eps } \tagcmt{by def $\ha = \argmax_i \hmu_i$} \\
  \stackrel{}{=}\,& \PP\del{\muhat_{i} - \mu_{i} - \muhat_1 + \mu_1 \ge \Delta_{i},\, \muhat_{i} - \mu_{i} > \eps + \Delta_{i}}. 
\end{align*}

Let $X_i = \hmu_i - \mu_i$ and $X_1 = \muhat_1 - \mu_1$, we further have
\begin{align*}
  &\PP\del{X_{i} - X_1 \ge \Delta_{i},\, X_{i} > \eps + \Delta_{i}} \\
  \stackrel{}{=}\,& \int_{x_1,x_{i}} \idt{x_{i} - x_1 \ge \Delta_{i},\, x_{i} > \eps + \Delta_{i}}\dif \PP(x_1)\dif \PP(x_{i}) \\
  \stackrel{}{=}\,& \int_{x_{i}=\eps+\Delta_{i}}^{\infty} \int_{x_1=-\infty}^{x_{i} - \Delta_{i}} 1 \dif \PP(x_1)\dif \PP(x_{i}) \\
  \stackrel{}{\ge}\,& \int_{x_{i}=\eps+\Delta_{i}}^{\infty} \int_{x_1=-\infty}^{0} 1 \dif \PP(x_1)\dif \PP(x_{i}) \tagcmt{since $x_i - \Delta_i \ge \eps + \Delta_i - \Delta_i \ge 0$} \\
  \stackrel{}{=}\,& \int_{x_{i}=\eps+\Delta_{i}}^{\infty} \frac{1}{2} \dif \PP(x_{i}) \tagcmt{$x_i$ is of Gaussian distribution with zero mean} \\
  \stackrel{}{=}\,& \frac{1}{2}\PP\del{X_{i} > \eps + \Delta_{i}} \\
  \stackrel{}{\ge}\,& \frac{1}{2}\PP\del{\hmu_{i} - \mu_i > \eps} \\
  \stackrel{}{\ge}\,& \frac{1}{2}\frac{1}{4\sqrt{\pi}}\exp\del{-\frac{7N_{i}\eps^2}{2}} \tagcmt{use Lemma ~\ref{xlemma:anti_concentration_inequality} with variance $\sigma^2 = \fr{1}{N_i}$} \\
  \stackrel{}{=}\,& \frac{1}{8\sqrt{\pi}}\exp\del{-\frac{7N_{i}\eps^2}{2}}.
\end{align*}

From the first and second probability bounds, we have $\forall i \in [K], \PP\del{\ha = i,\, \muhat_i - \mu_1 > \eps} \ge \frac{1}{8\sqrt{\pi}}\exp\del{-\frac{7N_{i}\eps^2}{2}}$. Therefore,
\begin{align*}
  &\int_{0}^{\infty} \PP\del{\ha = 1,\, \muhat_i - \mu_1 > \eps} 2\eps \dif \eps + \sum_{i \in [2,K]} \int_{0}^{\infty} \PP\del{\ha = i,\, \muhat_i - \mu_1 > \eps} 2\eps \dif \eps \\
  \stackrel{}{\ge}\,&  \sum_{i \in [K]}  \int_{0}^{\infty} \frac{1}{8\sqrt{\pi}} \exp\del{-\frac{7N_i\eps^2}{2}} 2\eps \dif \eps \\
  \stackrel{}{=}\,& \frac{1}{8\sqrt{\pi}} \sum_{i \in [K]} \del{- \frac{2}{7N_i}\exp\del{-\frac{7N_i\eps^2}{2}}}\Big|_{0}^{\infty} \\
  \stackrel{}{=}\,& \frac{1}{8\sqrt{\pi}} \sum_{i \in [K]} \frac{1}{N_i}.
\end{align*}
\end{proof}
